# Supplementary material for: Polaronic-Quasiparticle Picture for Generation Dynamics of Coherent Phonons in Semiconductors: Transient and Non-Linear Fano Resonance
Source: arXiv:1510.00263 source file (2016-04-15)
Supplement: Supplementary file 1 [file SupplementalMaterial_final.pdf]

Supplemental Material is composed of the following appendix-sections.


**A:** Parameters of Materials and Lasers Employed in the Present Study

**B:** Derivation of Eq. (12): A Factorization Approximation

**C:** Solutions of Eigenvalue Equations of Eqs. (22) and (23)

**D:** Closed Analytic Forms of $F^{\dagger}_{\boldsymbol{q}\beta}$ and $F_{\boldsymbol{q}\beta}$ Derived by Solving Eq. (67)

- **D1:** Introduction of Operators of $F^{0\dagger}_{\boldsymbol{q}\beta}$ and $F^{0}_{\boldsymbol{q}\beta}$
- **D2:** Approximate Solutions of $F^{\dagger}_{\boldsymbol{q}\beta}$ and $F_{\boldsymbol{q}\beta}$
- **D3:** Bosonization Scheme and its Approximate Validity
- **D4:** Solutions of the Fano Problem given by Adiabatic Coupled-Equations of Eq. (D3)

**E:** Detail of Deriving an Expression of Total Retarded Longitudinal-Susceptibility $\chi^{(t)}_{\boldsymbol{q}}(t,t')$

- **E1:** Derivation of a Retarded Susceptibility due to Electron-Induced Interaction $\chi_{\boldsymbol{q}}(t,t')$
- **E2:** Derivation of a Retarded Susceptibility due to LO-Phonon-Induced Interaction $\chi'_{\boldsymbol{q}}(t,t')$
- **E3:** Expression of $\chi^{(t)}_{\boldsymbol{q}}(t'+\tau,t')$
- **E4:** Calculation of $\tilde{R}_{\boldsymbol{q}\gamma\gamma'}(t,t_D)$ of Eq. (E10)

**F:** Derivation of Eq. (114): Shore's Spectral Profile

**G:** Derivation of Eq. (126): Phonon Displacement Function $Q_{\boldsymbol{q}}(t)$

**H:** Properties of Dimensionless Function $\mathcal{D}_{\boldsymbol{q}\alpha_p}(t,t_D)$


## APPENDIX A: PARAMETERS OF MATERIALS AND LASERS EMPLOYED IN THE PRESENT STUDY

TABLE A-1: Materials parameters of undoped Si and undoped GaAs employed in the present study, where $m_c$ and $m_v$ represent effective masses of conduction- and valence-electrons at Γ point, respectively, $\epsilon_0$ and $\epsilon_\infty$ represent a static dielectric constant and a dielectric constant in the high-frequency limit, respectively, $g^D_{c\boldsymbol{q}}$ and $g^D_{v\boldsymbol{q}}$ represent conduction- and valence-band electron-LO-phonon coupling constants of deformation-potential interaction, respectively [1]. $\omega^{(LO)}_{\boldsymbol{q}}$ represents LO-phonon frequency at Γ point, $N_s$ represents the total number of sites included in calculations, and $d$ represents a lattice constant. Here, the magnitude of momentum $\boldsymbol{q}$ is assumed to be quite small; $|\boldsymbol{q}| = 0.015$. Atomic units are used herein, unless otherwise stated.

| Parameters | undoped Si | undoped GaAs |
|---|---|---|
| $m_c$ | 0.158 | 0.067 |
| $m_v$ | -0.523 | -0.45 |
| $\epsilon_0$ | 11.9 | 11.53 |
| $\epsilon_\infty$ | 11.9 | 10.10 |
| $g^D_{c\boldsymbol{q}}$ | 0 | 0 |
| $g^D_{v\boldsymbol{q}}$ | 0.195 | 0.101 |
| $\omega^{(LO)}_{\boldsymbol{q}}$ | 63 meV | 35 meV |
| $N_s$ | $70^3(=3.43\times10^5)$ | $64^3(=2.62\times10^5)$ |
| $d$ | 10.5 | 10.5 |

TABLE A-2: Parameters of a square-shaped pulse laser employed in the present study, where $\Delta\omega$ represents detuning with reference to energy-band gap, $\tau_L$ represents temporal width, $A_L$ represents pulse area, and $N^0_{ex}$ represents the maximum excited-electron density.

| Parameters | undoped Si | undoped GaAs |
|---|---|---|
| $\Delta\omega$ | 82 meV | 73 meV |
| $\tau_L$ | 15 fs | 15 fs |
| $A_L$ | $0.12\pi$ | $0.20\pi$ |
| $N^0_{ex}$ | $6.31\times10^{17}/\text{cm}^3$ | $5.30\times10^{17}/\text{cm}^3$ |


[1] More accurate values of $g^D_{v\boldsymbol{q}}$ for undoped Si and GaAs are given by, for instance, W. Pötz and P. Vogl, Phys. Rev. B **24**, 2025 (1981).

## APPENDIX B: DERIVATION OF EQ. (12): A FACTORIZATION APPROXIMATION

For the purpose of deriving Eq. (12), the following commutation relation:

$$
\begin{aligned}
&[A^\dagger_{\boldsymbol{q}_1}(\boldsymbol{k}_1 b_1 b'_1), A^\dagger_{\boldsymbol{q}_2}(\boldsymbol{k}_2 b_2 b'_2)] \\
&= \left[a^\dagger_{b_1,\boldsymbol{k}_1+\boldsymbol{q}_1} a_{b'_1\boldsymbol{k}_1}, a^\dagger_{b_2,\boldsymbol{k}_2+\boldsymbol{q}_2} a_{b'_2\boldsymbol{k}_2}\right] \\
= \; & a^\dagger_{b_1,\boldsymbol{k}_1+\boldsymbol{q}_1} a_{b'_2\boldsymbol{k}_2}\delta_{b'_1 b_2}\delta_{\boldsymbol{k}_1,\boldsymbol{k}_2+\boldsymbol{q}_2} \\
& -a^\dagger_{b_2,\boldsymbol{k}_2+\boldsymbol{q}_2} a_{b'_1\boldsymbol{k}_1}\delta_{b_1 b'_2}\delta_{\boldsymbol{k}_1+\boldsymbol{q}_1,\boldsymbol{k}_2}.
\end{aligned} \tag{B1}
$$

is applied to $[\hat{\mathcal{H}}_e(t), A^\dagger_{\boldsymbol{q}}(\boldsymbol{k}bb')]$ in a repeated manner. First, the commutator of $[\hat{H}_e, A^\dagger_{\boldsymbol{q}}(\boldsymbol{k}bb')]$ is provided by

$$
\begin{aligned}
&\left[\hat{H}_e, A^\dagger_{\boldsymbol{q}}(\boldsymbol{k}bb')\right] \\
&= (\varepsilon'_{b\boldsymbol{k}+\boldsymbol{q}} - \varepsilon'_{b'\boldsymbol{k}})A^\dagger_{\boldsymbol{q}}(\boldsymbol{k}bb') \\
&+\frac{1}{2}\sum_{\boldsymbol{q}'(\neq \boldsymbol{0})\boldsymbol{k}'\tilde{b}} V^{(C)}_{\boldsymbol{q}'}\Big\{A^\dagger_{\boldsymbol{q}'}(\boldsymbol{k}'\tilde{b}\tilde{b})A^\dagger_{\boldsymbol{q}-\boldsymbol{q}'}(\boldsymbol{k}bb') \\
&-A^\dagger_{\boldsymbol{q}'}(\boldsymbol{k}'\tilde{b}\tilde{b})A^\dagger_{\boldsymbol{q}-\boldsymbol{q}'}(\boldsymbol{k}+\boldsymbol{q}'bb') + A^\dagger_{\boldsymbol{q}+\boldsymbol{q}'}(\boldsymbol{k}bb')A^\dagger_{-\boldsymbol{q}'}(\boldsymbol{k}'\tilde{b}\tilde{b}) \\
&- A^\dagger_{\boldsymbol{q}+\boldsymbol{q}'}(\boldsymbol{k}-\boldsymbol{q}'bb')A^\dagger_{-\boldsymbol{q}'}(\boldsymbol{k}'\tilde{b}\tilde{b})\Big\}.
\end{aligned} \tag{B2}
$$

By use of a factorization approximation, the four-operator term, $A^\dagger_{\boldsymbol{q}'}(\boldsymbol{k}'\tilde{b}\tilde{b})A^\dagger_{\boldsymbol{q}-\boldsymbol{q}'}(\boldsymbol{k}bb')$, which appears as the first term in the curl brackets of the right-hand side of Eq. (B2), is further reduced to

$$
\begin{aligned}
&A^\dagger_{\boldsymbol{q}'}(\boldsymbol{k}'\tilde{b}\tilde{b})A^\dagger_{\boldsymbol{q}-\boldsymbol{q}'}(\boldsymbol{k}bb') \\
&\approx \langle a^\dagger_{\tilde{b},\boldsymbol{k}'+\boldsymbol{q}'} a_{\tilde{b}\boldsymbol{k}'}\rangle A^\dagger_{\boldsymbol{q}-\boldsymbol{q}'}(\boldsymbol{k}bb') + A^\dagger_{\boldsymbol{q}'}(\boldsymbol{k}'\tilde{b}\tilde{b})\langle a^\dagger_{b,\boldsymbol{k}+\boldsymbol{q}-\boldsymbol{q}'} a_{b'\boldsymbol{k}}\rangle \\
&-\langle a^\dagger_{\tilde{b},\boldsymbol{k}'+\boldsymbol{q}'} a_{b'\boldsymbol{k}}\rangle a^\dagger_{b,\boldsymbol{k}+\boldsymbol{q}-\boldsymbol{q}'} a_{b'\boldsymbol{k}'} \\
&-a^\dagger_{\tilde{b},\boldsymbol{k}'+\boldsymbol{q}'} a_{b'\boldsymbol{k}}\langle a^\dagger_{b,\boldsymbol{k}+\boldsymbol{q}-\boldsymbol{q}'} a_{b'\boldsymbol{k}'}\rangle \\
&\approx \rho_{\tilde{b}\tilde{b}\boldsymbol{k}'}\delta_{\boldsymbol{q}'\boldsymbol{0}}A^\dagger_{\boldsymbol{q}}(\boldsymbol{k}bb') + A^\dagger_{\boldsymbol{q}}(\boldsymbol{k}'\tilde{b}\tilde{b})\rho_{bb'\boldsymbol{k}}\delta_{\boldsymbol{q}'\boldsymbol{q}} \\
&-\rho_{\tilde{b}b'\boldsymbol{k}}\delta_{\boldsymbol{k}'+\boldsymbol{q}',\boldsymbol{k}}A^\dagger_{\boldsymbol{q}}(\boldsymbol{k}-\boldsymbol{q}'bb') \\
&-A^\dagger_{\boldsymbol{q}}(\boldsymbol{k}\tilde{b}b')\rho_{bb'\boldsymbol{k}'}\delta_{\boldsymbol{k}'+\boldsymbol{q}',\boldsymbol{k}+\boldsymbol{q}}.
\end{aligned} \tag{B3}
$$

In the first equality, the factorization approximation is made that the four-operator term is split into a product of a two-operator term and an expectation value of the rest of the two-operator term, where $\langle\hat{X}\rangle$ means an expectation value of an operator $\hat{X}$ with respect to the ground state. Further, in the second equality, the expectation value is replaced by a density matrix of the form $\rho_{bb'\boldsymbol{k}} \equiv \langle a^\dagger_{b,\boldsymbol{k}} a_{b'\boldsymbol{k}}\rangle$, based on the random-phase approximation. The similar reduction procedure is applied to the remaining four-operator terms in Eq. (B2). Thus, the commutator of $[\hat{H}_e, A^\dagger_{\boldsymbol{q}}(\boldsymbol{k}bb')]$ can be expresses as the form that is linearized with respect to a single kind of operator of the form $A^\dagger_{\boldsymbol{q}}$.

Next, the commutator of $[\hat{H}'(t), A^\dagger_{\boldsymbol{q}}(\boldsymbol{k}bb')]$ is also evaluated by use of Eq. (B1), which leads to

$$
\begin{aligned}
&[\hat{H}'(t), A^\dagger_{\boldsymbol{q}}(\boldsymbol{k}bb')] \\
&= -\frac{1}{2}\sum_{b_1 b'_1}\Big\{\Omega_{b_1 b'_1}(t)\left[A^\dagger_{\boldsymbol{q}}(\boldsymbol{k}b_1 b')\delta_{b'_1 b} - A^\dagger_{\boldsymbol{q}}(\boldsymbol{k}bb'_1)\delta_{b_1 b'}\right] \\
&+ \Omega^*_{b'_1 b_1}(t)\left[A^\dagger_{\boldsymbol{q}}(\boldsymbol{k}b'_1 b')\delta_{b_1 b} - A^\dagger_{\boldsymbol{q}}(\boldsymbol{k}bb_1)\delta_{b'_1 b'}\right]\Big\} \\
&= -\sum_{b_1 b'_1}\Omega_{b_1 b'_1}(t)\left[A^\dagger_{\boldsymbol{q}}(\boldsymbol{k}b_1 b')\delta_{b'_1 b} - A^\dagger_{\boldsymbol{q}}(\boldsymbol{k}bb'_1)\delta_{b_1 b'}\right],
\end{aligned} \tag{B4}
$$

where the fact that $\Omega^*_{b'_1 b_1}(t)$ is real is considered. Collecting the resulting expressions of Eqs. (B2) and (B4), eventually one obtains Eq. (12),

$$
[\hat{\mathcal{H}}_e(t), A^\dagger_{\boldsymbol{q}}(\boldsymbol{k}bb')] \approx \sum_{\tilde{\boldsymbol{k}}\tilde{b}\tilde{b}'} A^\dagger_{\boldsymbol{q}}(\tilde{\boldsymbol{k}}\tilde{b}\tilde{b}')Z_{\boldsymbol{q}}(\tilde{\boldsymbol{k}}\tilde{b}\tilde{b}', \boldsymbol{k}bb'), \tag{B5}
$$

where the obtained expression is found linearized with respect to the operator $A^\dagger_{\boldsymbol{q}}$, and $Z_{\boldsymbol{q}}$ is given in Eq. (13).

## APPENDIX C: SOLUTIONS OF EIGENVALUE EQUATIONS OF EQS. (22) AND (23)

First, the left eigenvalue equation of Eq. (22) is solved in an analytic manner. This equation is explicitly represented in terms of respective components of the left eigenvector $U_{\boldsymbol{q}}^{L\dagger}$ as follows:

$$U_{\boldsymbol{q}}^{L\dagger}(\boldsymbol{k}cc) = g_{cc\boldsymbol{kq}}\Bigg\{V_{\boldsymbol{q}}^{(C)}\Delta\bar{\rho}_{cc\boldsymbol{kq}}\sum_{\boldsymbol{k}'}U_{\boldsymbol{q}}^{(+)}(\boldsymbol{k}') - \left[\bar{\Omega}_{vc\boldsymbol{k}}^{(R)}\,U_{\boldsymbol{q}}^{L\dagger}(\boldsymbol{k}vc) - \bar{\Omega}_{cv\boldsymbol{k}}^{(R)}\,U_{\boldsymbol{q}}^{L\dagger}(\boldsymbol{k}cv)\right]\Bigg\}, \tag{C1}$$

$$U_{\boldsymbol{q}}^{L\dagger}(\boldsymbol{k}vv) = g_{vv\boldsymbol{kq}}\Bigg\{V_{\boldsymbol{q}}^{(C)}\Delta\bar{\rho}_{vv\boldsymbol{kq}}\sum_{\boldsymbol{k}'}U_{\boldsymbol{q}}^{(+)}(\boldsymbol{k}') + \left[\bar{\Omega}_{vc\boldsymbol{k}}^{(R)}\,U_{\boldsymbol{q}}^{L\dagger}(\boldsymbol{k}vc) - \bar{\Omega}_{cv\boldsymbol{k}}^{(R)}\,U_{\boldsymbol{q}}^{L\dagger}(\boldsymbol{k}cv)\right]\Bigg\}, \tag{C2}$$

$$U_{\boldsymbol{q}}^{L\dagger}(\boldsymbol{k}cv) = g_{cv\boldsymbol{kq}}\Bigg\{V_{\boldsymbol{q}}^{(C)}\Delta\bar{\rho}_{cv\boldsymbol{kq}}\sum_{\boldsymbol{k}'}U_{\boldsymbol{q}}^{(+)}(\boldsymbol{k}') + \bar{\Omega}_{vc\boldsymbol{k}}^{(R)}\,U_{\boldsymbol{q}}^{(-)}(\boldsymbol{k})\Bigg\}, \tag{C3}$$

and

$$U_{\boldsymbol{q}}^{L\dagger}(\boldsymbol{k}vc) = g_{vc\boldsymbol{kq}}\Bigg\{V_{\boldsymbol{q}}^{(C)}\Delta\bar{\rho}_{vc\boldsymbol{kq}}\sum_{\boldsymbol{k}'}U_{\boldsymbol{q}}^{(+)}(\boldsymbol{k}') - \bar{\Omega}_{cv\boldsymbol{k}}^{(R)}\,U_{\boldsymbol{q}}^{(-)}(\boldsymbol{k})\Bigg\}, \tag{C4}$$

where $g_{bb'\boldsymbol{kq}}$ and $U_{\boldsymbol{q}}^{(\pm)}(\boldsymbol{k})$ are defined as

$$g_{bb'\boldsymbol{kq}} = \left[\mathcal{E}_{\boldsymbol{q}\alpha} - \bar{w}_{bb'\boldsymbol{q}}\right]^{-1} \tag{C5}$$

with $\bar{w}_{bb'\boldsymbol{kq}} \equiv w_{bb'\boldsymbol{kq}} - \bar{\omega}_{bb'}$, and

$$U_{\boldsymbol{q}}^{(\pm)}(\boldsymbol{k}) = U_{\boldsymbol{q}}^{L\dagger}(\boldsymbol{k}cc) \pm U_{\boldsymbol{q}}^{L\dagger}(\boldsymbol{k}vv), \tag{C6}$$

respectively. Further, $w_{bb'\boldsymbol{q}}$ and $\bar{\Omega}_{bb'\boldsymbol{k}}^{(R)}$ are given in Eqs. (14), and (21), respectively, and $\Delta\bar{\rho}_{bb'\boldsymbol{kq}}$ is given by

$$\Delta\bar{\rho}_{bb'\boldsymbol{kq}} = \bar{\rho}_{bb'\boldsymbol{k}} - \bar{\rho}_{bb'\boldsymbol{k}+\boldsymbol{q}}. \tag{C7}$$

Eliminating $U_{\boldsymbol{q}}^{L\dagger}(\boldsymbol{k}cv)$ and $U_{\boldsymbol{q}}^{L\dagger}(\boldsymbol{k}vc)$ by putting Eqs. (C3) and (C4) into Eqs. (C1) and (C2), and further employing Eq. (C6), one obtains a set of equations for $U_{\boldsymbol{q}}^{(\pm)}(\boldsymbol{k})$:

$$U_{\boldsymbol{q}}^{(+)}(\boldsymbol{k}) = V_{\boldsymbol{q}}^{(C)}\mathcal{P}_{\boldsymbol{kq}}^{(1)}\sum_{\boldsymbol{k}'}U_{\boldsymbol{q}}^{(+)}(\boldsymbol{k}') + [g_{cc\boldsymbol{kq}} - g_{vv\boldsymbol{kq}}]W_{\boldsymbol{kq}}U_{\boldsymbol{q}}^{(-)}(\boldsymbol{k}), \tag{C8}$$

and

$$U_{\boldsymbol{q}}^{(-)}(\boldsymbol{k}) = V_{\boldsymbol{q}}^{(C)}\mathcal{P}_{\boldsymbol{kq}}^{(2)}\sum_{\boldsymbol{k}'}U_{\boldsymbol{q}}^{(+)}(\boldsymbol{k}'), \tag{C9}$$

where $\mathcal{P}_{\boldsymbol{kq}}^{(1)}$ and $\mathcal{P}_{\boldsymbol{kq}}^{(2)}$ are defined as

$$\mathcal{P}_{\boldsymbol{kq}}^{(1)} = g_{cc\boldsymbol{kq}}\Delta\bar{\rho}_{cc\boldsymbol{kq}} + g_{vv\boldsymbol{kq}}\Delta\bar{\rho}_{vv\boldsymbol{kq}} + (g_{cc\boldsymbol{kq}} - g_{vv\boldsymbol{kq}})\Delta\Omega_{\boldsymbol{kq}}, \tag{C10}$$

and

$$\mathcal{P}_{\boldsymbol{kq}}^{(2)} = \left[1 - (g_{cc\boldsymbol{kq}} + g_{vv\boldsymbol{kq}})W_{\boldsymbol{kq}}\right]^{-1} \times \left[g_{cc\boldsymbol{kq}}\Delta\bar{\rho}_{cc\boldsymbol{kq}} - g_{vv\boldsymbol{kq}}\Delta\bar{\rho}_{vv\boldsymbol{kq}} + (g_{cc\boldsymbol{kq}} + g_{vv\boldsymbol{kq}})\Delta\Omega_{\boldsymbol{kq}}\right], \tag{C11}$$

respectively. Further, $\Delta\Omega_{\boldsymbol{kq}}$ and $W_{\boldsymbol{kq}}$ are defined as

$$\Delta\Omega_{\boldsymbol{kq}} = \bar{\Omega}_{cv\boldsymbol{k}}^{(R)}g_{cv\boldsymbol{kq}}\Delta\bar{\rho}_{cv\boldsymbol{kq}} - \bar{\Omega}_{vc\boldsymbol{k}}^{(R)}g_{vc\boldsymbol{kq}}\Delta\bar{\rho}_{vc\boldsymbol{kq}}, \tag{C12}$$

and

$$W_{\boldsymbol{kq}} = \bar{\Omega}_{vc\boldsymbol{k}}^{(R)}g_{vc\boldsymbol{kq}}\bar{\Omega}_{cv\boldsymbol{k}}^{(R)} + \bar{\Omega}_{cv\boldsymbol{k}}^{(R)}g_{cv\boldsymbol{kq}}\bar{\Omega}_{vc\boldsymbol{k}}^{(R)}, \tag{C13}$$

respectively. Eliminating $U_{\boldsymbol{q}}^{(-)}(\boldsymbol{k})$ by putting Eq. (C9) into Eq. (C8) leads to

$$U_{\boldsymbol{q}}^{(+)}(\boldsymbol{k}) = V_{\boldsymbol{q}}^{(C)}\mathcal{P}_{\boldsymbol{kq}}\sum_{\boldsymbol{k}'}U_{\boldsymbol{q}}^{(+)}(\boldsymbol{k}'), \tag{C14}$$

where $\mathcal{P}_{\boldsymbol{kq}}$ is defined as

$$\mathcal{P}_{\boldsymbol{kq}} = \mathcal{P}_{\boldsymbol{kq}}^{(1)} + (g_{cc\boldsymbol{kq}} - g_{vv\boldsymbol{kq}})W_{\boldsymbol{kq}}\mathcal{P}_{\boldsymbol{kq}}^{(2)}. \tag{C15}$$

Taking the summation of both sides of Eq. (C14) over $\boldsymbol{k}$ leads to

$$\sum_{\boldsymbol{k}}U_{\boldsymbol{q}}^{(+)}(\boldsymbol{k}) = V_{\boldsymbol{q}}^{(C)}\sum_{\boldsymbol{k}}\mathcal{P}_{\boldsymbol{kq}}\sum_{\boldsymbol{k}'}U_{\boldsymbol{q}}^{(+)}(\boldsymbol{k}'). \tag{C16}$$

Therefore, one obtains an identity relation:

$$1 = V_{\boldsymbol{q}}^{(C)}\sum_{\boldsymbol{k}}\mathcal{P}_{\boldsymbol{kq}}(\mathcal{E}_{\boldsymbol{q}\alpha}), \tag{C17}$$

where energy-dependence of $\mathcal{P}_{\boldsymbol{kq}}$ is explicitly represented. Indeed, a full set of eigenenergies denoted as $\{\mathcal{E}_{\boldsymbol{q}\alpha}\}$ are determined by solving the transcendental equation of Eq. (C17). The $\alpha$th solution of $U_{\boldsymbol{q}\alpha}^{(+)}(\boldsymbol{k})$ is provided by the form:

$$U_{\boldsymbol{q}\alpha}^{(+)}(\boldsymbol{k}) = N_{\boldsymbol{q}\alpha}^{L}V_{\boldsymbol{q}}^{(C)}\mathcal{P}_{\boldsymbol{kq}}(\mathcal{E}_{\boldsymbol{q}\alpha}), \tag{C18}$$

where $N_{\boldsymbol{q}\alpha}^{L}$ is a proportional constant to be determined later. Moreover, in view of the identity relation of Eq. (C17), one obtains the following relation

$$\sum_{\boldsymbol{k}}U_{\boldsymbol{q}\alpha}^{(+)}(\boldsymbol{k}) = N_{\boldsymbol{q}\alpha}^{L}, \tag{C19}$$

and thus, by using Eq. (C9), the $\alpha$th solution of $U^{(-)}_{\boldsymbol{q}\alpha}(\boldsymbol{k})$ is provided as

$$U^{(-)}_{\boldsymbol{q}\alpha}(\boldsymbol{k}) = N^L_{\boldsymbol{q}\alpha} V^{(C)}_{\boldsymbol{q}} \mathcal{P}^{(2)}_{\boldsymbol{kq}}(\mathcal{E}_{\boldsymbol{q}\alpha}). \tag{C20}$$

Hence, due to the relation of Eq. (C6), both of $U^{L\dagger}_{\boldsymbol{q}}(\boldsymbol{k}cc)$ and $U^{L\dagger}_{\boldsymbol{q}}(\boldsymbol{k}vv)$ are determined, and further, by inserting the expressions of $U^{(\pm)}_{\boldsymbol{q}\alpha}(\boldsymbol{k})$ back into Eqs. (C3) and (C4), both of $U^{L\dagger}_{\boldsymbol{q}}(\boldsymbol{k}cv)$ and $U^{L\dagger}_{\boldsymbol{q}}(\boldsymbol{k}vc)$ are also determined. To summarize, $U^{L\dagger}_{\boldsymbol{q}}(\boldsymbol{k}bb')$ is expressed as

$$U^{L\dagger}_{\boldsymbol{q}\alpha}(\boldsymbol{k}bb') = N^L_{\boldsymbol{q}\alpha} V^{(C)}_{\boldsymbol{q}} u^{L\dagger}_{\boldsymbol{q}\alpha}(\boldsymbol{k}bb'), \tag{C21}$$

where

$$u^{L\dagger}_{\boldsymbol{q}\alpha}(\boldsymbol{k}cc) = \frac{1}{2}\left[\mathcal{P}_{\boldsymbol{kq}}(\mathcal{E}_{\boldsymbol{q}\alpha}) + \mathcal{P}^{(2)}_{\boldsymbol{kq}}(\mathcal{E}_{\boldsymbol{q}\alpha})\right], \tag{C22}$$

$$u^{L\dagger}_{\boldsymbol{q}\alpha}(\boldsymbol{k}vv) = \frac{1}{2}\left[\mathcal{P}_{\boldsymbol{kq}}(\mathcal{E}_{\boldsymbol{q}\alpha}) - \mathcal{P}^{(2)}_{\boldsymbol{kq}}(\mathcal{E}_{\boldsymbol{q}\alpha})\right], \tag{C23}$$

$$u^{L\dagger}_{\boldsymbol{q}\alpha}(\boldsymbol{k}cv) = g_{cv\boldsymbol{kq}}\left[\Delta\bar{\rho}_{cv\boldsymbol{kq}} + \bar{\Omega}^{(R)}_{vc\boldsymbol{k}} \mathcal{P}^{(2)}_{\boldsymbol{kq}}(\mathcal{E}_{\boldsymbol{q}\alpha})\right], \tag{C24}$$

and

$$u^{L\dagger}_{\boldsymbol{q}\alpha}(\boldsymbol{k}vc) = g_{vc\boldsymbol{kq}}\left[\Delta\bar{\rho}_{vc\boldsymbol{kq}} - \bar{\Omega}^{(R)}_{cv\boldsymbol{k}} \mathcal{P}^{(2)}_{\boldsymbol{kq}}(\mathcal{E}_{\boldsymbol{q}\alpha})\right]. \tag{C25}$$

Next, the right eigenvalue equation of Eq. (23) is solved in an analytic manner. This equation is explicitly represented in terms of respective components of the right eigenvector $U^R_{\boldsymbol{q}}$ as follows:

$$\begin{aligned} U^R_{\boldsymbol{q}}(\boldsymbol{k}cc) &= g_{cc\boldsymbol{kq}}\left\{V^{(C)}_{\boldsymbol{q}}\sum_{\boldsymbol{k}'} U'^{(+)}_{\boldsymbol{q}}(\boldsymbol{k}') \right.\\ &\left. + W_{\boldsymbol{kq}} U'^{(-)}_{\boldsymbol{q}}(\boldsymbol{k}')\right\}, \end{aligned} \tag{C26}$$

$$\begin{aligned} U^R_{\boldsymbol{q}}(\boldsymbol{k}vv) &= g_{vv\boldsymbol{kq}}\left\{V^{(C)}_{\boldsymbol{q}}\sum_{\boldsymbol{k}'} U'^{(+)}_{\boldsymbol{q}}(\boldsymbol{k}') \right.\\ &\left. - W_{\boldsymbol{kq}} U'^{(-)}_{\boldsymbol{q}}(\boldsymbol{k}')\right\}, \end{aligned} \tag{C27}$$

$$U^R_{\boldsymbol{q}}(\boldsymbol{k}cv) = g_{cv\boldsymbol{kq}}\bar{\Omega}^{(R)}_{cv\boldsymbol{k}} U'^{(-)}_{\boldsymbol{q}}(\boldsymbol{k}'), \tag{C28}$$

and

$$U^R_{\boldsymbol{q}}(\boldsymbol{k}vc) = -g_{vc\boldsymbol{kq}}\bar{\Omega}^{(R)}_{vc\boldsymbol{k}} U'^{(-)}_{\boldsymbol{q}}(\boldsymbol{k}'), \tag{C29}$$

where

$$U'^{(+)}_{\boldsymbol{q}}(\boldsymbol{k}) = \sum_{bb'} \Delta\bar{\rho}_{bb'\boldsymbol{kq}} U^R_{\boldsymbol{q}}(\boldsymbol{k}bb'), \tag{C30}$$

and

$$U'^{(-)}_{\boldsymbol{q}}(\boldsymbol{k}) = U^R_{\boldsymbol{q}}(\boldsymbol{k}cc) - U^R_{\boldsymbol{q}}(\boldsymbol{k}vv). \tag{C31}$$

Defining $U'^{(d)}_{\boldsymbol{q}}(\boldsymbol{k})$ as

$$U'^{(d)}_{\boldsymbol{q}}(\boldsymbol{k}) = \sum_b \Delta\bar{\rho}_{bb\boldsymbol{kq}} U^R_{\boldsymbol{q}}(\boldsymbol{k}bb), \tag{C32}$$

Eq. (C30) is rewritten as

$$U'^{(+)}_{\boldsymbol{q}}(\boldsymbol{k}) = U'^{(d)}_{\boldsymbol{q}}(\boldsymbol{k}) + \Delta\Omega_{\boldsymbol{kq}} U'^{(-)}_{\boldsymbol{q}}(\boldsymbol{k}). \tag{C33}$$

Putting Eqs. (C26) and (C27) into Eqs. (C31) and (C32), one obtains

$$U'^{(-)}_{\boldsymbol{q}}(\boldsymbol{k}) = V^{(C)}_{\boldsymbol{q}} \mathcal{P}'^{(2)}_{\boldsymbol{kq}} \sum_{\boldsymbol{k}'} U'^{(+)}_{\boldsymbol{q}}(\boldsymbol{k}'), \tag{C34}$$

and

$$\begin{aligned} U'^{(d)}_{\boldsymbol{q}}(\boldsymbol{k}) &= \left(\sum_b \Delta\bar{\rho}_{bb\boldsymbol{kq}}\, g_{bb\boldsymbol{kq}}\right) V^{(C)}_{\boldsymbol{q}} U'^{(+)}_{\boldsymbol{q}}(\boldsymbol{k}) \\ &+ \mathcal{P}'^{(3)}_{\boldsymbol{kq}} U'^{(-)}_{\boldsymbol{q}}(\boldsymbol{k}) \end{aligned} \tag{C35}$$

where

$$\begin{aligned} \mathcal{P}'^{(2)}_{\boldsymbol{kq}} &= [1 - (g_{cc\boldsymbol{kq}} + g_{vv\boldsymbol{kq}})W_{\boldsymbol{kq}}]^{-1} \\ &\times (g_{cc\boldsymbol{kq}} - g_{vv\boldsymbol{kq}})\, V^{(C)}_{\boldsymbol{q}}, \end{aligned} \tag{C36}$$

and

$$\mathcal{P}'^{(3)}_{\boldsymbol{kq}} = (\Delta\bar{\rho}_{cc\boldsymbol{kq}}\, g_{cc\boldsymbol{kq}} - \Delta\bar{\rho}_{vv\boldsymbol{kq}}\, g_{vv\boldsymbol{kq}})\, W_{\boldsymbol{kq}}. \tag{C37}$$

Putting Eqs. (C34) and (C35) into Eq. (C33) leads to

$$U'^{(+)}_{\boldsymbol{q}}(\boldsymbol{k}) = V^{(C)}_{\boldsymbol{q}} \mathcal{P}_{\boldsymbol{kq}} \sum_{\boldsymbol{k}'} U'^{(+)}_{\boldsymbol{q}}(\boldsymbol{k}'), \tag{C38}$$

which looks similar to Eq. (C14).

Therefore, taking the summation of both sides of Eq. (C38), one obtains the identity relation of Eq. (C17) again, and the $\alpha$th solution of $U'^{(+)}_{\boldsymbol{q}\alpha}(\boldsymbol{k})$ is provided by the form:

$$U'^{(+)}_{\boldsymbol{q}\alpha}(\boldsymbol{k}) = N^R_{\boldsymbol{q}\alpha} V^{(C)}_{\boldsymbol{q}} \mathcal{P}_{\boldsymbol{kq}}(\mathcal{E}_{\boldsymbol{q}\alpha}), \tag{C39}$$

with the normalization constant of $N^R_{\boldsymbol{q}\alpha}$. Further, the following relation is straightforward derived

$$\sum_{\boldsymbol{k}} U'^{(+)}_{\boldsymbol{q}\alpha}(\boldsymbol{k}) = N^R_{\boldsymbol{q}\alpha}, \tag{C40}$$

and thus, by using Eq. (C34), the $\alpha$th solution of $U'^{(-)}_{\boldsymbol{q}\alpha}(\boldsymbol{k})$ is provided as

$$U'^{(-)}_{\boldsymbol{q}\alpha}(\boldsymbol{k}) = N^R_{\boldsymbol{q}\alpha} V^{(C)}_{\boldsymbol{q}} \mathcal{P}'^{(2)}_{\boldsymbol{kq}}(\mathcal{E}_{\boldsymbol{q}\alpha}). \tag{C41}$$

$U^R_{\boldsymbol{q}}(\boldsymbol{k}bb')$ is expressed as

$$U^R_{\boldsymbol{q}\alpha}(\boldsymbol{k}bb') = N^R_{\boldsymbol{q}\alpha} V^{(C)}_{\boldsymbol{q}} u^R_{\boldsymbol{q}\alpha}(\boldsymbol{k}bb'). \tag{C42}$$

Explicit expressions of $u^R_{\boldsymbol{q}\alpha}(\boldsymbol{k}bb')$ are obtained by using Eqs. (C26)-(C29), (C39), and (C41). To summarize,

$$u^R_{\boldsymbol{q}\alpha}(\boldsymbol{k}cc) = g_{cc\boldsymbol{kq}}\left[1 + (g_{cc\boldsymbol{kq}} - g_{vv\boldsymbol{kq}})\mathcal{G}_{\boldsymbol{kq}}W_{\boldsymbol{kq}}\right], \quad (C43)$$

$$u^R_{\boldsymbol{q}\alpha}(\boldsymbol{k}vv) = g_{vv\boldsymbol{kq}}\left[1 - (g_{cc\boldsymbol{kq}} - g_{vv\boldsymbol{kq}})\mathcal{G}_{\boldsymbol{kq}}W_{\boldsymbol{kq}}\right], \quad (C44)$$

$$u^R_{\boldsymbol{q}\alpha}(\boldsymbol{k}cv) = g_{cv\boldsymbol{kq}}\bar{\Omega}^{(R)}_{\boldsymbol{k}cv}(g_{cc\boldsymbol{kq}} - g_{vv\boldsymbol{kq}})\mathcal{G}_{\boldsymbol{kq}}, \quad (C45)$$

and

$$u^R_{\boldsymbol{q}\alpha}(\boldsymbol{k}vc) = -g_{vc\boldsymbol{kq}}\bar{\Omega}^{(R)}_{\boldsymbol{k}vc}(g_{cc\boldsymbol{kq}} - g_{vv\boldsymbol{kq}})\mathcal{G}_{\boldsymbol{kq}}, \quad (C46)$$

where

$$\mathcal{G}_{\boldsymbol{kq}} = \left[1 - (g_{cc\boldsymbol{kq}} + g_{vv\boldsymbol{kq}})W_{\boldsymbol{kq}}\right]^{-1}. \quad (C47)$$

It is evident that both of the left and right eigenvectors thus obtained satisfy the biorthogonal relation

$$\sum_{\boldsymbol{k}bb'} U^{L\dagger}_{\boldsymbol{q}\alpha}(\boldsymbol{k}bb')U^R_{\boldsymbol{q}\alpha'}(\boldsymbol{k}bb') = \delta_{\alpha\alpha'}, \quad (C48)$$

and the completeness

$$\sum_{\alpha} U^R_{\boldsymbol{q}\alpha}(\boldsymbol{k}_1b_1b'_1)U^{L\dagger}_{\boldsymbol{q}\alpha}(\boldsymbol{k}_2b_2b'_2) = \delta_{\boldsymbol{k}_1\boldsymbol{k}_2}\delta_{b_1b_2}\delta_{b'_1b'_2}. \quad (C49)$$

The normalization constants, $N^L_{\boldsymbol{q}\alpha}$ and $N^R_{\boldsymbol{q}\alpha}$ are determined by the normalization condition

$$\sum_{\boldsymbol{k}bb'} U^{L\dagger}_{\boldsymbol{q}\alpha}(\boldsymbol{k}bb')U^R_{\boldsymbol{q}\alpha}(\boldsymbol{k}bb') = 1, \quad (C50)$$

In terms of Eqs. (C21) and (C42), this is of the form

$$\left[N^L_{\boldsymbol{q}\alpha}N^R_{\boldsymbol{q}\alpha}\left(V^{(C)}_{\boldsymbol{q}}\right)^2\right]^{-1} = \sum_{\boldsymbol{k}bb'} u^{L\dagger}_{\boldsymbol{q}\alpha}(\boldsymbol{k}bb')u^R_{\boldsymbol{q}\alpha}(\boldsymbol{k}bb'). \quad (C51)$$

Finally, in the small-$\boldsymbol{q}$ limit of our primary concern, a number of expressions worth while to be mentioned are derived, regarding both of the eigenenergy-determining transcendental equation of Eq. (C17) and of the normalization condition of Eq. (C51). In this limit, $\bar{\rho}_{bb'\boldsymbol{kq}}$, $g_{bb'\boldsymbol{kq}}$, and $\mathcal{G}_{\boldsymbol{kq}}$ are expressed as

$$\Delta\bar{\rho}_{bb'\boldsymbol{kq}} \simeq -|\boldsymbol{q}|\hat{\boldsymbol{q}}\cdot\boldsymbol{\nabla}\bar{\rho}_{bb'\boldsymbol{k}}, \quad (C52)$$

$$g_{bb\boldsymbol{kq}} \simeq \frac{1}{\mathcal{E}_{\boldsymbol{q}}}\left(1 + \frac{1}{\mathcal{E}_{\boldsymbol{q}}}|\boldsymbol{q}|\hat{\boldsymbol{q}}\cdot\boldsymbol{\nabla}\varepsilon^{(r)}_{b\boldsymbol{k}}\right), \quad (C53)$$

$$g_{b\bar{b}\boldsymbol{kq}} \simeq g_{b\bar{b}\boldsymbol{k},\boldsymbol{q}=\boldsymbol{0}} \equiv g_{b\bar{b}\boldsymbol{k}}, \quad (C54)$$

and

$$\mathcal{G}_{\boldsymbol{kq}} = \left(1 - \frac{2W_{\boldsymbol{kq}}}{\mathcal{E}_{\boldsymbol{q}}}\right)^{-1}, \quad (C55)$$

where $\boldsymbol{\nabla}$ means a gradient with respect to $\boldsymbol{k}$, namely, $\partial/\partial\boldsymbol{k}$, $\varepsilon^{(r)}_{b\boldsymbol{k}}$ is given in Eq.(15), $\hat{\boldsymbol{q}} = \boldsymbol{q}/|\boldsymbol{q}|$, and $\bar{b}$ means $\bar{b} \neq b$. Equation (C17) becomes of the form

$$K(\mathcal{E}_{\boldsymbol{q}}) = 1, \quad (C56)$$

where

$$\begin{aligned}
&K(\mathcal{E}_{\boldsymbol{q}}) \\
&= \frac{V^{(C)}_{\boldsymbol{q}}\boldsymbol{q}^2}{\mathcal{E}^2_{\boldsymbol{q}}}\sum_{\boldsymbol{k}}\Big\{\bar{\rho}_{cc\boldsymbol{k}}\left(\hat{\boldsymbol{q}}\cdot\boldsymbol{\nabla}\right)\Big[\left(\hat{\boldsymbol{q}}\cdot\boldsymbol{\nabla}\varepsilon^{(r)}_{c\boldsymbol{k}}\right) \\
&+ \left(\hat{\boldsymbol{q}}\cdot\boldsymbol{\nabla}\Delta\varepsilon^{(r)}_{\boldsymbol{k}}\right)\frac{W_{\boldsymbol{kq}}\mathcal{G}_{\boldsymbol{kq}}}{\mathcal{E}_{\boldsymbol{q}}}\Big] + \bar{\rho}_{vv\boldsymbol{k}}\left(\hat{\boldsymbol{q}}\cdot\boldsymbol{\nabla}\right)\Big[\left(\hat{\boldsymbol{q}}\cdot\boldsymbol{\nabla}\varepsilon^{(r)}_{v\boldsymbol{k}}\right) \\
&- \left(\hat{\boldsymbol{q}}\cdot\boldsymbol{\nabla}\Delta\varepsilon^{(r)}_{\boldsymbol{k}}\right)\frac{W_{\boldsymbol{kq}}\mathcal{G}_{\boldsymbol{kq}}}{\mathcal{E}_{\boldsymbol{q}}}\Big] + \bar{\rho}_{cv\boldsymbol{k}}\left(\hat{\boldsymbol{q}}\cdot\boldsymbol{\nabla}\right)\Big[\left(\hat{\boldsymbol{q}}\cdot\boldsymbol{\nabla}\Delta\varepsilon^{(r)}_{\boldsymbol{k}}\right) \\
&\times\bar{\Omega}^{(R)}_{\boldsymbol{k}cv}g_{\boldsymbol{k}cv}\left(1 + \frac{2W_{\boldsymbol{kq}}\mathcal{G}_{\boldsymbol{kq}}}{\mathcal{E}_{\boldsymbol{q}}}\right)\Big] - \bar{\rho}_{vc\boldsymbol{k}}\left(\hat{\boldsymbol{q}}\cdot\boldsymbol{\nabla}\right) \\
&\times\Big[\left(\hat{\boldsymbol{q}}\cdot\boldsymbol{\nabla}\Delta\varepsilon^{(r)}_{\boldsymbol{k}}\right)\bar{\Omega}^{(R)}_{\boldsymbol{k}vc}g_{\boldsymbol{k}vc}\left(1 + \frac{2W_{\boldsymbol{kq}}\mathcal{G}_{\boldsymbol{kq}}}{\mathcal{E}_{\boldsymbol{q}}}\right)\Big]\Big\}
\end{aligned} \quad (C57)$$

with

$$\Delta\varepsilon^{(r)}_{\boldsymbol{k}} = \varepsilon^{(r)}_{c\boldsymbol{k}} - \varepsilon^{(r)}_{v\boldsymbol{k}}. \quad (C58)$$

Using Eqs. (C5) and(C13), and defining

$$D_{\boldsymbol{kq}}(\mathcal{E}_{\boldsymbol{q}}) = \mathcal{E}^2_{\boldsymbol{q}} - \bar{w}^2_{cv\boldsymbol{kq}} - |2\bar{\Omega}^{(R)}_{\boldsymbol{k}cv}|^2, \quad (C59)$$

Eq. (C57) is of the explicit form that

$$\begin{aligned}
&K(\mathcal{E}_{\boldsymbol{q}}) \\
&= \frac{1}{\mathcal{E}^2_{\boldsymbol{q}}}\Big(\omega^2_{pl} + \frac{4\pi}{\epsilon_\infty}\sum_{\boldsymbol{k}}\Big\{\frac{1}{2}\left(\bar{\rho}_{cc\boldsymbol{k}} - \bar{\rho}_{vv\boldsymbol{k}}\right) \\
&\times\left(\hat{\boldsymbol{q}}\cdot\boldsymbol{\nabla}\right)\left[\left(\hat{\boldsymbol{q}}\cdot\boldsymbol{\nabla}\Delta\varepsilon^{(r)}_{\boldsymbol{k}}\right)\frac{|2\bar{\Omega}^{(R)}_{\boldsymbol{k}cv}|^2}{D_{\boldsymbol{kq}}(\mathcal{E}_{\boldsymbol{q}})}\right] \\
&+\bar{\rho}_{cv\boldsymbol{k}}\left(\hat{\boldsymbol{q}}\cdot\boldsymbol{\nabla}\right)\left[\left(\hat{\boldsymbol{q}}\cdot\boldsymbol{\nabla}\Delta\varepsilon^{(r)}_{\boldsymbol{k}}\right)\frac{\bar{\Omega}^{(R)}_{\boldsymbol{k}cv}(\mathcal{E}_{\boldsymbol{q}} + \bar{w}_{cv\boldsymbol{kq}})}{D_{\boldsymbol{kq}}(\mathcal{E}_{\boldsymbol{q}})}\right] \\
&- \bar{\rho}_{vc\boldsymbol{k}}\left(\hat{\boldsymbol{q}}\cdot\boldsymbol{\nabla}\right)\left[\left(\hat{\boldsymbol{q}}\cdot\boldsymbol{\nabla}\Delta\varepsilon^{(r)}_{\boldsymbol{k}}\right)\frac{\bar{\Omega}^{(R)}_{\boldsymbol{k}vc}(\mathcal{E}_{\boldsymbol{q}} + \bar{w}_{vc\boldsymbol{kq}})}{D_{\boldsymbol{kq}}(\mathcal{E}_{\boldsymbol{q}})}\right]\Big\}\Big).
\end{aligned} \quad (C60)$$

Here, $\omega_{pl}$ represents plasma frequency, defined as

$$\omega^2_{pl} = \frac{4\pi N_{ex}}{\epsilon_\infty m_{cv}}, \quad (C61)$$

where $N_{ex}$ means excited electron density, given by

$$N_{ex} = \frac{1}{V}\sum_{\boldsymbol{k}}\bar{\rho}_{cc\boldsymbol{k}}, \quad (C62)$$

and $m_{cv}$ is reduced mass of an electron in a joint band composed of $c$ and $v$ bands under an effective mass approximation. In the case that the Rabi frequency terms,

$\bar{\Omega}^{(R)}_{\boldsymbol{k}cv}$ and $\bar{\Omega}^{(R)}_{\boldsymbol{k}vc}$, are neglected, Eq.(C56) is straightforward solved to provide $\mathcal{E}^2_{\boldsymbol{q}}$ that equals $\omega^2_{pl}$.

Next, it is shown that Eq. (C51) is of the form

$$\left[N^L_{\boldsymbol{q}\alpha}N^R_{\boldsymbol{q}\alpha}\left(V^{(C)}_{\boldsymbol{q}}\right)^2\right]^{-1} = -\frac{\boldsymbol{q}^2}{\mathcal{E}^2_{\boldsymbol{q}\alpha}}\sum_{\boldsymbol{k}bb'}\left(\hat{\boldsymbol{q}}\cdot\boldsymbol{\nabla}\rho_{bb'\boldsymbol{k}}\right)f_{bb'\boldsymbol{k}}, \tag{C63}$$

where

$$f_{cc\boldsymbol{k}} = \frac{1}{\mathcal{E}_{\boldsymbol{q}}}\left[(\hat{\boldsymbol{q}}\cdot\boldsymbol{\nabla})\left(\varepsilon^{(r)}_{c\boldsymbol{k}}+\varepsilon^{(r)}_{v\boldsymbol{k}}\right)+\left(\hat{\boldsymbol{q}}\cdot\boldsymbol{\nabla}\Delta\varepsilon^{(r)}_{\boldsymbol{k}}\right)\mathcal{G}_{\boldsymbol{kq}}d_{\boldsymbol{kq}}\right], \tag{C64}$$

$$f_{vv\boldsymbol{k}} = \frac{1}{\mathcal{E}_{\boldsymbol{q}}}\left[(\hat{\boldsymbol{q}}\cdot\boldsymbol{\nabla})\left(\varepsilon^{(r)}_{c\boldsymbol{k}}+\varepsilon^{(r)}_{v\boldsymbol{k}}\right)-\left(\hat{\boldsymbol{q}}\cdot\boldsymbol{\nabla}\Delta\varepsilon^{(r)}_{\boldsymbol{k}}\right)\mathcal{G}_{\boldsymbol{kq}}d_{\boldsymbol{kq}}\right], \tag{C65}$$

$$f_{cv\boldsymbol{k}} = \left(\hat{\boldsymbol{q}}\cdot\boldsymbol{\nabla}\Delta\varepsilon^{(r)}_{\boldsymbol{k}}\right)g_{cv\boldsymbol{k}}\bar{\Omega}^{(R)}_{\boldsymbol{k}cv}\mathcal{G}_{\boldsymbol{kq}}\left(g_{cv\boldsymbol{k}}+\frac{2d_{\boldsymbol{kq}}}{\mathcal{E}_{\boldsymbol{q}}}\right), \tag{C66}$$

and

$$f_{vc\boldsymbol{k}} = -\left(\hat{\boldsymbol{q}}\cdot\boldsymbol{\nabla}\Delta\varepsilon^{(r)}_{\boldsymbol{k}}\right)g_{vc\boldsymbol{k}}\bar{\Omega}^{(R)}_{\boldsymbol{k}vc}\mathcal{G}_{\boldsymbol{kq}}\left(g_{vc\boldsymbol{k}}+\frac{2d_{\boldsymbol{kq}}}{\mathcal{E}_{\boldsymbol{q}}}\right), \tag{C67}$$

with

$$\begin{aligned} d_{\boldsymbol{kq}} &= 1+\mathcal{G}_{\boldsymbol{kq}}W_{\boldsymbol{kq}}\left(\frac{1}{\mathcal{E}_{\boldsymbol{q}}}+\frac{g^2_{cv\boldsymbol{k}}+g^2_{vc\boldsymbol{k}}}{g_{cv\boldsymbol{k}}+g_{vc\boldsymbol{k}}}\right) \\ &\approx 1+\frac{2}{\mathcal{E}_{\boldsymbol{q}}}\mathcal{G}_{\boldsymbol{kq}}W_{\boldsymbol{kq}}\approx\mathcal{G}_{\boldsymbol{kq}}. \end{aligned} \tag{C68}$$

It is noted that the normalization constant $N_{\boldsymbol{q}}$, and both of $u^{L\dagger}_{\boldsymbol{q}}$ and $u^R_{\boldsymbol{q}}$ become proportional to $|\boldsymbol{q}|$ in the small $\boldsymbol{q}$-limit.

Moreover, making a replacement of $\mathcal{E}_{\boldsymbol{q}\alpha}$ by $-\mathcal{E}^*_{\boldsymbol{q}\alpha}$ in Eq. (C60), followed by taking a complex conjugate of both sides of this equation, one readily obtains a relation

$$K(\mathcal{E}_{\boldsymbol{q}\alpha}) = \left[K(-\mathcal{E}^*_{\boldsymbol{q}\alpha})\right]^*. \tag{C69}$$

This implies that a pair of $\mathcal{E}_{\boldsymbol{q}\alpha_+}$ and $\mathcal{E}_{\boldsymbol{q}\alpha_-}(\equiv -\mathcal{E}^*_{\boldsymbol{q}\alpha_+})$ are solutions of Eq. (C56) at the same time. Applying the same procedure to Eq. (C63) also leads to a relation

$$N^L_{\boldsymbol{q}\alpha_+}N^R_{\boldsymbol{q}\alpha_+} = -\left[N^L_{\boldsymbol{q}\alpha_-}N^R_{\boldsymbol{q}\alpha_-}\right]^*. \tag{C70}$$

According to an energy-phase of $\exp\left[i\int^t_{t'}\mathcal{E}_{\boldsymbol{q}\alpha}(\tau)d\tau\right]$ in Eq. (32), it is seen that $\mathcal{E}_{\boldsymbol{q}\alpha_+}$ plays a role of a complex energy of a quasi-boson created by an operator of $B^\dagger_{\boldsymbol{q}\alpha_+}$, where amplitude of this operator temporally diminishes, following $\exp\left[-\int^t_{t'}\mathrm{Im}\mathcal{E}_{\boldsymbol{q}\alpha_+}(\tau)d\tau\right]$. Similarly, since an energy-phase of $B_{\boldsymbol{q}\alpha_-}$ is given by $\exp\left[-i\int^t_{t'}\mathcal{E}^*_{\boldsymbol{q}\alpha}(\tau)d\tau\right]$, $\mathcal{E}_{\boldsymbol{q}\alpha_-}$ is interpreted straightforward as a complex energy of a quasi-boson annihilated by this operator, where amplitude of it damps, following $\exp\left[-\int^t_{t'}\mathrm{Im}\mathcal{E}_{\boldsymbol{q}\alpha_+}(\tau)d\tau\right]$ again.

## APPENDIX D: CLOSED ANALYTIC FORMS OF $F^\dagger_{\boldsymbol{q}\beta}$ AND $F_{\boldsymbol{q}\beta}$ DERIVED BY SOLVING EQ. (67)

### 1. Introduction of Operators of $F^{0\dagger}_{\boldsymbol{q}\beta}$ and $F^0_{\boldsymbol{q}\beta}$

Prior to solving Eq. (67), an equation of motion of another PQ operator

$$F^{0\dagger}_{\boldsymbol{q}} = [B^{0\dagger}_{\boldsymbol{q}}, c^\dagger_{\boldsymbol{q}}]V_{\boldsymbol{q}}, \tag{D1}$$

is considered, which is given by

$$-i\frac{d}{dt}F^{0\dagger}_{\boldsymbol{q}\beta} = F^{0\dagger}_{\boldsymbol{q}\beta}E^0_{\boldsymbol{q}\beta}, \tag{D2}$$

where Eq. (D1) mimics Eq. (58) by introducing a quasi-boson operator $B^{0\dagger}_{\boldsymbol{q}}$ and an $[(N+2)\times N]$-rectangular matrix $V_{\boldsymbol{q}}$ differing from $B^\dagger_{\boldsymbol{q}}$ and $V^R_{\boldsymbol{q}}$, respectively. $V_{\boldsymbol{q}}$ satisfies an equation different from Eq. (57), that is,

$$h^0_{\boldsymbol{q}}V_{\boldsymbol{q}} = V_{\boldsymbol{q}}E^0_{\boldsymbol{q}}, \tag{D3}$$

where $h^0_{\boldsymbol{q}}$ is a hermitian matrix, given by

$$h^0_{\boldsymbol{q}} = \begin{pmatrix} \mathcal{E}^0_{\boldsymbol{q}} & M_{\boldsymbol{q}} \\ M^\dagger_{\boldsymbol{q}} & \omega^{(LO)}_{\boldsymbol{q}} \end{pmatrix}, \tag{D4}$$

and in addition, $\mathcal{E}^0_{\boldsymbol{q}}$ is real, as defined below Eq. (D14), with $E^0_{\boldsymbol{q}\beta} = \mathcal{E}^0_{\boldsymbol{q}\bar{\alpha}}$. Further, similarly to Eq. (59), an $[N\times(N+2)]$-rectangular matrix $\bar{V}_{\boldsymbol{q}}$ is introduced to ensure the inverse relation of Eq. (D1), that is,

$$[B^{0\dagger}_{\boldsymbol{q}}, c^\dagger_{\boldsymbol{q}}] = F^{0\dagger}_{\boldsymbol{q}}\bar{V}_{\boldsymbol{q}}. \tag{D5}$$

Thus, one obtains

$$\bar{V}_{\boldsymbol{q}}V_{\boldsymbol{q}} = 1, \tag{D6}$$

and

$$V_{\boldsymbol{q}}\bar{V}_{\boldsymbol{q}} = 1 \tag{D7}$$

which correspond to the expressions given right below Eq. (59) for $V^R_{\boldsymbol{q}}$ and $\bar{V}^R_{\boldsymbol{q}}$. In addition, following Eq. (61), $F^0_{\boldsymbol{q}}$ is introduced as a hermitian-conjugate of $F^{0\dagger}_{\boldsymbol{q}}$, namely,

$$F^0_{\boldsymbol{q}} = V^\dagger_{\boldsymbol{q}}\begin{bmatrix} B^0_{\boldsymbol{q}} \\ c_{\boldsymbol{q}} \end{bmatrix}. \tag{D8}$$

Here, both of $F^0_{\boldsymbol{q}\beta}$ and $F^{0\dagger}_{\boldsymbol{q}\beta}$ are required to ensure the following expectation values of equal-time commutation relations as

$$\langle[F^0_{\boldsymbol{q}\beta}, F^{0\dagger}_{\boldsymbol{q}'\beta'}]\rangle = \delta_{\boldsymbol{qq}'}\delta_{\beta\beta'}, \tag{D9}$$

and

$$\langle[F^0_{\boldsymbol{q}\beta}, F^0_{\boldsymbol{q}'\beta'}]\rangle = \langle[F^{0\dagger}_{\boldsymbol{q}\beta}, F^{0\dagger}_{\boldsymbol{q}'\beta'}]\rangle = 0, \tag{D10}$$

instead of the corresponding equal-time commutation relations in which expectation values are not taken. Under

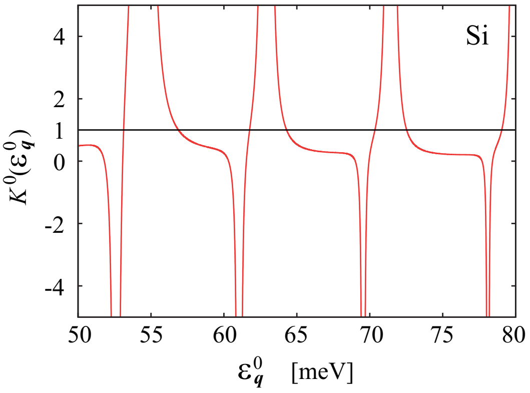


FIG. D-1: (Color Online) A trace of $K^0(\mathcal{E}^0_{\boldsymbol{q}})$ as a function of $\mathcal{E}^0_{\boldsymbol{q}}$. A horizontal solid line shows $K^0(\mathcal{E}^0_{\boldsymbol{q}}) = 1$.

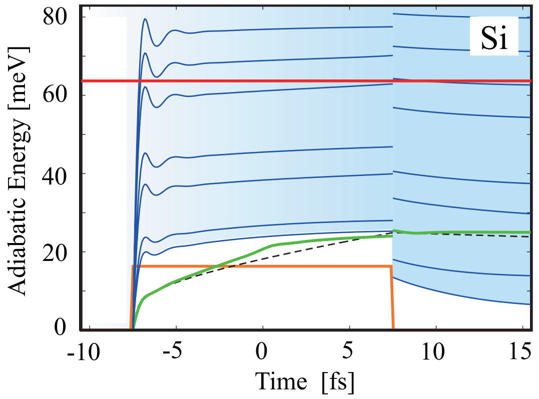


FIG. D-2: (Color Online) Adiabatic energy curves of Si (in the unit of meV) as a function of time $t$ (in the unit of fs). The curves are calculated based on Eq. (D14). A plasmon-like mode is represented by a green solid line, and a bundle of the electron-hole continua is represented by blue solid lines. Further, the alteration of bare Rabi frequency $\Omega_{0cv}$ as a function of $t$ is represented by an orange solid line; here this is of squared shape [see Eq. (19)]. In addition, the LO-phonon energy, $\omega^{(LO)}_{\boldsymbol{q}} = 63$ meV, is represented by a red solid line, and plasmon energy proportional to total excited electron density $N_{ex}(t)$ is represented by a broken line, just for the purpose of comparison of the plasmon-like mode. The gradation of blue color shows schematic change of $N_{ex}(t)$ in $t$, where the lowest limit of this gradation represents the threshold energy of a bundle of the electron-hole continua.

these conditions, $F^0_{\boldsymbol{q}\beta}$ and $F^{0\dagger}_{\boldsymbol{q}\beta}$ would be allowed to be considered as boson operators. In Eqs. (D9) and (D10), the argument $t$ of these operators is omitted just for the sake of simplicity. Applying Eqs. (D1) and (D8) to Eqs. (D9) and (D10), it is readily shown that the following conditions are imposed on $B^0_{\boldsymbol{q}\alpha}$, $B^{0\dagger}_{\boldsymbol{q}\alpha}$, and $\bar{V}_{\boldsymbol{q}}$ as:

$$\langle [B^0_{\boldsymbol{q}\alpha}, B^{0\dagger}_{\boldsymbol{q}'\alpha'}] \rangle = \delta_{\boldsymbol{q}\boldsymbol{q}'}\delta_{\alpha\alpha'}, \tag{D11}$$

$$\langle [B^0_{\boldsymbol{q}\alpha}, B^0_{\boldsymbol{q}'\alpha'}] \rangle = \langle [B^{0\dagger}_{\boldsymbol{q}\alpha}, B^{0\dagger}_{\boldsymbol{q}'\alpha'}] \rangle = 0. \tag{D12}$$

and

$$\bar{V}_{\boldsymbol{q}} = V^\dagger_{\boldsymbol{q}}. \tag{D13}$$

In Sec. D 3, one examines the criteria of the validity of the bosonization scheme just mentioned above.

A set of solutions $V_{\boldsymbol{q}}$ of the Fano problem given by the adiabatic coupled-equations of Eq. (D3) is provided in Sec. D 4. On the other hand, a set of eigenvalues $\mathcal{E}^0_{\boldsymbol{q}}$ is determined by

$$K^0(\mathcal{E}^0_{\boldsymbol{q}}) = 1, \tag{D14}$$

where an explicit expression of $K^0(\mathcal{E}^0_{\boldsymbol{q}})$ is given by

$$\begin{aligned} &K^0(\mathcal{E}^0_{\boldsymbol{q}}) \\ &= \left(\frac{1}{\mathcal{E}^0_{\boldsymbol{q}}}\right)^2 \left\{ \omega^2_{pl} + \frac{4\pi}{\epsilon_\infty} \sum_{\boldsymbol{k}} \frac{1}{2} (\bar{\rho}_{cc\boldsymbol{k}} - \bar{\rho}_{vv\boldsymbol{k}}) \, (\hat{\boldsymbol{q}} \cdot \boldsymbol{\nabla}) \right. \\ &\times \left. \left[ \left( \hat{\boldsymbol{q}} \cdot \boldsymbol{\nabla} \Delta\varepsilon^{(r)}_{\boldsymbol{k}} \right) \frac{|2\bar{\Omega}^{(R)}_{\boldsymbol{k}cv}|^2}{\left(\mathcal{E}^0_{\boldsymbol{q}}\right)^2 - \bar{w}^2_{cv\boldsymbol{k}\boldsymbol{q}} - |2\bar{\Omega}^{(R)}_{\boldsymbol{k}cv}|^2} \right] \right\}. \end{aligned} \tag{D15}$$

Here, $\omega_{pl}$ is a plasma frequency given below Eq. (35), $\hat{\boldsymbol{q}} = \boldsymbol{q}/|\boldsymbol{q}|$, and $\boldsymbol{\nabla} \equiv \partial/\partial\boldsymbol{k}$. [In fact, $K^0(\mathcal{E}^0_{\boldsymbol{q}})$ is substituted for $K(\mathcal{E}_{\boldsymbol{q}})$ of Eq. (C60) by making a consistent approximation with the approximation for deriving Eq. (D50) from Eq. (D46), namely, by both adopting the equality of Eq. (D56) and neglecting interband density matrices.]

Below, a couple of properties of solutions of the transcendental equation of Eq. (D14) are discussed. A trace of $K^0(\mathcal{E}^0_{\boldsymbol{q}})$ as a function of $\mathcal{E}^0_{\boldsymbol{q}}$ is shown in Fig. D-1 for Si; the similar trace to this figure for GaAs is also obtained, though not shown here. Points of intersection of $K^0(\mathcal{E}^0_{\boldsymbol{q}})$ with unity correspond to *real* solutions of Eq. (D15). [It should be noted that just a set of solutions the normalization constants of which satisfy Eq. (D57) is eligible for the present bosonization scheme; to be more concrete, usually just either of adjacent points of intersection ensures this condition.] Hereafter, it is understood that the normalization constants for state $\alpha$ are express as

$$N^L_{\boldsymbol{q}\alpha} = N^{R*}_{\boldsymbol{q}\alpha} \equiv N^0_{\boldsymbol{q}\alpha}, \tag{D16}$$

with $N^0_{\boldsymbol{q}\alpha}$ real, unless otherwise stated. Existence of such a set of real eigenvalues, $\{\mathcal{E}^0_{\boldsymbol{q}\alpha}\}$, is in harmony with the demand that $h^0_{\boldsymbol{q}}$ should be hermitian.

This set of eigenvalues is shown in the adiabatic energy curve of Fig. D-2. It seems that this curve well reproduces that shown in Fig. 2 calculated without the bosonization scheme. This fact would demonstrate the validity of this scheme. Further, it is pointed out that even after laser irradiation is brought to completion, $\bar{\Omega}^{(R)}_{\boldsymbol{k}cv}$ does not vanish due to the Coulomb correction. On the occasion of $\bar{\Omega}^{(R)}_{\boldsymbol{k}cv} = 0$, Eq. (D15) provides just solutions

of $\mathcal{E}^0_{\boldsymbol{q}} = \pm\omega_{pl}$, and the electron-hole continuum states become absent from the adiabatic energy curves of Fig. D-2. Therefore, it should be noted that the Coulomb correction is significant so as to form the continuum states, to which a discrete state of LO-phonon is coupled, resulting in FR after the completion of laser irradiation.

According to Fig. D-1, it is seen that the eigenvalues pertaining to continuum states $\bar{\alpha}$'s are located in the proximity of the poles ascribable to the denominator in the square brackets of the right-hand side of Eq. (D15), aside from a solution of $\mathcal{E}^0_{\boldsymbol{q}\alpha_1}$ corresponding to a plasmon. Therefore, the eigenvalue for the $\bar{\alpha}$ state is well approximated to be

$$\mathcal{E}^0_{\boldsymbol{q}\bar{\alpha}} \approx \pm\sqrt{\bar{w}^2_{cv\boldsymbol{k}\boldsymbol{q}} + |2\bar{\Omega}^{(R)}_{\boldsymbol{k}cv}|^2}, \tag{D17}$$

and further, the index $\bar{\alpha}$ can be considered approximately as equal to Bloch momentum $|\boldsymbol{k}|$: regarding plus and minus signs of Eq. (D17), consult Eq.(C69).

### 2. Approximate Solutions of $F^\dagger_{\boldsymbol{q}\beta}$ and $F_{\boldsymbol{q}\beta}$

Equation (67) is solved in an approximate manner in terms of the PQ operators of $F^{0\dagger}_{\boldsymbol{q}\beta}$ introduced above. To do this, a new operator $\tilde{F}^{0\dagger}_{\boldsymbol{q}\beta}$ is defined first as

$$\tilde{F}^{0\dagger}_{\boldsymbol{q}\beta}(t) = F^{0\dagger}_{\boldsymbol{q}\beta}(t)\, e^{-\mathfrak{Z}^*_{\boldsymbol{q}\beta}(t,t_0)}. \tag{D18}$$

where $t_0$ is initial time when an initial condition is imposed before laser irradiation: $t_0 < -\tau_L/2$. Here, both effects of the phenomenological damping and the non-adiabatic correction attributed to diagonal components are incorporated in

$$\mathfrak{Z}_{\boldsymbol{q}\beta}(t,\tilde{t}) = \int_{\tilde{t}}^{t} dt' \left[\frac{\gamma^{(0)}_{\boldsymbol{q}\beta}(t')}{2} + I^*_{\boldsymbol{q}\beta\beta}(t')\right]. \tag{D19}$$

For the sake of later convenience, $\mathfrak{I}_{\boldsymbol{q}\beta}(t,\bar{t})$ is defined as

$$\mathfrak{I}_{\boldsymbol{q}\beta}(t,\bar{t}) = \int_{\tilde{t}}^{t} dt' I^*_{\boldsymbol{q}\beta\beta}(t'). \tag{D20}$$

Thus, it is readily seen from Eq. (D2) that $\tilde{F}^{0\dagger}_{\boldsymbol{q}\beta}(t)$ satisfies the equation of motion given by

$$\begin{aligned} &-i\frac{d}{dt}\tilde{F}^{0\dagger}_{\boldsymbol{q}\beta}(t) \\ &= \tilde{F}^{0\dagger}_{\boldsymbol{q}\beta}(t)\left\{E^0_{\boldsymbol{q}\beta}(t) + i\left[\frac{\gamma^{(0)}_{\boldsymbol{q}\beta}(t)}{2} + I_{\boldsymbol{q}\beta\beta}(t)\right]\right\}. \end{aligned} \tag{D21}$$

Subtracting Eq. (D21) from Eq. (67) side by side with defining $\Delta F^\dagger_{\boldsymbol{q}\beta}$ as

$$\Delta F^\dagger_{\boldsymbol{q}\beta} = F^\dagger_{\boldsymbol{q}\beta} - \tilde{F}^{0\dagger}_{\boldsymbol{q}\beta}, \tag{D22}$$

the following equation of motion is obtained as:

$$\begin{aligned} &-i\frac{d}{dt}\Delta F^\dagger_{\boldsymbol{q}\beta}(t) \\ &= \Delta F^\dagger_{\boldsymbol{q}\beta}(t)\left\{E_{\boldsymbol{q}\beta}(t) + i\left[\frac{\gamma^{(0)}_{\boldsymbol{q}\beta}(t)}{2} + I_{\boldsymbol{q}\beta\beta}(t)\right]\right\} \\ &+i\sum_{\beta'(\neq\beta)}\left[\tilde{F}^{0\dagger}_{\boldsymbol{q}\beta'}(t) + \Delta F^\dagger_{\boldsymbol{q}\beta'}(t)\right] I_{\boldsymbol{q}\beta'\beta}(t) \\ &+\tilde{F}^{0\dagger}_{\boldsymbol{q}\beta}(t)\left[E_{\boldsymbol{q}\beta}(t) - E^0_{\boldsymbol{q}\beta}(t)\right]. \end{aligned} \tag{D23}$$

The formal solution of this is provided by

$$\begin{aligned} \Delta F^\dagger_{\boldsymbol{q}\beta}(t) &= \Delta F^\dagger_{\boldsymbol{q}\beta}(t_0)e^{i\Theta^*_{\boldsymbol{q}\beta}(t,t_0)} \\ &- \sum_{\beta'(\neq\beta)}\int_{t_0}^{t} dt'\left[\tilde{F}^{0\dagger}_{\boldsymbol{q}\beta'}(t') + \Delta F^\dagger_{\boldsymbol{q}\beta'}(t')\right] \\ &\times I_{\boldsymbol{q}\beta'\beta}(t')e^{-i\left[\Theta^*_{\boldsymbol{q}\beta}(t',t_0) - \Theta^*_{\boldsymbol{q}\beta}(t,t_0)\right]} \\ &+i\int_{t_0}^{t} dt'\tilde{F}^{0\dagger}_{\boldsymbol{q}\beta}(t')\left[E_{\boldsymbol{q}\beta}(t') - E^0_{\boldsymbol{q}\beta}(t')\right] \\ &\times e^{-i\left[\Theta^*_{\boldsymbol{q}\beta}(t',t_0) - \Theta^*_{\boldsymbol{q}\beta}(t,t_0)\right]}, \end{aligned} \tag{D24}$$

where $\Theta_{\boldsymbol{q}\beta}(t,\tilde{t})$ is an adiabatic energy phase given by

$$\begin{aligned} &\Theta_{\boldsymbol{q}\beta}(t,\tilde{t}) \\ &= \int_{\tilde{t}}^{t} dt'\left\{E^*_{\boldsymbol{q}\beta}(t') - i\left[\frac{\gamma^{(0)}_{\boldsymbol{q}\beta}(t')}{2} + I^*_{\boldsymbol{q}\beta\beta}(t)\right]\right\}. \end{aligned} \tag{D25}$$

It is supposed that the initial condition of the above equation is given by

$$\Delta F^\dagger_{\boldsymbol{q}\beta}(t_0) = 0, \tag{D26}$$

that is, $F^\dagger_{\boldsymbol{q}\beta}(t_0) = F^{0\dagger}_{\boldsymbol{q}\beta}(t_0)$, with an additional approximation that $E^*_{\boldsymbol{q}\beta}(t) \approx E^0_{\boldsymbol{q}\beta}(t)$ which leads to

$$\begin{aligned} &\Theta_{\boldsymbol{q}\beta}(t,\tilde{t}) \\ &\approx \int_{\tilde{t}}^{t} dt'\left\{E^0_{\boldsymbol{q}\beta}(t') - i\left[\frac{\gamma^{(0)}_{\boldsymbol{q}\beta}(t')}{2} + I^*_{\boldsymbol{q}\beta\beta}(t')\right]\right\}. \end{aligned} \tag{D27}$$

Therefore, Eq. (D24) becomes

$$\begin{aligned} \Delta F^\dagger_{\boldsymbol{q}\beta}(t) &\approx -\sum_{\beta'(\neq\beta)}\int_{t_0}^{t} dt'\left[\tilde{F}^{0\dagger}_{\boldsymbol{q}\beta'}(t') + \Delta F^\dagger_{\boldsymbol{q}\beta'}(t')\right] \\ &\times I_{\boldsymbol{q}\beta'\beta}(t')e^{-i\left[\Theta^*_{\boldsymbol{q}\beta}(t',t_0) - \Theta^*_{\boldsymbol{q}\beta}(t,t_0)\right]}. \end{aligned} \tag{D28}$$

As seen in the second equality of Eq. (64), the non-adiabatic interaction $I_{\boldsymbol{q}}(t)$ is affected by the two contributions, namely, $W_{\boldsymbol{q}}(t)$ and a time-derivative of $\bar{V}^R_{\boldsymbol{q}}(t)$. There are two pronounced effects on $W_{\boldsymbol{q}}(t)$. One is an effect of a crossing between adiabatic states of $\alpha'$ and $\alpha$.

Here, the adiabatic energy curves of $\mathcal{E}_{\boldsymbol{q}\alpha'}(t)$ and $\mathcal{E}_{\boldsymbol{q}\alpha}(t)$ tend to swerve sharply in the vicinity of the crossing region around $t = t_j$ due to a Landau-Zener coupling, resulting in spike-like change; it is seen that this effect arises from the energy denominator in Eq. (35) [2]. The similar change is also caused in the second term of the second equality of Eq. (64). The other is an effect of abrupt change of $\Omega^{(R)}_{bb'\boldsymbol{k}}(t)$ of Eq. (13), namely, $d\Omega^{(R)}_{bb'\boldsymbol{k}}(t)/dt$, at $t = \pm\tau_L/2$ because of the impulsive temporal-shape of $F_0(t)$ of Eq. (19). This effect would be dominant even off a temporal region of a Resen-Zener-Demkov coupling, where adiabatic energy curves run parallel each other [2]. Accordingly, $I_{\boldsymbol{q}}(t)$ would be well described by

$$I_{\boldsymbol{q}}(t) \approx \sum_j \mathfrak{I}^{(j)\dagger}_{\boldsymbol{q}} \delta(t - t_j), \tag{D29}$$

where it is understood that a set of $t_j$'s also includes $\pm\tau_L/2$, and $\mathfrak{I}^{(j)}_{\boldsymbol{q}}$ is a constant matrix with $\mathfrak{I}^{(j)\dagger}_{\boldsymbol{q}} \neq -\mathfrak{I}^{(j)}_{\boldsymbol{q}}$.

Putting Eq. (D29) into Eq. (D28) yields

$$\begin{aligned}&\Delta F^{\dagger}_{\boldsymbol{q}\beta}(t)\\ &\approx -\sum_j \sum_{\beta'(\neq\beta)} \left[\tilde{F}^{0\dagger}_{\boldsymbol{q}\beta'}(t_j) + \Delta F^{\dagger}_{\boldsymbol{q}\beta'}(t_j)\right]\\ &\times \mathfrak{I}^{(j)*}_{\boldsymbol{q}\beta'\beta}\theta(t - t_j) e^{-i\left[\Theta^*_{\boldsymbol{q}\beta}(t_j,t_0) - \Theta^*_{\boldsymbol{q}\beta}(t,t_0)\right]}. \end{aligned}\tag{D30}$$

From among a set of the off-diagonal elements $\{\mathfrak{I}^{(j)}_{\boldsymbol{q}\beta'\neq\beta}\}$, let just the single leading contribution, namely, at $t = t_D$, be retained. In practical calculations, $t_D$ is set equal to $\tau_L/2$, that is,

$$t_D = \frac{\tau_L}{2}. \tag{D31}$$

Thus, one obtains

$$\begin{aligned}&\Delta F^{\dagger}_{\boldsymbol{q}\beta}(t_D)\\ &\approx -\sum_{\beta'} \tilde{F}^{0\dagger}_{\boldsymbol{q}\beta'}(t_D) \left[\phi_{\boldsymbol{q}}(t_D) \frac{1}{1 + \phi_{\boldsymbol{q}}(t_D)}\right]_{\beta'\beta}, \end{aligned}\tag{D32}$$

where

$$\phi_{\boldsymbol{q}\beta'\beta}(t) = \mathfrak{I}^{(D)*}_{\boldsymbol{q}\beta'\beta}\theta(t - t_D)\bar{\delta}_{\beta'\beta} \tag{D33}$$

with $\bar{\delta}_{\beta'\beta} = 1 - \delta_{\beta'\beta}$. If more than two contributions of $\{\mathfrak{I}^{(j)}_{\boldsymbol{q}\beta'\neq\beta}\}$ are retained, a set of $\Delta F^{\dagger}_{\boldsymbol{q}\beta}(t_j)$'s is obtained in a more complicated closed-form than Eq. (D32). Hereafter, just $\mathfrak{I}^{(D)}_{\boldsymbol{q}\beta'\beta}$ is taken account of simply because the present theoretical framework is described succinctly.

Putting Eq. (D32) back into Eq. (D30), $\Delta F^{\dagger}_{\boldsymbol{q}\beta}(t)$ is provided by

$$\begin{aligned}\Delta F^{\dagger}_{\boldsymbol{q}\beta}(t) &\approx -e^{i\Theta^*_{\boldsymbol{q}\beta}(t,t_0)} \sum_{\beta'} F^{0\dagger}_{\boldsymbol{q}\beta'}(t_0)\\ &\times \left[\frac{1}{1 + \tilde{\phi}_{\boldsymbol{q}}(t_D)} \tilde{\phi}_{\boldsymbol{q}}(t)\right]_{\beta'\beta}, \end{aligned}\tag{D34}$$

where $\tilde{\phi}_{\boldsymbol{q}}$ is defined as

$$\tilde{\phi}_{\boldsymbol{q}\beta'\beta}(t) = e^{i\Theta^*_{\beta'}(t_D,t_0)} \phi_{\boldsymbol{q}\beta'\beta}(t) e^{-i\Theta^*_{\beta}(t_D,t_0)}, \tag{D35}$$

and Eq. (D18) is used. Therefore, in view of Eq. (D22), $F^{\dagger}_{\boldsymbol{q}\beta}(t)$ is given by

$$\begin{aligned}F^{\dagger}_{\boldsymbol{q}\beta}(t) &= e^{i\Theta^*_{\boldsymbol{q}\beta}(t,t_0)} \sum_{\beta'} F^{0\dagger}_{\boldsymbol{q}\beta'}(t_0)\\ &\times \left[\frac{1 + \tilde{\phi}_{\boldsymbol{q}}(t_D) - \tilde{\phi}_{\boldsymbol{q}}(t)}{1 + \tilde{\phi}_{\boldsymbol{q}}(t_D)}\right]_{\beta'\beta}\\ &= e^{i\Theta^*_{\boldsymbol{q}\beta}(t,t_D)} \sum_{\beta'} F^{0\dagger}_{\boldsymbol{q}\beta'}(t_D) \mathcal{T}'_{\boldsymbol{q}\beta'\beta}(t), \end{aligned}\tag{D36}$$

and taking its hermitian-conjugate yields

$$F_{\boldsymbol{q}\beta}(t) = e^{-i\Theta_{\boldsymbol{q}\beta}(t,t_D)} \sum_{\beta'} \mathcal{T}'^{\dagger}_{\boldsymbol{q}\beta\beta'}(t) F^{0}_{\boldsymbol{q}\beta'}(t_D), \tag{D37}$$

where the off-diagonal components of non-adiabatic interaction are renormalized to $\mathcal{T}'_{\boldsymbol{q}}(t)$ defined as

$$\begin{aligned}&\mathcal{T}'_{\boldsymbol{q}\beta'\beta}(t)\\ &= \left[\frac{1 + \tilde{\phi}_{\boldsymbol{q}}(t_D) - \tilde{\phi}_{\boldsymbol{q}}(t)}{1 + \tilde{\phi}_{\boldsymbol{q}}(t_D)}\right]_{\beta'\beta} e^{-\mathfrak{I}^*_{\boldsymbol{q}\beta}(t_D,t_0)}. \end{aligned}\tag{D38}$$

In terms of $F_{\boldsymbol{q}}$ and $F^{\dagger}_{\boldsymbol{q}}$ thus obtained, the associated retarded Green function [3] is defined as

$$G^R_{\boldsymbol{q}\beta\beta'}(t,t') = -i\theta(t - t')\Big\langle\Big[F_{\boldsymbol{q}\beta}(t), F^{\dagger}_{\boldsymbol{q}\beta'}(t')\Big]\Big\rangle, \tag{D39}$$

and the concomitant advanced Green function [3] is given by

$$G^A_{\boldsymbol{q}\beta\beta'}(t,t') = \left[G^R_{\boldsymbol{q}\beta'\beta}(t',t)\right]^*. \tag{D40}$$

Thus, putting Eqs. (D36) and (D37) into Eq. (D39), the retarded Green function ends up with

$$\begin{aligned}&G^R_{\boldsymbol{q}\beta\beta'}(t,t')\\ &= -i\theta(t - t') e^{-i\Theta_{\boldsymbol{q}\beta}(t,t_D)} \sum_{\gamma\gamma'} V^{R\dagger}_{\boldsymbol{q}\beta\gamma}(t_D)\\ &\times T_{\boldsymbol{q}\gamma\gamma'}(t,t') V^R_{\boldsymbol{q}\gamma'\beta'}(t_D) e^{i\Theta^*_{\boldsymbol{q}\beta'}(t',t_D)}, \end{aligned}\tag{D41}$$

where Eq. (D9) is employed. Here, the matrix of $T_{\boldsymbol{q}}$ is introduced for the purpose of later convenience as

$$T_{\boldsymbol{q}}(t,t') = \mathcal{T}^{\dagger}_{\boldsymbol{q}}(t)\mathcal{T}_{\boldsymbol{q}}(t'), \tag{D42}$$

where

$$\mathcal{T}_{\boldsymbol{q}}(t) = \mathcal{T}'_{\boldsymbol{q}}(t)\bar{V}^R_{\boldsymbol{q}}(t_D). \tag{D43}$$

Similarly to Eq. (D41), the expectation values of equal-time commutation relations for the PQ operators are evaluated as

$$\begin{aligned}\langle[F_{\boldsymbol{q}\beta}(t), F^{\dagger}_{\boldsymbol{q}'\beta'}(t)]\rangle &= e^{-i\Theta_{\boldsymbol{q}\beta}(t,t_D)} \sum_{\gamma\gamma'} V^{R\dagger}_{\boldsymbol{q}\beta\gamma}(t_D) T_{\boldsymbol{q}\gamma\gamma'}(t,t)\\ &\times V^R_{\boldsymbol{q}\gamma'\beta'}(t_D) e^{i\Theta^*_{\boldsymbol{q}\beta'}(t,t_D)}, \end{aligned}\tag{D44}$$

and

$$\langle [F_{\boldsymbol{q}\beta}(t), F_{\boldsymbol{q}'\beta'}(t)] \rangle = \langle [F^{\dagger}_{\boldsymbol{q}\beta}(t), F^{\dagger}_{\boldsymbol{q}'\beta'}(t)] \rangle = 0, \qquad \text{(D45)}$$

due to Eq. (D10).


[2] E. E. Nikitin and S. Ya. Umanskii, *Theory of Slow Atomic Collisions*, Springer Series in Chemical Physics **30**, (Springer-Verlag, Berlin, 1984) Chap. 7.

[3] W. Schäfer and M. Wegener, *Semiconductor Optics and Transport Phenomena* (Springer-Verlag, Berlin, 2002) Chaps. 2, 10, and 11.


### 3. Bosonization Scheme and its Approximate Validity

First, an expectation value of $\langle [B_{\boldsymbol{q}\alpha}, B^{\dagger}_{\boldsymbol{q}'\alpha'}] \rangle$ is evaluated. This is reduced to

$$\begin{aligned}
&\langle [B_{\boldsymbol{q}\alpha}, B^{\dagger}_{\boldsymbol{q}'\alpha'}] \rangle \\
&= \sum_{\boldsymbol{k}\boldsymbol{k}'b_1b_1'b_2b_2'} U^{R\dagger}_{\boldsymbol{q}\alpha}(\boldsymbol{k}b_1b_1') \\
&\times \langle [\bar{A}_{\boldsymbol{q}}(\boldsymbol{k}b_1b_1'), \bar{A}^{\dagger}_{\boldsymbol{q}'}(\boldsymbol{k}'b_2b_2')] \rangle U^{R}_{\boldsymbol{q}'\alpha'}(\boldsymbol{k}'b_2b_2') \\
&= \delta_{\boldsymbol{q}\boldsymbol{q}'} \sum_{\boldsymbol{k}b_2b_3} \left\{ \sum_{\boldsymbol{k}b_1} \left[ U^{R\dagger}_{\boldsymbol{q}\alpha}(\boldsymbol{k}b_1b_2)\bar{\rho}_{b_1b_3\boldsymbol{k}} \right.\right. \\
&\left.\left. - U^{R\dagger}_{\boldsymbol{q}\alpha}(\boldsymbol{k}b_3b_1)\bar{\rho}_{b_2b_1\boldsymbol{k}+\boldsymbol{q}} \right] \right\} U^{R}_{\boldsymbol{q}\alpha'}(\boldsymbol{k}b_2b_3), \qquad \text{(D46)}
\end{aligned}$$

where Eqs.(28) and (33) is used in the first equality. Here, $\bar{U}^{L\dagger}_{\boldsymbol{q}\alpha}$ is defined as the term in the curl brackets of the second equality of the right-hand side of Eq. (D46), that is,

$$\bar{U}^{L\dagger}_{\boldsymbol{q}\alpha}(\boldsymbol{k}b_2b_3) = N^{R*}_{\boldsymbol{q}\alpha} V^{(C)}_{\boldsymbol{q}} \bar{u}^{L\dagger}_{\boldsymbol{q}\alpha}(\boldsymbol{k}b_2b_3), \qquad \text{(D47)}$$

where

$$\begin{aligned}
\bar{u}^{L\dagger}_{\boldsymbol{q}\alpha}(\boldsymbol{k}b_2b_3) \ &= \ \sum_{b_1} \left[ u^{R\dagger}_{\boldsymbol{q}\alpha}(\boldsymbol{k}b_1b_2)\bar{\rho}_{b_1b_3\boldsymbol{k}} \right. \\
&\left. - u^{R\dagger}_{\boldsymbol{q}\alpha}(\boldsymbol{k}b_3b_1)\bar{\rho}_{b_2b_1\boldsymbol{k}+\boldsymbol{q}} \right]. \qquad \text{(D48)}
\end{aligned}$$

[It is remarked that an eigenvalue associated with an eigenvector of $u^{R\dagger}_{\boldsymbol{q}\alpha}$ is $\mathcal{E}^*_{\boldsymbol{q}\alpha}$ because of $U^{R\dagger}_{\boldsymbol{q}}\bar{Z}^{\dagger}_{\boldsymbol{q}} = \mathcal{E}^*_{\boldsymbol{q}}U^{R\dagger}_{\boldsymbol{q}}$, which is readily obtained by Eq. (23). Thus, every component of $u^{R\dagger}_{\boldsymbol{q}\alpha}$ is given by $u^{R}_{\boldsymbol{q}\alpha}$ of Eqs. (C43)-(C45), followed by replacing $\mathcal{E}_{\boldsymbol{q}\alpha}$ by $\mathcal{E}^*_{\boldsymbol{q}\alpha}$ and by taking its complex-conjugate.] Thus, Eq. (D46) becomes of the form

$$\langle [B_{\boldsymbol{q}\alpha}, B^{\dagger}_{\boldsymbol{q}'\alpha'}] \rangle = \delta_{\boldsymbol{q}\boldsymbol{q}'} \sum_{\boldsymbol{k}b_2b_3} \bar{U}^{L\dagger}_{\boldsymbol{q}\alpha}(\boldsymbol{k}b_2b_3) U^{R}_{\boldsymbol{q}\alpha'}(\boldsymbol{k}b_2b_3). \qquad \text{(D49)}$$

If $\bar{U}^{L\dagger}_{\boldsymbol{q}\alpha}(\boldsymbol{k}b_2b_3)$ were in exact agreement with $U^{L\dagger}_{\boldsymbol{q}\alpha}(\boldsymbol{k}b_2b_3)$, the expectation value of concern would satisfy a desirable relation of

$$\langle [B_{\boldsymbol{q}\alpha}, B^{\dagger}_{\boldsymbol{q}'\alpha'}] \rangle = \delta_{\boldsymbol{q}\boldsymbol{q}'}\delta_{\alpha\alpha'} \qquad \text{(D50)}$$

because of $U^{L\dagger}_{\boldsymbol{q}}U^{R}_{\boldsymbol{q}} = 1$.

Below, the quantity of

$$\begin{aligned}
r_{\alpha\alpha'} \ &= \ \left| \delta_{\alpha\alpha'} - \langle [B_{\boldsymbol{q}\alpha}, B^{\dagger}_{\boldsymbol{q}'\alpha'}] \rangle \right| \\
&= \ \left| \sum_{\boldsymbol{k}bb'} \left[ U^{L\dagger}_{\boldsymbol{q}\alpha}(\boldsymbol{k}bb') - \bar{U}^{L\dagger}_{\boldsymbol{q}\alpha}(\boldsymbol{k}bb') \right] U^{R}_{\boldsymbol{q}\alpha'}(\boldsymbol{k}bb') \right|
\end{aligned} \qquad \text{(D51)}$$

is evaluated within a small-$|\boldsymbol{q}|$ limit. $r_{\alpha\alpha'}$ serves as an estimate of a criterion of the validity of concern. First, one obtains the following expression as:

$$\begin{aligned}
&\sum_{\boldsymbol{k}bb'} \left[ u^{L\dagger}_{\boldsymbol{q}\alpha}(\boldsymbol{k}bb') - \bar{u}^{L\dagger}_{\boldsymbol{q}\alpha}(\boldsymbol{k}bb') \right] u^{R}_{\boldsymbol{q}\alpha'}(\boldsymbol{k}bb') \\
&= -\frac{\boldsymbol{q}^2}{2\mathcal{E}^3_{\hat{\boldsymbol{q}}\alpha'}} \sum_{\boldsymbol{k}} \left[ \hat{\boldsymbol{q}} \cdot \boldsymbol{\nabla} \left( \bar{\rho}_{cc\boldsymbol{k}} - \bar{\rho}_{vv\boldsymbol{k}} \right) \right] \left( \hat{\boldsymbol{q}} \cdot \boldsymbol{\nabla}\Delta\varepsilon^{(r)}_{\boldsymbol{k}} \right) \\
&\times \frac{|2\bar{\Omega}^{(R)}_{\boldsymbol{k}cv}|^2}{\mathcal{E}^2_{\boldsymbol{q}\alpha}} \left( 1 + \frac{|2\bar{\Omega}^{(R)}_{\boldsymbol{k}cv}|^2}{\mathcal{E}^2_{\boldsymbol{q}\alpha}} \right) \left( 1 + \frac{|2\bar{\Omega}^{(R)}_{\boldsymbol{k}cv}|^2}{\mathcal{E}^2_{\boldsymbol{q}\alpha'}} \right) \\
&\times \left( 1 + \frac{|2\bar{\Omega}^{(R)}_{\boldsymbol{k}cv}|^2}{\mathcal{E}_{\boldsymbol{q}\alpha}\mathcal{E}_{\boldsymbol{q}\alpha'}} \right) \\
&+ (\text{terms factorized by } \bar{\rho}_{cv\boldsymbol{k}}, \bar{\rho}_{vc\boldsymbol{k}}, \Delta\Omega_{\boldsymbol{k}\boldsymbol{q}}). \qquad \text{(D52)}
\end{aligned}$$

On the other hand, the associated normalization constant is rewritten as

$$\begin{aligned}
&\left[ N^{L}_{\boldsymbol{q}\alpha} N^{R}_{\boldsymbol{q}\alpha} \left( V^{(C)}_{\boldsymbol{q}} \right)^2 \right]^{-1} \\
&= -\frac{\boldsymbol{q}^2}{\mathcal{E}^2_{\boldsymbol{q}\alpha}} \sum_{\boldsymbol{k}b} \left( \hat{\boldsymbol{q}} \cdot \boldsymbol{\nabla}\rho_{b\boldsymbol{k}} \right) f_{b\boldsymbol{k}} \\
&+ (\text{terms factorized by } \bar{\rho}_{cv\boldsymbol{k}}, \bar{\rho}_{vc\boldsymbol{k}}) \\
&= -\frac{\boldsymbol{q}^2}{\mathcal{E}^3_{\boldsymbol{q}\alpha}} \sum_{\boldsymbol{k}} \left[ \hat{\boldsymbol{q}} \cdot \boldsymbol{\nabla} \left( \bar{\rho}_{cc\boldsymbol{k}} - \bar{\rho}_{vv\boldsymbol{k}} \right) \right] \left( \hat{\boldsymbol{q}} \cdot \boldsymbol{\nabla}\Delta\varepsilon^{(r)}_{\boldsymbol{k}} \right) \\
&\times \left[ \mathcal{G}_{\boldsymbol{k}\boldsymbol{q}}(\mathcal{E}_{\boldsymbol{q}\alpha}) \right]^2 + (\text{terms factorized by } \bar{\rho}_{cv\boldsymbol{k}}, \bar{\rho}_{vc\boldsymbol{k}}).
\end{aligned} \qquad \text{(D53)}$$

[It is remarked that the normalization constant is given in Eq. (C63), and $\mathcal{G}_{\boldsymbol{k}\boldsymbol{q}}$ is expressed as

$$\mathcal{G}_{\boldsymbol{k}\boldsymbol{q}}(\mathcal{E}_{\boldsymbol{q}\alpha}) \approx \left( 1 - \frac{|2\bar{\Omega}^{(R)}_{\boldsymbol{k}cv}|^2}{\mathcal{E}^2_{\boldsymbol{q}\alpha}} \right)^{-1} \qquad \text{(D54)}$$

due to Eqs. (C13) and (C55).]

According to Eq. (D51), $r_{\alpha\alpha'}$ is cast into

$$\begin{aligned}
r_{\alpha\alpha'} \ &= \ \left| N^{L}_{\boldsymbol{q}\alpha} N^{R}_{\boldsymbol{q}\alpha'} \left( V^{(C)}_{\boldsymbol{q}} \right)^2 \right| \\
&\times \left| \sum_{\boldsymbol{k}bb'} \left[ u^{L\dagger}_{\boldsymbol{q}\alpha}(\boldsymbol{k}bb') - \frac{N^{R*}_{\boldsymbol{q}\alpha}}{N^{L}_{\boldsymbol{q}\alpha}} \bar{u}^{L\dagger}_{\boldsymbol{q}\alpha}(\boldsymbol{k}bb') \right] u^{R}_{\boldsymbol{q}\alpha'}(\boldsymbol{k}bb') \right|.
\end{aligned} \qquad \text{(D55)}$$

For the purpose of obtaining more explicit expression of $r_{\alpha\alpha'}$, Eq. (D55) is evaluated by making the following approximations. First, $N^{R*}_{\boldsymbol{q}\alpha}$ is made equal to $N^L_{\boldsymbol{q}\alpha}$. That is,

$$N^{R*}_{\boldsymbol{q}\alpha} = N^L_{\boldsymbol{q}\alpha}, \tag{D56}$$

which provides the result that

$$N^L_{\boldsymbol{q}\alpha} N^R_{\boldsymbol{q}\alpha} = |N^R_{\boldsymbol{q}\alpha}|^2 > 0. \tag{D57}$$

Second, in both of Eqs. (D52) and (D53), the terms factorized by $\bar{\rho}_{cv\boldsymbol{k}}$, $\bar{\rho}_{vc\boldsymbol{k}}$, and $\Delta\Omega_{\boldsymbol{kq}}$ are neglected, and further, just the leading contributions from expanded series of both of these equations with respect to $|2\bar{\Omega}^{(R)}_{\boldsymbol{k}cv}|/\mathcal{E}_{\boldsymbol{q}\alpha}$ and $|2\bar{\Omega}^{(R)}_{\boldsymbol{k}cv}|/\mathcal{E}_{\boldsymbol{q}\alpha'}$ are retained: in fact, $\Delta\Omega_{\boldsymbol{kq}}$ itself is factorized in terms of $\bar{\rho}_{cv\boldsymbol{k}}$ and $\bar{\rho}_{vc\boldsymbol{k}}$, as seen in Eq. (C12).

Therefore, Eq. (D55) results in a modulus of a ratio of Eq. (D52) to Eq. (D53). One obtains

$$\begin{aligned} r_{\alpha\alpha'} &\approx \left| \frac{\sum_{\boldsymbol{k}} [\hat{\boldsymbol{q}}\cdot\boldsymbol{\nabla}(\bar{\rho}_{cc\boldsymbol{k}} - \bar{\rho}_{vv\boldsymbol{k}})] \left(\hat{\boldsymbol{q}}\cdot\boldsymbol{\nabla}\Delta\varepsilon^{(r)}_{\boldsymbol{k}}\right) |2\bar{\Omega}^{(R)}_{\boldsymbol{k}cv}|^2}{2\mathcal{E}^{1/2}_{\boldsymbol{q}\alpha}\mathcal{E}^{3/2}_{\boldsymbol{q}\alpha'} \sum_{\boldsymbol{k}} [\hat{\boldsymbol{q}}\cdot\boldsymbol{\nabla}(\bar{\rho}_{cc\boldsymbol{k}} - \bar{\rho}_{vv\boldsymbol{k}})] \left(\hat{\boldsymbol{q}}\cdot\boldsymbol{\nabla}\Delta\varepsilon^{(r)}_{\boldsymbol{k}}\right)} \right| \\ &\approx \frac{1}{2}\left| \frac{\Omega^2_{0cv}}{\mathcal{E}^{1/2}_{\boldsymbol{q}\alpha}\mathcal{E}^{3/2}_{\boldsymbol{q}\alpha'}} \right| \le \frac{1}{2} x^2_{\alpha\alpha'}, \end{aligned} \tag{D58}$$

where in the second equality, a Coulomb correction to $\bar{\Omega}^{(R)}_{\boldsymbol{k}cv}$ given in Eq. (16) is neglected just for the sake of simplicity, and $x_{\alpha\alpha'}$ is defined as a ratio of Rabi frequency $\Omega_{0cv}$ to $\mathrm{Min}(|\mathcal{E}_{\boldsymbol{q}\alpha}|, |\mathcal{E}_{\boldsymbol{q}\alpha'}|)$, namely,

$$x_{\alpha\alpha'} = \frac{\Omega_{0cv}}{\mathrm{Min}(|\mathcal{E}_{\boldsymbol{q}\alpha}|, |\mathcal{E}_{\boldsymbol{q}\alpha'}|)}. \tag{D59}$$

Hence $r_{\alpha\alpha'}$ becomes negligibly small under a condition of $x_{\alpha\alpha'} \ll 1$.

Eventually, a criterion of the approximate validity of the relation

$$\langle [B_{\boldsymbol{q}\alpha}, B^\dagger_{\boldsymbol{q}'\alpha'}] \rangle \approx \delta_{\boldsymbol{qq}'}\delta_{\alpha\alpha'} \tag{D60}$$

can be found. It is stated that this commutation relation holds correctly under the condition that the left and right eigenvectors of $U^{L\dagger}_{\boldsymbol{q}}(z)$ and $U^R_{\boldsymbol{q}}(z)$, respectively, are assumed to be real functions of an argument $z$, and further, that a rough estimate of $x^2_{\alpha\alpha'}/2$ is much smaller than unity. The first condition corresponds to Eq. (D56) together with the procedure of neglecting terms that are factorized by interband density matrices of $\bar{\rho}_{cv\boldsymbol{k}}$ and $\bar{\rho}_{vc\boldsymbol{k}}$, which has the above-mentioned left and right eigenvectors complex. This condition is one of the necessary conditions for the bosonization scheme developed here. Without this, eigenenergy $\mathcal{E}_{\boldsymbol{q}\alpha}$ remains complex in general.

On the other hand, an expectation value of $\langle [B^\dagger_{\boldsymbol{q}\alpha}, B^\dagger_{\boldsymbol{q}'\alpha'}] \rangle$ causes mixing of PQs with different momenta through the effective coupling constant $\mathcal{M}''_{-\boldsymbol{q}\alpha}$ of Eq. (62). This coupling would be disregarded due to a higher-order effect in Eq. (60) compared with the first and second terms of the right-hand side, as long as the magnitude of $M''_{-\boldsymbol{q}\alpha}$ of Eq. (40) is considered as negligibly small. Hereafter, it is supposed that little of the CP generation dynamics would be affected by such an inter-PQ interaction, as already stated at the end of Sec. IIA2. As a result of the approximations made here, the relation of

$$\langle [B_{\boldsymbol{q}\alpha}, B_{\boldsymbol{q}'\alpha'}] \rangle = \langle [B^\dagger_{\boldsymbol{q}\alpha}, B^\dagger_{\boldsymbol{q}'\alpha'}] \rangle = 0 \tag{D61}$$

can be assumed, and thus, the effective coupling constants of $M''_{-\boldsymbol{q}\alpha}$ and $M'^*_{\boldsymbol{q}\alpha}$ are reduced to $M''_{-\boldsymbol{q}\alpha} = 0$ and $M'^*_{\boldsymbol{q}\alpha} = M^*_{\boldsymbol{q}\alpha}$, respectively. Eventually, the quasi-boson operators of $B_{\boldsymbol{q}\alpha}$ and $B^\dagger_{\boldsymbol{q}'\alpha'}$ satisfying Eqs. (D50) and (D61) are eligible for the boson operators of $B^0_{\boldsymbol{q}\alpha}$ and $B^{0\dagger}_{\boldsymbol{q}'\alpha'}$, respectively, both of which are introduced in Sec. D 1.

Finally, by consulting Fig. D-2 for adiabatic energy curves of $\mathcal{E}^0_{\boldsymbol{q}\alpha}$, one confirms the criterion of the validity of the bosonization scheme for the operators, $B^0_{\boldsymbol{q}\alpha}$ and $B^{0\dagger}_{\boldsymbol{q}'\alpha'}$. This energy is approximately expresses by Eq. (D17). Thus, threshold energy $|\mathcal{E}^0_{\boldsymbol{q}\bar{\alpha}_{th}}|$ of the band of $\{|\mathcal{E}^0_{\boldsymbol{q}\bar{\alpha}}|\}$ is determined by the Rabi frequency, that is,

$$|\mathcal{E}^0_{\boldsymbol{q}\bar{\alpha}_{th}}| \approx 2|\bar{\Omega}^{(R)}_{\boldsymbol{k}cv}| \approx \Omega_{0cv}, \tag{D62}$$

where in the second equality, a Coulomb correction to $\bar{\Omega}^{(R)}_{\boldsymbol{k}cv}$ is neglected just for the sake of simplicity. Because of $|\mathcal{E}^0_{\boldsymbol{q}\bar{\alpha}}| \ge |\mathcal{E}^0_{\boldsymbol{q}\bar{\alpha}_{th}}|$, it seems that most of continuum states $\bar{\alpha}$'s satisfy the criterion of the validity of the present bosonization scheme of Eq. (D58), that is, $r_{\bar{\alpha}\bar{\alpha}'} \approx x^2_{\bar{\alpha}\bar{\alpha}'}/2 \ll 1$, where $x_{\bar{\alpha}\bar{\alpha}'} = |\mathcal{E}^0_{\boldsymbol{q}\bar{\alpha}th}|/\mathrm{Min}(|\mathcal{E}^0_{\boldsymbol{q}\bar{\alpha}}|, |\mathcal{E}^0_{\boldsymbol{q}\bar{\alpha}'}|)$ [see Eq. (D59)]. On the other hand, a plasmon state $\alpha_1$ with $|\mathcal{E}^0_{\boldsymbol{q}\alpha_1}| \le |\mathcal{E}^0_{\boldsymbol{q}\bar{\alpha}_{th}}|$ would not ensure the criterion of the validity, while this condition is still applicable to a plasmon state with $|\mathcal{E}^0_{\boldsymbol{q}\alpha_1}| \gg |\mathcal{E}^0_{\boldsymbol{q}\bar{\alpha}_{th}}|$. In particular, after laser irradiation is brought to completion where $\Omega_{0cv}$ vanishes, Eq. (D50) would be satisfied, as obviously seen from Eq. (D58); it is remarked that to be precise, $\bar{\Omega}^{(R)}_{\boldsymbol{k}cv}$ does not vanish due to the Coulomb correction even after the laser irradiation completes, as stated above. Thus, in such a situation, a plasmon would be also considered as a boson.

#### 4. Solutions of the Fano Problem given by Adiabatic Coupled-Equations of Eq. (D3)

Solutions of the Fano Problem given by Eq. (D3) are sought in this section. Hereafter, just for the sake of typographical simplicity, it is understood that a superscript "0" of $h^0_{\boldsymbol{q}}$, $N^0_{\boldsymbol{q}}$, $\Delta N^0_{\boldsymbol{q}}$, $E^0_{\boldsymbol{q}}$, and $\mathcal{E}^0_{\boldsymbol{q}}$ is omitted, and these notations are replaced by non-superscript counterparts of $h_{\boldsymbol{q}}$, $N_{\boldsymbol{q}}$, $\Delta N_{\boldsymbol{q}}$, $E_{\boldsymbol{q}}$, and $\mathcal{E}_{\boldsymbol{q}}$, respectively, as far as it is not likely to cause unnecessary confusion between them. Thus, Eq. (D3) is read as

$$h_{\boldsymbol{q}} V_{\boldsymbol{q}} = V_{\boldsymbol{q}} E_{\boldsymbol{q}}, \tag{D63}$$

where the hermitian matrix $h_{\boldsymbol{q}}$ is given by

$$h_{\boldsymbol{q}} = \begin{bmatrix} \mathcal{E}_{\boldsymbol{q}} & 0 & M_{\boldsymbol{q}} \\ 0 & \omega_{\boldsymbol{q}\alpha_1} & M_{\boldsymbol{q}\alpha_1} \\ M_{\boldsymbol{q}}^{\dagger} & M_{\boldsymbol{q}\alpha_1}^{*} & \omega_{\boldsymbol{q}\alpha_2} \end{bmatrix} \equiv \begin{bmatrix} \mathcal{E}_{\boldsymbol{q}} & z_{\boldsymbol{q}} \\ z_{\boldsymbol{q}}^{\dagger} & h_{\boldsymbol{q}}^{(d)} \end{bmatrix}. \quad \text{(D64)}$$

Recall the notations used right below Eq. (57), where $N$ and $N_0$ means the number of discretized continua and the number of independent solutions of Eq. (E5), respectively. Here, $\mathcal{E}_{\boldsymbol{q}} = \{\mathcal{E}_{\boldsymbol{q}\bar{\alpha}}\delta_{\bar{\alpha}\bar{\alpha}'}\}$ is a $(N \times N)$-diagonal matrix, $M_{\boldsymbol{q}} = \{M_{\boldsymbol{q}\bar{\alpha}}\}$ is a $(N \times 1)$-matrix, $\epsilon_{\boldsymbol{q}\alpha_1} \equiv \mathcal{E}_{\boldsymbol{q}\alpha_1}$, and $\epsilon_{\boldsymbol{q}\alpha_2} \equiv \omega_{\boldsymbol{q}}^{(LO)}$. Further, $z_{\boldsymbol{q}}$ is a $(N \times 2)$-matrix and $h_{\boldsymbol{q}}^{(d)}$ is a $(2 \times 2)$-matrix, given by

$$z_{\boldsymbol{q}} = \begin{bmatrix} 0 & M_{\boldsymbol{q}} \end{bmatrix} \quad \text{(D65)}$$

and

$$h_{\boldsymbol{q}}^{(d)} = \begin{bmatrix} \epsilon_{\boldsymbol{q}\alpha_1} & M_{\boldsymbol{q}\alpha_1} \\ M_{\boldsymbol{q}\alpha_1}^{*} & \epsilon_{\boldsymbol{q}\alpha_2} \end{bmatrix}, \quad \text{(D66)}$$

respectively.

The Fano problem of concern is a scattering problem with a given energy $\mathcal{E}_{\boldsymbol{q}\bar{\alpha}}$ with one open-channel and two closed channels: $N_0 = N$ [4]. Therefore, Eq. (E5) is of the form of

$$h_{\boldsymbol{q}} \begin{bmatrix} \eta_{\boldsymbol{q}} \\ \nu_{\boldsymbol{q}} \end{bmatrix} = \begin{bmatrix} \eta_{\boldsymbol{q}} \\ \nu_{\boldsymbol{q}} \end{bmatrix} \mathcal{E}_{\boldsymbol{q}}, \quad \text{(D67)}$$

where $h_{\boldsymbol{q}}$ is defined in Eq. (E6) as:

$$h_{\boldsymbol{q}} = \begin{bmatrix} \mathcal{E}_{\boldsymbol{q}} & z_{\boldsymbol{q}} \\ z_{\boldsymbol{q}}^{\dagger} & h_{\boldsymbol{q}}^{(d)} \end{bmatrix}, \quad \text{(D68)}$$

and $V_{\boldsymbol{q}}$ is replaced by $V_{\boldsymbol{q}} = {}^{t}[\eta_{\boldsymbol{q}}, \nu_{\boldsymbol{q}}]$. Here, $\eta_{\boldsymbol{q}} = \{\eta_{\boldsymbol{q}\bar{\alpha}\bar{\alpha}}\}$ and $\nu_{\boldsymbol{q}} = \{\nu_{\boldsymbol{q}\mu\bar{\alpha}}\}$ $(\mu = 1, 2)$ are block matrices with size of $(N \times N)$ and $(2 \times N)$, respectively. Equation (D67) is expressed explicitly as:

$$\mathcal{E}_{\boldsymbol{q}\bar{\alpha}'}\eta_{\boldsymbol{q}\bar{\alpha}'\bar{\alpha}} + \sum_{\mu} z_{\boldsymbol{q}\bar{\alpha}'\mu}\nu_{\boldsymbol{q}\mu\bar{\alpha}} = \eta_{\boldsymbol{q}\bar{\alpha}'\bar{\alpha}}\mathcal{E}_{\boldsymbol{q}\bar{\alpha}}, \quad \text{(D69)}$$

and

$$\sum_{\bar{\alpha}'} z_{\boldsymbol{q}\bar{\alpha}'\mu}^{*}\eta_{\boldsymbol{q}\bar{\alpha}'\bar{\alpha}} + \sum_{\mu'} h_{\boldsymbol{q}\mu\mu'}^{(d)}\nu_{\boldsymbol{q}\mu'\bar{\alpha}} = \nu_{\boldsymbol{q}\mu\bar{\alpha}}\mathcal{E}_{\boldsymbol{q}\bar{\alpha}}. \quad \text{(D70)}$$

Equation (D69) is recast into

$$\eta_{\boldsymbol{q}\bar{\alpha}'\bar{\alpha}} = \left(\mathbb{P}\frac{1}{\mathcal{E}_{\boldsymbol{q}\bar{\alpha}} - \mathcal{E}_{\boldsymbol{q}\bar{\alpha}'}} + \Delta_{\boldsymbol{q}\bar{\alpha}}\delta_{\bar{\alpha}'\bar{\alpha}}\right)\sum_{\mu} z_{\boldsymbol{q}\bar{\alpha}'\mu}\nu_{\boldsymbol{q}\mu\bar{\alpha}}, \quad \text{(D71)}$$

where $\mathbb{P}[1/(\mathcal{E}_{\boldsymbol{q}\bar{\alpha}} - \mathcal{E}_{\boldsymbol{q}\bar{\alpha}'})]$ represents to take a Cauchy's principle value of $[1/(\mathcal{E}_{\boldsymbol{q}\bar{\alpha}} - \mathcal{E}_{\boldsymbol{q}\bar{\alpha}'})]$ and $\Delta_{\boldsymbol{q}\bar{\alpha}}$ is a constant to be determined later. Putting this expression back into Eq. (D70), one obtains

$$\sum_{\mu'} \left[h_{\boldsymbol{q}\mu\mu'}^{(d)} + \sigma_{\boldsymbol{q}\mu\mu'}(\mathcal{E}_{\boldsymbol{q}\bar{\alpha}})\right]\nu_{\boldsymbol{q}\mu'\bar{\alpha}} + \Delta_{\boldsymbol{q}\bar{\alpha}}z_{\boldsymbol{q}\bar{\alpha}\mu}^{*}\sum_{\mu'} z_{\boldsymbol{q}\bar{\alpha}\mu'}\nu_{\boldsymbol{q}\mu'\bar{\alpha}} = \nu_{\boldsymbol{q}\mu\bar{\alpha}}\mathcal{E}_{\boldsymbol{q}\bar{\alpha}}, \quad \text{(D72)}$$

where $\sigma_{\boldsymbol{q}\mu\mu'}(\mathcal{E}_{\boldsymbol{q}\bar{\alpha}})$ is given by

$$\sigma_{\boldsymbol{q}\mu\mu'}(\mathcal{E}_{\boldsymbol{q}\bar{\alpha}}) = \sum_{\bar{\alpha}'} \mathbb{P}\frac{z_{\boldsymbol{q}\bar{\alpha}'\mu}^{*}z_{\boldsymbol{q}\bar{\alpha}'\mu'}}{\mathcal{E}_{\boldsymbol{q}\bar{\alpha}} - \mathcal{E}_{\boldsymbol{q}\bar{\alpha}'}}. \quad \text{(D73)}$$

The matrix elements in square brackets of the first term of the left-hand side of Eq. (D72) is made diagonal in terms of a diagonalization matrix $A^{(r)}$ as follows:

$$\left[h_{\boldsymbol{q}}^{(d)} + \sigma_{\boldsymbol{q}}(\mathcal{E}_{\boldsymbol{q}\bar{\alpha}})\right]_{\mu\mu'} = \sum_{\mu''} A_{\mu'\mu''}^{(r)}\omega_{\boldsymbol{q}\mu''}A_{\mu''\mu}^{(r)\dagger}, \quad \text{(D74)}$$

with an eigenvalue as $\omega_{\boldsymbol{q}\mu}$. Thus, defining $\tilde{\nu}_{\boldsymbol{q}}$ and $\tilde{z}_{\boldsymbol{q}}$ as

$$\tilde{\nu}_{\boldsymbol{q}\mu\bar{\alpha}} = \sum_{\nu'} A_{\mu\mu'}^{(r)\dagger}\nu_{\boldsymbol{q}\mu'\bar{\alpha}}, \quad \text{(D75)}$$

and

$$\tilde{z}_{\boldsymbol{q}\bar{\alpha}\mu} = \sum_{\nu'} z_{\boldsymbol{q}\bar{\alpha}\mu'}A_{\mu'\mu}^{(r)}, \quad \text{(D76)}$$

Eq. (D72) becomes of the form:

$$\tilde{\nu}_{\boldsymbol{q}\mu\bar{\alpha}} = \Delta_{\boldsymbol{q}\bar{\alpha}}\frac{\tilde{z}_{\boldsymbol{q}\bar{\alpha}\mu}^{*}}{\mathcal{E}_{\boldsymbol{q}\bar{\alpha}} - \omega_{\boldsymbol{q}\mu}}\sum_{\mu'} \tilde{z}_{\boldsymbol{q}\bar{\alpha}\mu'}\tilde{\nu}_{\boldsymbol{q}\mu'\bar{\alpha}}, \quad \text{(D77)}$$

which determines $\Delta_{\boldsymbol{q}\bar{\alpha}}$ as

$$\Delta_{\boldsymbol{q}\bar{\alpha}}^{-1} = \sum_{\mu} \frac{|\tilde{z}_{\boldsymbol{q}\bar{\alpha}\mu}|^2}{\mathcal{E}_{\boldsymbol{q}\bar{\alpha}} - \omega_{\boldsymbol{q}\mu}}. \quad \text{(D78)}$$

According to commutation relations of Eqs. (D9) and (D11), one obtains the following relations:

$$\sum_{\bar{\alpha}} \tilde{\nu}_{\boldsymbol{q}\mu\bar{\alpha}}\tilde{\nu}_{\boldsymbol{q}\mu'\bar{\alpha}}^{*} = \delta_{\mu\mu'}, \quad \text{(D79)}$$

$$\sum_{\bar{\alpha}} \tilde{\nu}_{\boldsymbol{q}\mu\bar{\alpha}}\eta_{\boldsymbol{q}\bar{\alpha}'\bar{\alpha}}^{*} = 0, \quad \sum_{\bar{\alpha}} \eta_{\boldsymbol{q}\bar{\alpha}'\bar{\alpha}}\tilde{\nu}_{\boldsymbol{q}\mu\bar{\alpha}}^{*} = 0, \quad \text{(D80)}$$

and

$$\sum_{\bar{\alpha}''} \eta_{\boldsymbol{q}\bar{\alpha}\bar{\alpha}''}\eta_{\boldsymbol{q}\bar{\alpha}'\bar{\alpha}''}^{*} = \delta_{\bar{\alpha}\bar{\alpha}'}, \quad \text{(D81)}$$

where Eq. (D5) is used in view of Eq. (D13). Putting Eq. (D71) into the two equations of Eq. (D80), followed by subtracting the resulting equations side by side, one obtains

$$\sum_{\bar{\alpha}''} \tilde{\mathcal{Z}}_{\boldsymbol{q}\bar{\alpha}\bar{\alpha}''}\left(\mathbb{P}\frac{1}{\mathcal{E}_{\boldsymbol{q}\bar{\alpha}''} - \mathcal{E}_{\boldsymbol{q}\bar{\alpha}}} - \mathbb{P}\frac{1}{\mathcal{E}_{\boldsymbol{q}\bar{\alpha}''} - \mathcal{E}_{\boldsymbol{q}\bar{\alpha}'}}\right)\tilde{\mathcal{Z}}_{\boldsymbol{q}\bar{\alpha}''\bar{\alpha}'}^{\dagger} = \tilde{\mathcal{Z}}_{\boldsymbol{q}\bar{\alpha}\bar{\alpha}'}\Delta_{\boldsymbol{q}\bar{\alpha}'}\tilde{\mathcal{Z}}_{\boldsymbol{q}\bar{\alpha}'\bar{\alpha}'}^{\dagger} - \tilde{\mathcal{Z}}_{\boldsymbol{q}\bar{\alpha}\bar{\alpha}}\Delta_{\boldsymbol{q}\bar{\alpha}}\tilde{\mathcal{Z}}_{\boldsymbol{q}\bar{\alpha}\bar{\alpha}'}^{\dagger}, \quad \text{(D82)}$$

where

$$\tilde{\mathcal{Z}}_{\boldsymbol{q}\bar{\alpha}\bar{\alpha}'} = \sum_{\mu} \tilde{z}_{\boldsymbol{q}\bar{\alpha}\mu}\tilde{\nu}_{\boldsymbol{q}\mu\bar{\alpha}'}. \quad \text{(D83)}$$

Further, applying Eq. (D71) to Eq. (D81) again yields

$$\begin{aligned}\delta_{\bar{\alpha}\bar{\alpha}'} &= \sum_{\bar{\alpha}''} \tilde{\mathcal{Z}}_{\boldsymbol{q}\bar{\alpha}\bar{\alpha}''} \mathbb{P}\left(\frac{1}{\mathcal{E}_{\boldsymbol{q}\bar{\alpha}''}-\mathcal{E}_{\boldsymbol{q}\bar{\alpha}}}\frac{1}{\mathcal{E}_{\boldsymbol{q}\bar{\alpha}''}-\mathcal{E}_{\boldsymbol{q}\bar{\alpha}'}}\right)\tilde{\mathcal{Z}}^{\dagger}_{\boldsymbol{q}\bar{\alpha}''\bar{\alpha}'} \\ &\quad +\tilde{\mathcal{Z}}_{\boldsymbol{q}\bar{\alpha}\bar{\alpha}}\Delta_{\boldsymbol{q}\bar{\alpha}}\mathbb{P}\frac{1}{\mathcal{E}_{\boldsymbol{q}\bar{\alpha}}-\mathcal{E}_{\boldsymbol{q}\bar{\alpha}'}}\tilde{\mathcal{Z}}_{\boldsymbol{q}\bar{\alpha}\bar{\alpha}'} \\ &\quad -\tilde{\mathcal{Z}}_{\boldsymbol{q}\bar{\alpha}\bar{\alpha}'}\Delta_{\boldsymbol{q}\bar{\alpha}'}\mathbb{P}\frac{1}{\mathcal{E}_{\boldsymbol{q}\bar{\alpha}}-\mathcal{E}_{\boldsymbol{q}\bar{\alpha}'}}\tilde{\mathcal{Z}}_{\boldsymbol{q}\bar{\alpha}'\bar{\alpha}'} \\ &\quad +\delta_{\bar{\alpha}\bar{\alpha}'}\Delta^2_{\boldsymbol{q}\bar{\alpha}}|\tilde{\mathcal{Z}}_{\boldsymbol{q}\bar{\alpha}\bar{\alpha}}|^2 \\ &= \delta_{\bar{\alpha}\bar{\alpha}'}\left[(\pi\rho_{\boldsymbol{q}\bar{\alpha}})^2+\Delta^2_{\boldsymbol{q}\bar{\alpha}}\right]|\tilde{\mathcal{Z}}_{\boldsymbol{q}\bar{\alpha}\bar{\alpha}}|^2, \end{aligned} \tag{D84}$$

where in the first equality, Eq. (D83) is used, and in the second equality, Poincaré's theorem is applied, that is,

$$\begin{aligned} &\mathbb{P}\left(\frac{1}{\mathcal{E}_{\boldsymbol{q}\bar{\alpha}''}-\mathcal{E}_{\boldsymbol{q}\bar{\alpha}}}\frac{1}{\mathcal{E}_{\boldsymbol{q}\bar{\alpha}''}-\mathcal{E}_{\boldsymbol{q}\bar{\alpha}'}}\right) \\ &= \frac{1}{\mathcal{E}_{\boldsymbol{q}\bar{\alpha}}-\mathcal{E}_{\boldsymbol{q}\bar{\alpha}'}}\left(\mathbb{P}\frac{1}{\mathcal{E}_{\boldsymbol{q}\bar{\alpha}''}-\mathcal{E}_{\boldsymbol{q}\bar{\alpha}}}-\mathbb{P}\frac{1}{\mathcal{E}_{\boldsymbol{q}\bar{\alpha}''}-\mathcal{E}_{\boldsymbol{q}\bar{\alpha}'}}\right) \\ &+\pi^2\delta(\mathcal{E}_{\boldsymbol{q}\bar{\alpha}''}-\mathcal{E}_{\boldsymbol{q}\bar{\alpha}})\delta(\mathcal{E}_{\boldsymbol{q}\bar{\alpha}''}-\mathcal{E}_{\boldsymbol{q}\bar{\alpha}'}), \end{aligned} \tag{D85}$$

along with a density of state $\rho_{\boldsymbol{q}\bar{\alpha}}$ of state $\bar{\alpha}$, defined as

$$\rho_{\boldsymbol{q}\bar{\alpha}} = \frac{d\bar{\alpha}}{d\mathcal{E}_{\boldsymbol{q}\bar{\alpha}}}. \tag{D86}$$

Here, substituting $\mathcal{Z}_{\boldsymbol{q}\bar{\alpha}}$ for $\Delta_{\boldsymbol{q}\bar{\alpha}}\tilde{\mathcal{Z}}_{\boldsymbol{q}\bar{\alpha}\bar{\alpha}}$ just for the sake of simplicity, one obtains

$$\begin{aligned}\mathcal{Z}_{\boldsymbol{q}\bar{\alpha}} &= \Delta_{\boldsymbol{q}\bar{\alpha}}\tilde{\mathcal{Z}}_{\boldsymbol{q}\bar{\alpha}\bar{\alpha}} \\ &= \left[1+\left(\pi\rho_{\boldsymbol{q}\bar{\alpha}}\sum_{\mu}\frac{|\tilde{z}_{\boldsymbol{q}\bar{\alpha}\mu}|^2}{\mathcal{E}_{\boldsymbol{q}\bar{\alpha}}-\omega_{\boldsymbol{q}\mu}}\right)^2\right]^{-1/2}\end{aligned} \tag{D87}$$

from Eq. (D84) in view of Eq. (D78).

Thus, Eq. (D77) readily provides

$$\tilde{\nu}_{\boldsymbol{q}\mu\bar{\alpha}} = \frac{\tilde{z}^*_{\boldsymbol{q}\bar{\alpha}\mu}}{\mathcal{E}_{\boldsymbol{q}\bar{\alpha}}-\omega_{\boldsymbol{q}\mu}}\mathcal{Z}_{\boldsymbol{q}\bar{\alpha}}, \tag{D88}$$

and eventually, $\nu_{\boldsymbol{q}\mu\bar{\alpha}}$ is given by means of Eq. (D75). Further, putting Eq. (D88) into Eq. (D83) yields the expression of $\tilde{\mathcal{Z}}_{\boldsymbol{q}\bar{\alpha}\bar{\alpha}'}$. Accordingly, from Eq. (D71), $\eta_{\boldsymbol{q}\bar{\alpha}'\bar{\alpha}}$ is given by

$$\eta_{\boldsymbol{q}\bar{\alpha}'\bar{\alpha}} = \left[\sum_{\mu}\left(\mathbb{P}\frac{\tilde{z}_{\boldsymbol{q}\bar{\alpha}'\mu}\tilde{z}^*_{\boldsymbol{q}\bar{\alpha}\mu}}{\mathcal{E}_{\boldsymbol{q}\bar{\alpha}}-\mathcal{E}_{\boldsymbol{q}\bar{\alpha}'}}\frac{1}{\mathcal{E}_{\boldsymbol{q}\bar{\alpha}}-\omega_{\boldsymbol{q}\mu}}\right)+\delta_{\bar{\alpha}'\bar{\alpha}}\right]\mathcal{Z}_{\boldsymbol{q}\bar{\alpha}}. \tag{D89}$$

[4] U. Fano, Phys. Rev. **124**, 1866 (1961).

## APPENDIX E: DETAIL OF DERIVING AN EXPRESSION OF TOTAL RETARDED LONGITUDINAL-SUSCEPTIBILITY $\chi^{(t)}_{\boldsymbol{q}}(t,t')$

### 1. Derivation of a Retarded Susceptibility due to Electron-Induced Interaction $\chi_{\boldsymbol{q}}(t,t')$

The retarded susceptibility $\chi_{\boldsymbol{q}}(t,t')$ of Eq. (84) is read as

$$\begin{aligned} i\chi_{-\boldsymbol{q}}(t,t') &= \frac{4\pi}{V}\sum_{\alpha\alpha'\gamma\gamma'} N^{L*}_{\boldsymbol{q}\alpha}(t)\left\{R_{\boldsymbol{q}\alpha\gamma}(t,t_D)\right. \\ &\quad \left.\times T_{\boldsymbol{q}\gamma\gamma'}(t,t')\left[R_{\boldsymbol{q}}(t',t_D)\right]^{\dagger}_{\gamma'\alpha'}\right\} N^{L}_{\boldsymbol{q}\alpha'}(t'), \end{aligned} \tag{E1}$$

using Eq. (88), where one employs the explicit representation of $G^R_{\boldsymbol{q}\beta\beta'}(t,t')$ of Eq. (71)

$$\begin{aligned} &G^R_{\boldsymbol{q}\beta\beta'}(t,t') \\ &= -i\theta(t-t')e^{-i\Theta_{\boldsymbol{q}\beta}(t,t_D)}\sum_{\gamma\gamma'}V^{R\dagger}_{\boldsymbol{q}\beta\gamma}(t_D) \\ &\times T_{\boldsymbol{q}\gamma\gamma'}(t,t')V^{R}_{\boldsymbol{q}\gamma'\beta'}(t_D)e^{i\Theta^*_{\boldsymbol{q}\beta'}(t',t_D)}, \end{aligned} \tag{E2}$$

[see also Eq. (D41)], and further, $R_{\boldsymbol{q}\gamma\gamma'}(t,t_D)$ is defined as

$$R_{\boldsymbol{q}\gamma\gamma'}(t,t_D) = \sum_{\beta}\bar{V}^{R\dagger}_{\boldsymbol{q}\gamma\beta}(t)e^{-i\Theta_{\boldsymbol{q}\beta}(t)}V^{R\dagger}_{\boldsymbol{q}\beta\gamma'}(t_D). \tag{E3}$$

Hereafter, it is understood that $\Theta_{\boldsymbol{q}\beta}(t,t_D)$ given in Eq. (D27) is replaced by $\Theta_{\boldsymbol{q}\beta}(t)$, that is,

$$\Theta_{\boldsymbol{q}\beta}(t) = \Theta_{\boldsymbol{q}\beta}(t,t_D) \tag{E4}$$

just for the sake of simplicity.

Unfortunately, without approximation, it would be a formidable task to solve the non-hermitian Fano problem of Eq. (57), and hence to obtain $V^R_{\boldsymbol{q}}$ for evaluating Eq. (E3). Therefore, it would be preferable to substitute a hermitian Fano problem for Eq. (57) in an approximate manner. Actually, Eq. (D3) is solved; such an approximation would be verified within the criterion of the validity of the bosonization scheme developed in Sec. D 3. Hereafter, just for the sake of typographical simplicity, it is understood that a superscript "0" of $h^0_{\boldsymbol{q}}$, $N^0_{\boldsymbol{q}}$, $\Delta N^0_{\boldsymbol{q}}$, $E^0_{\boldsymbol{q}}$, and $\mathcal{E}^0_{\boldsymbol{q}}$ is omitted, and these notations are replaced by non-superscript counterparts of $h_{\boldsymbol{q}}$, $N_{\boldsymbol{q}}$, $\Delta N_{\boldsymbol{q}}$, $E_{\boldsymbol{q}}$, and $\mathcal{E}_{\boldsymbol{q}}$, respectively, as far as it is not likely to cause unnecessary confusion between them. Thus, Eq. (D3) is read as

$$h_{\boldsymbol{q}}V_{\boldsymbol{q}} = V_{\boldsymbol{q}}E_{\boldsymbol{q}}, \tag{E5}$$

where the hermitian matrix $h_{\boldsymbol{q}}$ is given by

$$h_{\boldsymbol{q}} = \begin{bmatrix}\mathcal{E}_{\boldsymbol{q}} & 0 & M_{\boldsymbol{q}} \\ 0 & \omega_{\boldsymbol{q}\alpha_1} & M_{\boldsymbol{q}\alpha_1} \\ M^{\dagger}_{\boldsymbol{q}} & M^*_{\boldsymbol{q}\alpha_1} & \omega_{\boldsymbol{q}\alpha_2}\end{bmatrix} \equiv \begin{bmatrix}\mathcal{E}_{\boldsymbol{q}} & z_{\boldsymbol{q}} \\ z^{\dagger}_{\boldsymbol{q}} & h^{(d)}_{\boldsymbol{q}}\end{bmatrix}. \tag{E6}$$

Recall the notations used right below Eq. (57), where $N$ and $N_0$ means the number of discretized continua and the number of independent solutions of Eq. (E5), respectively. Here, $\mathcal{E}_{\boldsymbol{q}} = \{\mathcal{E}_{\boldsymbol{q}\bar{\alpha}}\delta_{\bar{\alpha}\bar{\alpha}'}\}$ is a $(N \times N)$-diagonal matrix, $M_{\boldsymbol{q}} = \{M_{\boldsymbol{q}\bar{\alpha}}\}$ is a $(N \times 1)$-matrix, $\epsilon_{\boldsymbol{q}\alpha_1} \equiv \mathcal{E}_{\boldsymbol{q}\alpha_1}$, and $\epsilon_{\boldsymbol{q}\alpha_2} \equiv \omega_{\boldsymbol{q}}^{(LO)}$. Further, $z_{\boldsymbol{q}}$ is a $(N \times 2)$-matrix and $h_{\boldsymbol{q}}^{(d)}$ is a $(2 \times 2)$-matrix, given by

$$z_{\boldsymbol{q}} = \begin{bmatrix} 0 & M_{\boldsymbol{q}} \end{bmatrix} \tag{E7}$$

and

$$h_{\boldsymbol{q}}^{(d)} = \begin{bmatrix} \epsilon_{\boldsymbol{q}\alpha_1} & M_{\boldsymbol{q}\alpha_1} \\ M^*_{\boldsymbol{q}\alpha_1} & \epsilon_{\boldsymbol{q}\alpha_2} \end{bmatrix}, \tag{E8}$$

respectively. The Fano problem of concern is a scattering problem with a given energy $\mathcal{E}_{\boldsymbol{q}\bar{\alpha}}$ with one open-channel and two closed channels: $N_0 = N$; The set of solutions $\{V_{\boldsymbol{q}\gamma\beta}\}$ is provided in Sec. D 4.

Accordingly, substituting $V_{\boldsymbol{q}}$, $V_{\boldsymbol{q}}^\dagger$, and $N_{\boldsymbol{q}}$ for $V_{\boldsymbol{q}}^R$, $\bar{V}_{\boldsymbol{q}}^R$, and $N_{\boldsymbol{q}}^L$, respectively [see Eqs. (D13) and (D16)], Eq. (E3) becomes of the approximated form:

$$R_{\boldsymbol{q}\gamma\gamma'}(t,t_D) \approx \sum_\beta V_{\boldsymbol{q}\gamma\beta}(t)e^{-i\Theta_{\boldsymbol{q}\beta}(t)}V^\dagger_{\boldsymbol{q}\beta\gamma'}(t_D). \tag{E9}$$

In practical calculations, it is convenient to evaluate

$$\tilde{R}_{\boldsymbol{q}\gamma\gamma'}(t,t_D) = \sum_{\bar{\alpha}} \tilde{V}_{\boldsymbol{q}\gamma\bar{\alpha}}(t)e^{-i\Theta_{\boldsymbol{q}\bar{\alpha}}(t)}\tilde{V}^\dagger_{\boldsymbol{q}\bar{\alpha}\gamma'}(t_D), \tag{E10}$$

rather than $R_{\boldsymbol{q}}(t,t_D)$, where $\tilde{V}_{\boldsymbol{q}}(t)$ is defined as

$$\tilde{V}_{\boldsymbol{q}\gamma\bar{\alpha}}(t) = \sum_{\gamma'} \mathcal{A}^{(r)}_{\boldsymbol{q}\gamma\gamma'}(t)V_{\boldsymbol{q}\gamma'\bar{\alpha}}(t). \tag{E11}$$

Here, a $[(N+2)\times(N+2)]$-matrix $\mathcal{A}^{(r)}$ is introduced as:

$$\mathcal{A}^{(r)}_{\boldsymbol{q}} = \begin{bmatrix} 1 & 0 \\ 0 & A^{(r)}_{\boldsymbol{q}} \end{bmatrix}, \tag{E12}$$

where one of the two diagonal block matrices is a $[N\times N]$-unit block matrix with $\gamma$, $\gamma' = 1 \sim N$, and the other is a $(2 \times 2)$-block-matrix just equal to $A^{(r)}_{\boldsymbol{q}}$ relevant to $h^{(d)}_{\boldsymbol{q}}$ with $\gamma$, $\gamma' = (N+1) \sim (N+2)$; $A^{(r)}_{\boldsymbol{q}}$ is defined in Eq. (D74), indicating the degree of mixing between the two discrete levels, $\alpha_1$ and $\alpha_2$. The rest of off-diagonal block matrices is nothing but rectangular matrices with null components. Thus, Eq. (E9) is given by

$$R_{\boldsymbol{q}\gamma\gamma'}(t,t_D) = \sum_{\gamma''\gamma'''} \mathcal{A}^{(r)\dagger}_{\boldsymbol{q}\gamma\gamma''}(t)\tilde{R}_{\boldsymbol{q}\gamma''\gamma'''}(t,t_D) \times\mathcal{A}^{(r)}_{\boldsymbol{q}\gamma'''\gamma'}(t_D). \tag{E13}$$

According to Sec. E 4 showing the reduction of $\tilde{R}_{\boldsymbol{q}\gamma\gamma'}(t,t_D)$ to an explicit expression, Eq. (E13) with

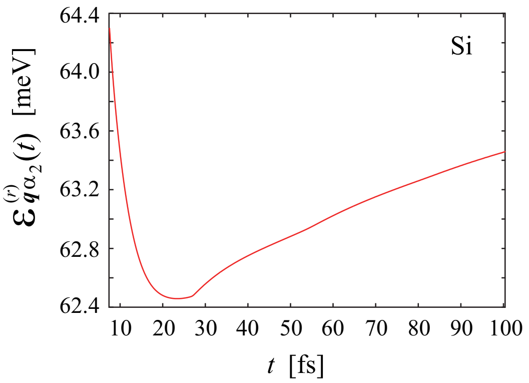


FIG. E-1: (Color Online) A trace of adiabatic energy $\mathcal{E}^{(r)}_{\boldsymbol{q}\alpha_2}(t)$ (in the unit of meV) as a function of time $t$ (in the unit of fs).

$\gamma = \alpha$ is cast into

$$\begin{aligned} &R_{\boldsymbol{q}\alpha\gamma'}(t,t_D) \\ &= \sum_{\bar{\alpha}} \mathcal{A}^{(r)\dagger}_{\boldsymbol{q}\alpha\bar{\alpha}}(t)\exp\left[-i\int_{t_D}^t \mathcal{E}_{\boldsymbol{q}\bar{\alpha}}(t'')dt''\right] \\ &\times e^{-\mathfrak{Z}_{\boldsymbol{q}\bar{\alpha}}(t,t_D)}\mathcal{A}^{(r)}_{\boldsymbol{q}\bar{\alpha}\gamma'}(t_D) \\ &+ \sum_{p=1,2} \mathcal{A}^{(r)\dagger}_{\boldsymbol{q}\alpha\alpha_p}(t)\exp\left[-i\int_{t_D}^t \mathcal{E}^{(r)}_{\boldsymbol{q}\alpha_p}(t'')dt''\right] \\ &\times\exp\left[-\int_{t_D}^t \frac{\Gamma_{\boldsymbol{q}\alpha_p}(t'')}{2}dt''\right]e^{-\mathfrak{Z}_{\boldsymbol{q}\bar{\alpha}_p}(t,t_D)} \\ &\times\mathcal{D}_{\boldsymbol{q}\alpha_p}(t,t_D)\mathcal{A}^{(r)}_{\boldsymbol{q}\alpha_p\gamma'}(t_D). \end{aligned} \tag{E14}$$

Here, $\mathcal{E}^{(r)}_{\boldsymbol{q}\alpha_p}$ represents resonance energy of state $\alpha_p$, given by

$$\mathcal{E}^{(r)}_{\boldsymbol{q}\alpha_p}(t) = \mathcal{E}_{\boldsymbol{q}\bar{\alpha}_p}(t), \tag{E15}$$

and $\Gamma_{\boldsymbol{q}\alpha_p}$ represents natural resonance width – full width at half maximum – of state $\alpha_p$, given by

$$\Gamma_{\boldsymbol{q}\alpha_p}(t) = 2\pi\rho_{\boldsymbol{q}\bar{\alpha}_p}(t)|\tilde{z}_{\boldsymbol{q}\bar{\alpha}_p\alpha_p}(t)|^2, \tag{E16}$$

where

$$\tilde{z}_{\boldsymbol{q}\bar{\alpha}\mu} = \sum_{\mu'} z_{\boldsymbol{q}\bar{\alpha}\mu'}A^{(r)}_{\boldsymbol{q}\mu'\mu} = M_{\boldsymbol{q}\bar{\alpha}}A^{(r)}_{\boldsymbol{q}2\mu}. \tag{E17}$$

Further, a new index $\bar{\alpha}_p$ is introduced, implying the index of continuum $\bar{\alpha}$ on the occasion that $\mathcal{E}_{\boldsymbol{q}\alpha_p}$ resonantly coincides with $\mathcal{E}_{\boldsymbol{q}\bar{\alpha}}$. By solving Eq. (D14), the adiabatic energy $\mathcal{E}^{(r)}_{\boldsymbol{q}\alpha_2}(t)$ of Si is obtained. The variance of this as a function of time is shown in Fig. E-1, where it is seen that the adiabatic energy changes within a couple of meV. The similar result is also obtained for GaAs, though not shown here.

In Eq. (E14), $\rho_{\boldsymbol{q}\bar{\alpha}_p}(t)$ represents a density of state of $\bar{\alpha}_p$ at time $t$, as defined in Eq. (D86). An approximate

expression of $\rho_{\boldsymbol{q}\bar{\alpha}_p}(t)$ is obtained in terms of Eq. (D17). It is noted that the contributions of the non-adiabatic correction incorporated in $\mathfrak{Z}_{\boldsymbol{q}\bar{\alpha}}(t, t_D)$, namely, $\mathfrak{I}_{\boldsymbol{q}\bar{\alpha}}(t, t_D)$, is a complex number in general [see the second term in the squared brackets of the right-hand side of Eq. (D19)], and this is approximately given by

$$\mathfrak{I}_{\boldsymbol{q}\bar{\alpha}}(t, t_D) \approx \sum_j \mathfrak{I}^{(j)}_{\boldsymbol{q}\bar{\alpha}\bar{\alpha}}\, \theta(t - t_j)\theta(t_j - t_D), \qquad \text{(E18)}$$

due to Eq. (D29). Especially, the imaginary part of it is represented as $\upsilon_{\boldsymbol{q}\bar{\alpha}}(t, t_D)$, that is,

$$\begin{aligned} \upsilon_{\boldsymbol{q}\bar{\alpha}}(t, t_D) &\equiv \mathrm{Im}\, \mathfrak{I}_{\boldsymbol{q}\bar{\alpha}\bar{\alpha}}(t, t_D) = \mathrm{Im}\, \mathfrak{Z}_{\boldsymbol{q}\bar{\alpha}}(t, t_D) \\ &= \sum_j \mathrm{Im}\mathfrak{I}^{(j)}_{\boldsymbol{q}\bar{\alpha}\bar{\alpha}}\, \theta(t - t_j)\theta(t_j - t_D), \end{aligned} \qquad \text{(E19)}$$

because this function plays a significant role of determining spectral profile due to transient FR, as shown in Sec. III. In addition, as regards $\mathfrak{Z}_{\boldsymbol{q}\bar{\alpha}_2}(t, t_D)$, $\gamma^{(0)}_{\boldsymbol{q}\bar{\alpha}_2}(t')$ is considered as negligibly small, that is,

$$\gamma^{(0)}_{\boldsymbol{q}\bar{\alpha}_2}(t') \approx 0, \qquad \text{(E20)}$$

since $V_{\boldsymbol{q}\alpha\bar{\alpha}_2} \approx 0$ because of $\alpha \neq \alpha_2$; a discrete-like FR-feature is mostly determined by the component $V_{\boldsymbol{q}\alpha_2\bar{\alpha}_2} \approx 1$ [see also Eq. (65), Eq. (66), and the definition of the index $\alpha$ given below Eq. (56)].

Moreover, in Eq.(E14), $\mathcal{D}_{\boldsymbol{q}\alpha_p}(t, t_D)$ is given by

$$\begin{aligned} &\mathcal{D}_{\boldsymbol{q}\alpha_p}(t, t_D) \\ &= \frac{\pi\rho^0_{\boldsymbol{q}\bar{\alpha}_p}}{\bar{\Gamma}_{\boldsymbol{q}\alpha_p}(t, t_D)/2} \left\{ \left[\Delta\Gamma_{\boldsymbol{q}\alpha_p}(t;t) - i\tilde{z}_{\boldsymbol{q}\bar{\alpha}_p\alpha_p}(t)\right] \right. \\ &\times \left[\Delta\Gamma_{\boldsymbol{q}\alpha_p}(t;t_D) + i\tilde{z}^*_{\boldsymbol{q}\bar{\alpha}_p\alpha_p}(t_D)\right] \\ &- \left[\Delta\Gamma_{\boldsymbol{q}\alpha_p}(t;t) - \pi\rho^0_{\boldsymbol{q}\bar{\alpha}_p}|\tilde{z}_{\boldsymbol{q}\bar{\alpha}_p\alpha_p}(t)|^2\right] \\ &\times \left[\Delta\Gamma_{\boldsymbol{q}\alpha_p}(t;t_D) - \pi\rho^0_{\boldsymbol{q}\bar{\alpha}_p}|\tilde{z}_{\boldsymbol{q}\bar{\alpha}_p\alpha_p}(t_D)|^2\right] \\ &\left. + (\pi\rho^0_{\boldsymbol{q}\bar{\alpha}_p})^2 |\tilde{z}_{\boldsymbol{q}\bar{\alpha}_p\alpha_p}(t)|^2 |\tilde{z}_{\boldsymbol{q}\bar{\alpha}_p\alpha_p}(t_D)|^2 \right\}, \end{aligned} \qquad \text{(E21)}$$

where

$$\begin{aligned} \Delta\Gamma_{\boldsymbol{q}\alpha_p}(t;t') &= \frac{1}{2}\bar{\Gamma}_{\boldsymbol{q}\alpha_p}(t, t_D) \\ &\quad -\pi\rho^0_{\boldsymbol{q}\bar{\alpha}_p}|\tilde{z}_{\boldsymbol{q}\bar{\alpha}_p\alpha_p}(t')|^2, \qquad \text{(E22)} \\ \bar{\Gamma}_{\boldsymbol{q}\alpha_p}(t, t_D) &= \frac{1}{2}\left[\Gamma_{\boldsymbol{q}\alpha_p}(t) + \Gamma_{\boldsymbol{q}\alpha_p}(t_D)\right], \qquad \text{(E23)} \end{aligned}$$

and $\rho^0_{\boldsymbol{q}\bar{\alpha}_p} = \rho_{\boldsymbol{q}\bar{\alpha}_p}(t_D)$ [see also Eqs. (E65) and (E71)]. It is remarked that the first and second terms of the right-hand side of Eq. (E14) imply the contributions from background continuum and a resonance state $\alpha_p$, respectively. Furthermore, it is seen that $\Delta\Gamma_{\boldsymbol{q}\alpha_p}(t_D; t_D) = 0$ at equal time, and thus, $\mathcal{D}_{\boldsymbol{q}\alpha_p}(t_D, t_D) = 1$ and $R_{\boldsymbol{q}\alpha\gamma}(t_D, t_D) = \delta_{\alpha\gamma}$, as it should be.

As illustrated in Sec. III, in particular, the function $\mathcal{D}_{\boldsymbol{q}\alpha_2}(t; t_D)$ plays a key role of determining spectral profiles of transient FR of concern. This function is a constituent marking $R_{\boldsymbol{q}\gamma\gamma'}(t, t_D)$, as shown in Eq. (E14). It is evident from Eq. (E9) that $R_{\boldsymbol{q}\gamma\gamma'}(t, t_D)$ is attached a meaning of time-evolution of PQ from state $\gamma'$ at $t_D$ to state $\gamma$ at $t$.

Because of the presence of the adiabatic energy phase in Eq. (E14), the following form of expression is contained in $i\chi_{-\boldsymbol{q}}$ of Eq. (E1):

$$\begin{aligned} S_{\alpha\alpha'}(t, t') &= \exp\left[-i\int_{t_D}^{t} \mathcal{E}_\alpha(t'')dt''\right] \\ &\times X_{\alpha\alpha'}(t, t') \exp\left[i\int_{t_D}^{t'} \mathcal{E}^*_{\alpha'}(t'')dt''\right], \end{aligned} \qquad \text{(E24)}$$

where $\mathcal{E}_\alpha(t)$ represents a complex energy, if necessary, with a negative imaginary part due to natural resonance width, and $X_{\alpha\alpha'}(t, t')$ is an arbitrary matrix element; specific forms of $\mathcal{E}_\alpha(t)$ and $X_{\alpha\alpha'}(t, t')$ will be given later in Eqs. (E31) and (E32). Letting $\tau$ equal $t - t' \geq 0$, namely, $\tau \equiv t - t'$, Eq. (E24) becomes

$$S_{\alpha\alpha'}(t, t') = e^{-i\mathcal{E}_{\alpha'}(t_D)\tau}\,\Xi_{\alpha\alpha'}(t' + \tau, t'), \qquad \text{(E25)}$$

where

$$\begin{aligned} &\Xi_{\alpha\alpha'}(t' + \tau, t') \\ &= X_{\alpha\alpha'}(t' + \tau, t') \\ &\times \exp\left\{-i\int_{t'}^{t'+\tau} \left[\mathcal{E}^*_{\alpha'}(t'') - \mathcal{E}_{\alpha'}(t_D)\right] dt''\right\} \\ &\times \exp\left\{-i\int_{t_D}^{t'+\tau} \left[\mathcal{E}_\alpha(t'') - \mathcal{E}^*_{\alpha'}(t'')\right] dt''\right\}. \end{aligned} \qquad \text{(E26)}$$

Here, $\Xi_{\alpha\alpha'}(t' + \tau, t')$ is approximated as

$$\Xi_{\alpha\alpha'}(t' + \tau, t') \approx \delta_{\alpha\alpha'}\Xi_\alpha(t' + \tau, t'), \qquad \text{(E27)}$$

where

$$\begin{aligned} &\Xi_\alpha(t' + \tau, t') \\ &= X_{\alpha\alpha}(t' + \tau, t') \\ &\times \exp\left\{-i\int_{t'}^{t'+\tau} \left[\mathcal{E}^*_\alpha(t'') - \mathcal{E}_\alpha(t_D)\right] dt''\right\} \\ &\times \exp\left\{-2\int_{t_D}^{t'+\tau} \mathrm{Im}\mathcal{E}_\alpha(t'')dt''\right\}. \end{aligned} \qquad \text{(E28)}$$

This approximation would be correct for relatively large $t$ satisfying the condition that

$$\left|\int_{t_D}^{t'+\tau} \mathrm{Re}\left[\mathcal{E}_\alpha(t'') - \mathcal{E}^*_{\alpha'}(t'')\right] dt''\right| \gg 2\pi, \qquad \text{(E29)}$$

since the last exponential function in the right-hand side of Eq. (E26) oscillates rapidly with the increase in $t$, and a dominant contribution arises just from $\mathrm{Re}\mathcal{E}_\alpha(t'') = \mathrm{Re}\mathcal{E}_{\alpha'}(t'')$.

Applying Eq. (E25) to Eq. (E1) in the light of Eq. (E14), Eq. (85) ends up with

$$\begin{aligned} & i\chi_{-\boldsymbol{q}}(t'+\tau,t') \\ &= \frac{4\pi}{V}\theta(\tau)\left[\sum_{\bar{\alpha}} e^{-i\mathcal{E}_{\boldsymbol{q}\bar{\alpha}}\tau}\Xi^{(c)}_{\boldsymbol{q}\bar{\alpha}}(t'+\tau,t')\right. \\ &\left. + \sum_{p=1,2} e^{-i[\mathcal{E}^{(r)}_{\boldsymbol{q}\alpha_p}-i\Gamma_{\boldsymbol{q}\alpha_p}/2]\tau}\Xi^{(r)}_{\boldsymbol{q}\bar{\alpha}_p}(t'+\tau,t')\right]. \end{aligned} \quad \text{(E30)}$$

Hereafter, it is understood that the argument of $t_D$ in $\mathcal{E}_{\boldsymbol{q}\bar{\alpha}}(t_D)$, $\mathcal{E}^{(r)}_{\boldsymbol{q}\alpha_p}(t_D)$, and $\Gamma_{\boldsymbol{q}\alpha_p}(t_D)$ is omitted just for the sake of simplicity, unless otherwise stated. Here, $\Xi^{(c)}_{\boldsymbol{q}\bar{\alpha}}(t'+\tau,t')$ and $\Xi^{(r)}_{\boldsymbol{q}\bar{\alpha}_p}(t'+\tau,t')$ correspond to Eq. (E28), where $X_{\alpha\alpha}(t'+\tau,t')$ is replaced by $X^{(c)}_{\boldsymbol{q}\bar{\alpha}\bar{\alpha}}(t'+\tau,t')$ and $X^{(r)}_{\boldsymbol{q}\alpha_p\alpha_p}(t'+\tau,t')$, respectively, and $\mathcal{E}_\alpha$ is replaced by $\mathcal{E}_{\boldsymbol{q}\bar{\alpha}}$ and $\mathcal{E}^{(r)}_{\boldsymbol{q}\alpha_p} - i\Gamma_{\boldsymbol{q}\alpha_p}/2$, respectively. $X^{(c)}_{\boldsymbol{q}\alpha\bar{\alpha}}(t'+\tau,t')$ and $X^{(r)}_{\boldsymbol{q}\alpha_p\alpha_p}(t'+\tau,t')$ are given by

$$\begin{aligned} & X^{(c)}_{\boldsymbol{q}\bar{\alpha}\bar{\alpha}}(t'+\tau,t') \\ &= N_{\boldsymbol{q}\bar{\alpha}}(t'+\tau)T_{\boldsymbol{q}\bar{\alpha}\bar{\alpha}}(t'+\tau,t')N_{\boldsymbol{q}\bar{\alpha}}(t') \\ &\times e^{-\mathfrak{Z}_{\boldsymbol{q}\bar{\alpha}}(t'+\tau,t')}e^{-2\mathrm{Re}\mathfrak{Z}_{\boldsymbol{q}\bar{\alpha}}(t',t_D)}, \end{aligned} \quad \text{(E31)}$$

and

$$\begin{aligned} & X^{(r)}_{\boldsymbol{q}\alpha_p\alpha_p}(t'+\tau,t') \\ &= \tilde{N}^{(r)}_{\boldsymbol{q}\alpha_p}(t'+\tau)\mathcal{D}_{\boldsymbol{q}\alpha_p}(t'+\tau,t_D)\tilde{T}^{(r)}_{\boldsymbol{q}\alpha_p\alpha_p}(t'+\tau,t') \\ &\times \mathcal{D}^*_{\boldsymbol{q}\alpha_p}(t',t_D)\tilde{N}^{(r)\dagger}_{\boldsymbol{q}\alpha_p}(t')e^{-\mathfrak{Z}_{\boldsymbol{q}\bar{\alpha}_p}(t'+\tau,t')} \\ &\times e^{-2\mathrm{Re}\mathfrak{Z}_{\boldsymbol{q}\bar{\alpha}_p}(t',t_D)}, \end{aligned} \quad \text{(E32)}$$

where

$$\tilde{N}^{(r)}_{\boldsymbol{q}\alpha_p}(t) = [N_{\boldsymbol{q}}(t)\mathcal{A}^{(r)\dagger}_{\boldsymbol{q}}(t)]_{\alpha_p}, \quad \text{(E33)}$$

and

$$\tilde{T}^{(r)}_{\boldsymbol{q}} = \mathcal{A}^{(r)}_{\boldsymbol{q}}(t_D)T_{\boldsymbol{q}}\mathcal{A}^{(r)\dagger}_{\boldsymbol{q}}(t_D). \quad \text{(E34)}$$

It is noted that in the first term in the squared brackets of the right-hand side of Eq. (E30), the summation over $\bar{\alpha}$ includes not only terms with positive energy $\mathcal{E}_{\boldsymbol{q}\bar{\alpha}} = \mathcal{E}_{\boldsymbol{q}\bar{\alpha}_+} > 0$, but also terms with negative energy$\mathcal{E}_{\boldsymbol{q}\bar{\alpha}} = \mathcal{E}_{\boldsymbol{q}\bar{\alpha}_-} < 0$, where according to Eq. (C69), $\mathcal{E}_{\boldsymbol{q}\bar{\alpha}_+} = -\mathcal{E}_{\boldsymbol{q}\bar{\alpha}_-}$.

### 2. Derivation of a Retarded Susceptibility due to LO-Phonon-Induced Interaction $\chi'_{\boldsymbol{q}}(t,t')$

On the other hand, the retarded susceptibility of $\chi'_{\boldsymbol{q}}(t'+\tau,t')$ introduced in Eq. (79) is expressed as

$$\chi'_{\boldsymbol{q}}(t'+\tau,t') = \frac{4\pi}{V}|g'_{\boldsymbol{q}}|^2 D'^R_{\boldsymbol{q}}(t'+\tau,t'), \quad \text{(E35)}$$

where

$$|g'_{\boldsymbol{q}}|^2 = \left|\frac{g^0_{\boldsymbol{q}}}{v^{(C)}_{\boldsymbol{q}}}\right|^2 \quad \text{(E36)}$$

with $g^0_{\boldsymbol{q}}$ defined in Eq. (44), and

$$v^{(C)}_{\boldsymbol{q}} = \epsilon_\infty V^{(C)}_{\boldsymbol{q}} = \frac{4\pi}{V}\frac{1}{\boldsymbol{q}^2} \quad \text{(E37)}$$

with $\epsilon_\infty$ as a background dielectric constant given in Eq. (3). Further, $D'^R_{\boldsymbol{q}}(t,t')$ is a retarded phonon Green function given by[5]

$$\begin{aligned} & D'^R_{\boldsymbol{q}}(t,t') \\ &= -i\Big\langle\Big[c_{\boldsymbol{q}}(t) + c^\dagger_{-\boldsymbol{q}}(t), c_{-\boldsymbol{q}}(t') + c^\dagger_{\boldsymbol{q}}(t')\Big]\Big\rangle\theta(t-t') \\ &= -i\Big\langle\Big[c_{\boldsymbol{q}}(t), c^\dagger_{\boldsymbol{q}}(t')\Big] - \Big[c_{-\boldsymbol{q}}(t), c^\dagger_{-\boldsymbol{q}}(t')\Big]^\dagger\Big\rangle\theta(t-t') \\ &\equiv \bar{D}'^R_{\boldsymbol{q}}(t,t') + \big[\bar{D}'^R_{-\boldsymbol{q}}(t,t')\big]^*, \end{aligned} \quad \text{(E38)}$$

where

$$D'^R_{-\boldsymbol{q}}(t,t') = \big[D'^R_{\boldsymbol{q}}(t,t')\big]^*, \quad \text{(E39)}$$

and

$$\bar{D}'^R_{\boldsymbol{q}}(t,t') = -i\Big\langle\big[c_{\boldsymbol{q}}(t), c^\dagger_{\boldsymbol{q}}(t')\big]\Big\rangle\theta(t-t'). \quad \text{(E40)}$$

It is remarked that in the small-$\boldsymbol{q}$ limit, because of Eq. (E36), $\chi'_{\boldsymbol{q}}(t'+\tau,t') \propto |\boldsymbol{q}|^2$ for the Fröhlich interaction, while $\chi'_{\boldsymbol{q}}(t'+\tau,t') \propto |\boldsymbol{q}|^4$ for the deformation potential interaction.

Employing Eqs. (58), (61), and (D39), Eq.(E40) is recast into

$$\begin{aligned} & i\bar{D}'^R_{\boldsymbol{q}}(t,t') \\ &= \sum_{\beta\beta'} V_{\boldsymbol{q}\alpha_2\beta}(t)\Big\langle\Big[F_{\boldsymbol{q}\beta}(t), F^\dagger_{\boldsymbol{q}\beta'}(t')\Big]\Big\rangle V^\dagger_{\boldsymbol{q}\beta'\alpha_2}(t'), \\ &= i\sum_{\beta\beta'} V_{\boldsymbol{q}\alpha_2\beta}(t)G^R_{\boldsymbol{q}\beta\beta'}(t,t')V^\dagger_{\boldsymbol{q}\beta'\alpha_2}(t') \\ &= \sum_{\gamma\gamma'} R_{\boldsymbol{q}\alpha_2\gamma}(t,t_D)T_{\boldsymbol{q}\gamma\gamma'}(t,t')\left[R_{\boldsymbol{q}}(t',t_D)\right]^\dagger_{\gamma'\alpha_2}, \end{aligned} \quad \text{(E41)}$$

where in the third equality, Eqs. (D41) and (E9) are used. Similarly to Eq. (E14), $R_{\boldsymbol{q}\alpha_2\gamma}(t,t_D)$ is provided as

$$\begin{aligned} & R_{\boldsymbol{q}\alpha_2\gamma}(t,t_D) \\ &= \sum_{p=1,2}\mathcal{A}^{(r)\dagger}_{\boldsymbol{q}\alpha_2\alpha_p}(t)\exp\left[-i\int_{t_D}^t \mathcal{E}^{(r)}_{\boldsymbol{q}\alpha_p}(t'')dt''\right] \\ &\times\exp\left[-\int_{t_D}^t \frac{\Gamma_{\boldsymbol{q}\alpha_p}(t'')}{2}dt''\right]e^{-\mathfrak{Z}_{\boldsymbol{q}\bar{\alpha}_p}(t,t_D)}, \\ &\times\mathcal{D}_{\boldsymbol{q}\alpha_p}(t,t_D)\mathcal{A}^{(r)}_{\boldsymbol{q}\alpha_p\gamma}(t_D). \end{aligned} \quad \text{(E42)}$$

Thus, $\chi'_{\boldsymbol{q}}(t'+\tau,t')$ of Eq. (E35) becomes

$$\begin{aligned} & i\chi'_{\boldsymbol{q}}(t'+\tau,t') \\ &= \frac{4\pi}{V}\sum_{p=1,2}\Big\{e^{-i[\mathcal{E}^{(r)}_{\boldsymbol{q}\alpha_p}-i\Gamma_{\boldsymbol{q}\alpha_p}/2]\tau}\Pi^{(r)}_{\boldsymbol{q}\alpha_p}(t'+\tau,t') \\ &- e^{i[\mathcal{E}^{(r)}_{-\boldsymbol{q}\alpha_p}+i\Gamma_{-\boldsymbol{q}\alpha_p}/2]\tau}\Pi^{(r)*}_{-\boldsymbol{q}\alpha_p}(t'+\tau,t')\Big\}, \end{aligned} \quad \text{(E43)}$$

where $\Pi^{(r)}_{\boldsymbol{q}\alpha_p}$ is defined as

$$\Pi^{(r)}_{\boldsymbol{q}\alpha_p}(t'+\tau,t') = P^{(r)}_{\boldsymbol{q}\alpha_p\alpha_p}(t'+\tau,t') \times\exp\left\{-i\int_{t'}^{t'+\tau}\left[\mathcal{E}^*_{\boldsymbol{q}\bar{\alpha}_p}(t'')-\mathcal{E}^{(r)}_{\boldsymbol{q}\alpha_p}\right]dt''\right\} \times\exp\left\{\int_{t_D}^{t'+\tau}\Gamma_{\boldsymbol{q}\bar{\alpha}_p}(t'')dt''\right\}, \quad (E44)$$

and

$$P^{(r)}_{\boldsymbol{q}\alpha_p\alpha_p}(t'+\tau,t') = \left|g'_{\boldsymbol{q}}\right|^2 A^{(r)\dagger}_{\boldsymbol{q}\alpha_2\alpha_p}(t'+\tau)\mathcal{D}_{\boldsymbol{q}\alpha_p}(t'+\tau,t_D) \times\tilde{T}^{(r)}_{\boldsymbol{q}\alpha_p\alpha_p}(t'+\tau,t')\mathcal{D}^*_{\boldsymbol{q}\alpha_p}(t',t_D)A^{(r)}_{\boldsymbol{q}\alpha_p\alpha_2}(t') \times e^{-\mathfrak{Z}_{\boldsymbol{q}\bar{\alpha}_p}(t'+\tau,t')}e^{-2\mathrm{Re}\mathfrak{Z}_{\boldsymbol{q}\bar{\alpha}_p}(t',t_D)}. \quad (E45)$$

### 3. Expression of $\chi^{(t)}_{\boldsymbol{q}}(t'+\tau,t')$

According to Eqs. (E30) and (E43), the total retarded susceptibility $\chi^{(t)}_{\boldsymbol{q}}(t'+\tau,t')$ of Eq. (79) is given by

$$-i\chi^{(t)}_{\boldsymbol{q}}(t'+\tau,t') = \frac{4\pi}{V}\left\{\sum_{\bar{\alpha}=\bar{\alpha}_\pm} e^{i\mathcal{E}_{\boldsymbol{q}\bar{\alpha}}\tau}\Xi^{(c)*}_{\boldsymbol{q}\bar{\alpha}}(t'+\tau,t') + \sum_{p=1,2} e^{i[\mathcal{E}^{(r)}_{\boldsymbol{q}\alpha_p}+i\Gamma_{\boldsymbol{q}\alpha_p}/2]\tau} \times\left[\Xi^{(r)*}_{\boldsymbol{q}\alpha_p}(t'+\tau,t')+\Pi^{(r)*}_{\boldsymbol{q}\alpha_p}(t'+\tau,t')\right] - \sum_{p=1,2} e^{-i[\mathcal{E}^{(r)}_{\boldsymbol{q}\alpha_p}-i\Gamma_{\boldsymbol{q}\alpha_p}/2]\tau}\Pi^{(r)}_{\boldsymbol{q}\alpha_p}(t'+\tau,t')\right\}. \quad (E46)$$

Here, the following relations are taken into account as: $\mathcal{E}_{\boldsymbol{q}\bar{\alpha}}=\mathcal{E}_{-\boldsymbol{q}\bar{\alpha}}$, $\mathcal{E}^{(r)}_{\boldsymbol{q}\alpha_p}=\mathcal{E}^{(r)}_{-\boldsymbol{q}\alpha_p}$, $\Gamma_{\boldsymbol{q}\alpha_p}=\Gamma_{-\boldsymbol{q}\alpha_p}$, and $\Xi^{(r)}_{\boldsymbol{q}\alpha_p}(t'+\tau,t')=\Xi^{(r)}_{-\boldsymbol{q}\alpha_p}(t'+\tau,t')$, which are readily verified by consulting Appendix C within the framework of the bosonization scheme given in Sec. D 3 and the small-$\boldsymbol{q}$ limit.

### 4. Calculation of $\tilde{R}_{\boldsymbol{q}\gamma\gamma'}(t,t_D)$ of Eq. (E10)

Here, $\tilde{R}_{\boldsymbol{q}\gamma\gamma'}(t,t_D)$, given by

$$\tilde{R}_{\boldsymbol{q}\gamma\gamma'}(t,t_D) = \sum_{\bar{\alpha}}\tilde{V}_{\boldsymbol{q}\gamma\bar{\alpha}}(t)e^{-i\Theta_{\boldsymbol{q}\bar{\alpha}}(t)}\tilde{V}^\dagger_{\boldsymbol{q}\bar{\alpha}\gamma'}(t_D), \quad (E47)$$

is calculated, where $\tilde{V}_{\boldsymbol{q}\gamma\bar{\alpha}}(t)$ is provided by

$$\tilde{V}_{\boldsymbol{q}}(t)=\begin{bmatrix}\eta_{\boldsymbol{q}}(t)\\ \tilde{\nu}_{\boldsymbol{q}}(t)\end{bmatrix}, \quad (E48)$$

with $\eta_{\boldsymbol{q}}(t)=\{\eta_{\boldsymbol{q}\bar{\alpha}'\bar{\alpha}}(t)\}$ and $\tilde{\nu}_{\boldsymbol{q}}(t)=\{\tilde{\nu}_{\boldsymbol{q}\alpha'_p\bar{\alpha}}(t)\}$. These matrix components of $\eta_{\boldsymbol{q}\bar{\alpha}'\bar{\alpha}}(t)$ and $\tilde{\nu}_{\boldsymbol{q}\alpha'_p\bar{\alpha}}(t)$ are given in Eqs.(D89) and (D88), respectively. Thus, Eq. (E47) is divided into the following four cases:

$$\tilde{R}_{\boldsymbol{q}\alpha_p\alpha_{p'}}(t,t_D) = \sum_{\bar{\alpha}}\tilde{\nu}_{\boldsymbol{q}\alpha_p\bar{\alpha}}(t)e^{-i\Theta_{\boldsymbol{q}\bar{\alpha}}(t)}\tilde{\nu}^*_{\boldsymbol{q}\alpha_{p'}\bar{\alpha}}(t_D), \quad (E49)$$

$$\tilde{R}_{\boldsymbol{q}\alpha_p\bar{\alpha}'}(t,t_D) = \sum_{\bar{\alpha}}\tilde{\nu}_{\boldsymbol{q}\alpha_p\bar{\alpha}}(t)e^{-i\Theta_{\boldsymbol{q}\bar{\alpha}}(t)}\eta^*_{\boldsymbol{q}\bar{\alpha}'\bar{\alpha}}(t_D), \quad (E50)$$

$$\tilde{R}_{\boldsymbol{q}\bar{\alpha}'\alpha_p}(t,t_D) = \sum_{\bar{\alpha}}\eta_{\boldsymbol{q}\bar{\alpha}'\bar{\alpha}}(t)e^{-i\Theta_{\boldsymbol{q}\bar{\alpha}}(t)}\tilde{\nu}^*_{\boldsymbol{q}\alpha_p\bar{\alpha}}(t_D), \quad (E51)$$

and

$$\tilde{R}_{\boldsymbol{q}\bar{\alpha}'\bar{\alpha}''}(t,t_D) = \sum_{\bar{\alpha}}\eta_{\boldsymbol{q}\bar{\alpha}'\bar{\alpha}}(t)e^{-i\Theta_{\boldsymbol{q}\bar{\alpha}}(t)}\eta^*_{\boldsymbol{q}\bar{\alpha}''\bar{\alpha}}(t_D), \quad (E52)$$

where time-dependence of every term is explicitly indicated, and $\alpha_p,\alpha_{p'}=\alpha_1,\alpha_2$.

All of the expressions of $\tilde{R}_{\boldsymbol{q}\gamma\gamma'}(t,t_D)$ given above include a common factor of $\mathcal{Z}_{\boldsymbol{q}\bar{\alpha}}(t)\mathcal{Z}^*_{\boldsymbol{q}\bar{\alpha}}(t_D)$. According to Eq. (D87), $[\mathcal{Z}_{\boldsymbol{q}\bar{\alpha}}(t)]^{-2}$ is cast into

$$[\mathcal{Z}_{\boldsymbol{q}\bar{\alpha}}(t)]^{-2} = \{[\mathcal{E}_{\boldsymbol{q}\bar{\alpha}}(t)-\omega_{\boldsymbol{q}\alpha_1}(t)][\mathcal{E}_{\boldsymbol{q}\bar{\alpha}}(t)-\omega_{\boldsymbol{q}\alpha_2}(t)]\}^{-2} \times L_{\boldsymbol{q}\bar{\alpha}}(t), \quad (E53)$$

where

$$L_{\boldsymbol{q}\bar{\alpha}}(t) = \{[\mathcal{E}_{\boldsymbol{q}\bar{\alpha}}(t)-\omega_{\boldsymbol{q}\alpha_1}(t)][\mathcal{E}_{\boldsymbol{q}\bar{\alpha}}(t)-\omega_{\boldsymbol{q}\alpha_2}(t)]\}^2 +[\gamma_{\boldsymbol{q}\bar{\alpha}\alpha_2}(t)/2]^2[\mathcal{E}_{\boldsymbol{q}\bar{\alpha}}(t)-\omega_{\boldsymbol{q}\alpha_1}(t)]^2 +[\gamma_{\boldsymbol{q}\bar{\alpha}\alpha_1}(t)/2]^2[\mathcal{E}_{\boldsymbol{q}\bar{\alpha}}(t)-\omega_{\boldsymbol{q}\alpha_2}(t)]^2 +2[\gamma_{\boldsymbol{q}\bar{\alpha}\alpha_1}(t)/2]^2[\gamma_{\boldsymbol{q}\bar{\alpha}\alpha_2}(t)/2]^2 \times[\mathcal{E}_{\boldsymbol{q}\bar{\alpha}}(t)-\omega_{\boldsymbol{q}\alpha_1}(t)]^2[\mathcal{E}_{\boldsymbol{q}\bar{\alpha}}(t)-\omega_{\boldsymbol{q}\alpha_2}(t)], \quad (E54)$$

with

$$\gamma_{\boldsymbol{q}\bar{\alpha}\alpha_p}(t)=2\pi\rho_{\boldsymbol{q}\bar{\alpha}}(t)|\tilde{z}_{\boldsymbol{q}\bar{\alpha}\alpha_p}(t)|^2 \quad (E55)$$

[for $\rho_{\boldsymbol{q}\bar{\alpha}}(t)$, see Eq. (D86)]. Obviously, there are four solutions, given by $\mathcal{E}_{\boldsymbol{q}\bar{\alpha}}(t)=\mathcal{E}^{(\pm)}_{\boldsymbol{q}\bar{\alpha}_p}(t)$, ensuring an algebraic equation of $L_{\boldsymbol{q}\bar{\alpha}}(t)=0$ with $p=1,2$. By assuming an order of $[\gamma_{\boldsymbol{q}\bar{\alpha}\alpha_p}(t)/2]/[\omega_{\boldsymbol{q}\alpha_{p'}}(t)-\omega_{\boldsymbol{q}\alpha_p}(t)]$ for $p\neq p'$ to be negligibly small, that is,

$$\frac{\gamma_{\boldsymbol{q}\bar{\alpha}\alpha_p}(t)/2}{|\omega_{\boldsymbol{q}\alpha_{p'}}(t)-\omega_{\boldsymbol{q}\alpha_p}(t)|}\approx\frac{\Gamma_{\boldsymbol{q}\alpha_p}(t)/2}{|\omega_{\boldsymbol{q}\alpha_{p'}}(t)-\omega_{\boldsymbol{q}\alpha_p}(t)|}\ll 1, \quad (E56)$$

the solutions of $\mathcal{E}^{(\pm)}_{\boldsymbol{q}\bar{\alpha}_p}(t)$ are approximately provided as

$$\begin{aligned}\mathcal{E}^{(\pm)}_{\boldsymbol{q}\bar{\alpha}_p}(t) &\approx \omega_{\boldsymbol{q}\alpha_p}(t) \pm i\gamma_{\boldsymbol{q}\bar{\alpha}\alpha_p}(t)/2 \\ &\approx \omega_{\boldsymbol{q}\alpha_p}(t) \pm i\Gamma_{\boldsymbol{q}\alpha_p}(t)/2. \qquad \text{(E57)}\end{aligned}$$

Here, in both of the first equality of Eq. (E56) and the second equality of Eq. (E57), $\gamma_{\boldsymbol{q}\bar{\alpha}\alpha_p}(t)$ is evaluated in the vicinity of $\mathcal{E}_{\boldsymbol{q}\bar{\alpha}}(t) \approx \omega_{\boldsymbol{q}\alpha_p}(t)$, which would cause dominant contribution to $\gamma_{\boldsymbol{q}\bar{\alpha}\alpha_p}(t)$. Hence, $\Gamma_{\boldsymbol{q}\alpha_p}(t)$ is substituted for $\gamma_{\boldsymbol{q}\bar{\alpha}\alpha_p}(t)$, that is,

$$\Gamma_{\boldsymbol{q}\alpha_p}(t) = 2\pi\rho_{\boldsymbol{q}\bar{\alpha}_p}(t)|\tilde{z}_{\bar{\alpha}_p\alpha_p}(t)|^2, \qquad \text{(E58)}$$

where a new index $\bar{\alpha}_p$ is introduced, implying the index of continuum $\bar{\alpha}$ on the occasion that $\mathcal{E}_{\boldsymbol{q}\alpha_p}$ resonantly coincides with $\mathcal{E}_{\boldsymbol{q}\bar{\alpha}}$. Therefore, Eq. (E54) is recast into

$$\begin{aligned}L_{\boldsymbol{q}\bar{\alpha}}(t) &\approx \prod_{p=1,2}\left[\mathcal{E}_{\boldsymbol{q}\bar{\alpha}}(t) - \mathcal{E}^{(+)}_{\boldsymbol{q}\bar{\alpha}_p}(t)\right] \\ &\quad \times \left[\mathcal{E}_{\boldsymbol{q}\bar{\alpha}}(t) - \mathcal{E}^{(-)}_{\boldsymbol{q}\bar{\alpha}_p}(t)\right]. \qquad \text{(E59)}\end{aligned}$$

Thus, in terms of $L^0_{\boldsymbol{q}\bar{\alpha}}(t)$ defined as

$$L^0_{\boldsymbol{q}\bar{\alpha}}(t) = \prod_{p=1,2}\left[\mathcal{E}_{\boldsymbol{q}\bar{\alpha}}(t) - \omega_{\boldsymbol{q}\alpha_p}(t)\right], \qquad \text{(E60)}$$

$\mathcal{Z}_{\boldsymbol{q}\bar{\alpha}}(t)\mathcal{Z}^*_{\boldsymbol{q}\bar{\alpha}}(t_D)$ becomes

$$\mathcal{Z}_{\boldsymbol{q}\bar{\alpha}}(t)\mathcal{Z}^*_{\boldsymbol{q}\bar{\alpha}}(t_D) = \frac{L^0_{\boldsymbol{q}\bar{\alpha}}(t)L^0_{\boldsymbol{q}\bar{\alpha}}(t_D)}{\left[L_{\boldsymbol{q}\bar{\alpha}}(t)L_{\boldsymbol{q}\bar{\alpha}}(t_D)\right]^{1/2}}. \qquad \text{(E61)}$$

The factor of $L_{\boldsymbol{q}\bar{\alpha}}(t)L_{\boldsymbol{q}\bar{\alpha}}(t_D)$ in the denominator of the above equation is rewritten as products of a term

$$\mathcal{L}^{(p,\pm)}_{\boldsymbol{q}\bar{\alpha}}(t,t_D) = \left[\mathcal{E}_{\boldsymbol{q}\bar{\alpha}}(t) - \mathcal{E}^{(\pm)}_{\boldsymbol{q}\bar{\alpha}_p}(t)\right]\left[\mathcal{E}_{\boldsymbol{q}\bar{\alpha}}(t_D) - \mathcal{E}^{(\pm)}_{\boldsymbol{q}\bar{\alpha}_p}(t_D)\right], \qquad \text{(E62)}$$

that is,

$$L_{\boldsymbol{q}\bar{\alpha}}(t)L_{\boldsymbol{q}\bar{\alpha}}(t_D) = \prod_{p,\sigma=\pm}\mathcal{L}^{(p,\sigma)}_{\boldsymbol{q}\bar{\alpha}}(t,t_D), \qquad \text{(E63)}$$

where a plus or minus sign corresponds in Eq. (E62). Actually, $\mathcal{L}^{(p,\pm)}_{\boldsymbol{q}\bar{\alpha}}(t,t_D)$ is reduced to the approximate form:

$$\begin{aligned}&\mathcal{L}^{(p,\pm)}_{\boldsymbol{q}\bar{\alpha}}(t,t_D) \\ &\approx \left\{\mathcal{E}_{\boldsymbol{q}\bar{\alpha}}(t_D) - \omega_{\boldsymbol{q}\alpha_p}(t_D) \mp \frac{i}{2}\bar{\Gamma}_{\boldsymbol{q}\alpha_p}(t,t_D)\right\}^2, \qquad \text{(E64)}\end{aligned}$$

and

$$\bar{\Gamma}_{\boldsymbol{q}\alpha_p}(t,t_D) = \frac{1}{2}\left[\Gamma_{\boldsymbol{q}\alpha_p}(t) + \Gamma_{\boldsymbol{q}\alpha_p}(t_D)\right]. \qquad \text{(E65)}$$

In deriving Eqs. (E63) and (E64), the approximations of

$$\mathcal{E}_{\boldsymbol{q}\bar{\alpha}}(t) - \omega_{\boldsymbol{q}\alpha_p}(t) \approx \mathcal{E}_{\boldsymbol{q}\bar{\alpha}}(t_D) - \omega_{\boldsymbol{q}\alpha_p}(t_D), \qquad \text{(E66)}$$

and

$$\Gamma_{\boldsymbol{q}\alpha_p}(t) \approx \Gamma_{\boldsymbol{q}\alpha_p}(t_D) \qquad \text{(E67)}$$

are partially made, respectively. It is remarked that these approximations would be ensured on the occasion of $\mathcal{E}_{\boldsymbol{q}\bar{\alpha}} \approx \omega_{\boldsymbol{q}\alpha_p}$, namely, in the resonant condition of $\bar{\alpha} \approx \bar{\alpha}_p$. Given Eq. (E64), the denominator of Eq. (E61) becomes

$$\begin{aligned}\left[L_{\boldsymbol{q}\bar{\alpha}}(t)L_{\boldsymbol{q}\bar{\alpha}}(t_D)\right]^{1/2} &= \prod_p\Big\{\left[\mathcal{E}_{\boldsymbol{q}\bar{\alpha}}(t_D) - \omega_{\boldsymbol{q}\alpha_p}(t_D)\right]^2 \\ &\quad + \left[\bar{\Gamma}_{\boldsymbol{q}\alpha_p}(t,t_D)/2\right]^2\Big\}. \qquad \text{(E68)}\end{aligned}$$

This implies that an integrand of $\tilde{R}_{\boldsymbol{q}\gamma\gamma'}(t,t_D)$ in Eqs. (E49)-(E52) as a function of $\mathcal{E}_{\boldsymbol{q}\bar{\alpha}}(t_D)$ has two first-order poles at

$$\mathcal{E}_{\boldsymbol{q}\bar{\alpha}}(t_D) = \omega_{\boldsymbol{q}\alpha_p}(t_D) - \frac{i}{2}\bar{\Gamma}_{\boldsymbol{q}\alpha_p}(t,t_D) \qquad \text{(E69)}$$

in the lower-half complex-$\mathcal{E}_{\boldsymbol{q}\bar{\alpha}}(t_D)$-plane with $p = 1,2$.

To begin with an evaluation of Eq. (E49), by using Eq. (D88), $\tilde{R}_{\boldsymbol{q}\alpha_p\alpha_{p'}}(t,t_D)$ is rewritten as

$$\begin{aligned}&\tilde{R}_{\boldsymbol{q}\alpha_p\alpha_{p'}}(t,t_D) \\ &= \sum_{\bar{\alpha}}\frac{\tilde{z}^*_{\boldsymbol{q}\bar{\alpha}\alpha_p}(t)\tilde{z}_{\boldsymbol{q}\bar{\alpha}\alpha_{p'}}(t_D)e^{-i\Theta_{\boldsymbol{q}\bar{\alpha}}(t)}\mathcal{Z}_{\boldsymbol{q}\bar{\alpha}}(t)\mathcal{Z}^*_{\boldsymbol{q}\bar{\alpha}}(t_D)}{\left[\mathcal{E}_{\boldsymbol{q}\bar{\alpha}}(t) - \omega_{\boldsymbol{q}\alpha_p}(t)\right]\left[\mathcal{E}_{\boldsymbol{q}\bar{\alpha}}(t_D) - \omega_{\boldsymbol{q}\alpha_{p'}}(t_D)\right]} \\ &= \oint_{\text{lower}} d\mathcal{E}_{\boldsymbol{q}\bar{\alpha}}(t_D)\rho^0_{\boldsymbol{q}\bar{\alpha}} \\ &\quad \times \frac{\tilde{z}^*_{\boldsymbol{q}\bar{\alpha}\alpha_p}(t)\tilde{z}_{\boldsymbol{q}\bar{\alpha}\alpha_{p'}}(t_D)e^{-i\Theta_{\boldsymbol{q}\bar{\alpha}}(t)}\mathcal{Z}_{\boldsymbol{q}\bar{\alpha}}(t)\mathcal{Z}^*_{\boldsymbol{q}\bar{\alpha}}(t_D)}{\left[\mathcal{E}_{\boldsymbol{q}\bar{\alpha}}(t) - \omega_{\boldsymbol{q}\alpha_p}(t)\right]\left[\mathcal{E}_{\boldsymbol{q}\bar{\alpha}}(t_D) - \omega_{\boldsymbol{q}\alpha_{p'}}(t_D)\right]}. \qquad \text{(E70)}\end{aligned}$$

Here, in the second equality, the summation over $\bar{\alpha}$ is replaced by an integral over $\mathcal{E}_{\boldsymbol{q}\bar{\alpha}}(t_D)$ in view of Eq. (D86), and a density of state, $\rho^0_{\boldsymbol{q}\bar{\alpha}}$, at time $t_D$ is represented as

$$\rho^0_{\boldsymbol{q}\bar{\alpha}} = \rho_{\boldsymbol{q}\bar{\alpha}}(t_D). \qquad \text{(E71)}$$

Moreover, this is rewritten as a contour integral with respect to a complex variable of $\mathcal{E}_{\boldsymbol{q}\bar{\alpha}}(t_D)$, where the contour is along a semicircle with an infinite radius in a lower-half plane including a real axis. Such a choice of the path is ensured by existence of a vanishing exponential function of $\exp\left[-i\Theta_{\boldsymbol{q}\bar{\alpha}}(t)\right]$ along the lower-half plane. This would be made sure by rewriting the adiabatic energy phase $\Theta_{\boldsymbol{q}\bar{\alpha}}(t)$ of Eqs. (D27) and (E4) as

$$\begin{aligned}\Theta_{\boldsymbol{q}\bar{\alpha}}(t) &\approx \mathcal{E}_{\boldsymbol{q}\bar{\alpha}}(t_D)(t - t_D) \\ &\quad + \int_{t_D}^{t}dt'\left[\mathcal{E}_{\boldsymbol{q}\bar{\alpha}_p}(t') - \mathcal{E}_{\boldsymbol{q}\bar{\alpha}_p}(t_D)\right] \\ &\quad - i\mathfrak{Z}_{\boldsymbol{q}\bar{\alpha}_p}(t,t_D), \qquad \text{(E72)}\end{aligned}$$

where $\mathfrak{Z}_{\boldsymbol{q}\bar{\alpha}}(t,t_D)$ is defined in Eq. (D19), and $\bar{\alpha}$ is approximately replaced by $\bar{\alpha}_p$ in the second and third terms of Eq. (E72). Therefore, the evaluation of Eq. (E70) results

in calculus of residues at the poles given by Eq. (E69); it is remarked that spurious poles emerging in a denominator of the integrand of Eq. (E70) are exactly canceled with a factor of $L^0_{\boldsymbol{q}\bar{\alpha}}(t)L^0_{\boldsymbol{q}\bar{\alpha}}(t_D)$ of $\mathcal{Z}_{\boldsymbol{q}\bar{\alpha}}(t)\mathcal{Z}^*_{\boldsymbol{q}\bar{\alpha}}(t_D)$, as seen in Eq. (E61). The resulting expression is shown as follows:

$$\begin{aligned}&\tilde{R}_{\boldsymbol{q}\alpha_p\alpha_{p'}}(t,t_D)\\&\approx \delta_{\alpha_p\alpha_{p'}}\exp\left\{-i\int_{t_D}^{t}\left[\mathcal{E}^{(r)}_{\boldsymbol{q}\alpha_p}(t'')-i\frac{\Gamma_{\boldsymbol{q}\alpha_p}(t'')}{2}\right]dt''\right\}\\&\times e^{-\mathfrak{Z}_{\boldsymbol{q}\bar{\alpha}_p}(t,t_D)}\frac{\pi\rho^0_{\boldsymbol{q}\bar{\alpha}_p}}{\bar{\Gamma}_{\boldsymbol{q}\alpha_p}(t,t_D)/2}\tilde{z}_{\boldsymbol{q}\bar{\alpha}_p\alpha_p}(t)\tilde{z}^\dagger_{\boldsymbol{q}\bar{\alpha}_p\alpha_p}(t_D),\end{aligned} \tag{E73}$$

where $\mathcal{E}^{(r)}_{\boldsymbol{q}\alpha_p}(t'')$ is substituted for $\mathcal{E}_{\boldsymbol{q}\bar{\alpha}_p}(t'')$. It is evident that this expression is just compatible to the identity relation given by

$$\tilde{R}_{\boldsymbol{q}\alpha_p\alpha_{p'}}(t_D,t_D)=\delta_{\alpha_p\alpha_{p'}} \tag{E74}$$

because of $\mathfrak{Z}_{\boldsymbol{q}\bar{\alpha}_p}(t_D,t_D)=1$, where this arises from an equal-time commutation relation of Eq. (D79). In fact, such compatibility is realized by virtue of neglecting additional terms emerging on the way of reduction of Eq. (E70), based on the approximations made in Eqs. (E56) and Eq. (E64).

The similar way of calculation to that of Eq. (E49) is applicable to reduction procedures of Eqs. (E50)-(E52). Thus, below, just the points of difference are clarified between the ways of calculations of the former equation and the latter three ones without describing details of derivations. As regards Eq. (E50), $\eta_{\boldsymbol{q}\bar{\alpha}'\bar{\alpha}}$ consists of two terms including $\delta_{\bar{\alpha}'\bar{\alpha}}$ and a Cauchy's principle value, as seen in Eq. (D89). For the reason to be mentioned right below, an expression of the form, $\sum_{\bar{\alpha}'}\tilde{R}_{\boldsymbol{q}\alpha_p\bar{\alpha}'}(t,t_D)C_{\bar{\alpha}'}$, is evaluated rather than Eq. (E50), where $C_{\bar{\alpha}'}$ represents an auxiliary regular-function of $\mathcal{E}_{\boldsymbol{q}\bar{\alpha}'}$. One part of this expression with $\delta_{\bar{\alpha}'\bar{\alpha}}$ is straightforward evaluated just in the similar manner as done for Eq. (E49). On the other hand, the other part of it includes the Cauchy's principle value of an integral over $\mathcal{E}_{\boldsymbol{q}\bar{\alpha}}$. In evaluating this contour integral, the path of integral is to be modified from that taken in Eq. (E49) so as to avoid a singular point of $\mathcal{E}_{\boldsymbol{q}\bar{\alpha}}=\mathcal{E}_{\boldsymbol{q}\bar{\alpha}'}$. The equation resulting from this integration becomes of the form of another integral over $\mathcal{E}_{\boldsymbol{q}\bar{\alpha}'}$. The reduction to such an integral is the reason why the auxiliary function $C_{\bar{\alpha}'}$ is introduced in advance. This integration can be readily implemented by means of calculus of residues. The expression thus obtained is as follows:

$$\begin{aligned}&\tilde{R}_{\boldsymbol{q}\alpha_p\bar{\alpha}'}(t,t_D)\\&\approx \delta_{\bar{\alpha}_p\bar{\alpha}'}\exp\left\{-i\int_{t_D}^{t}\left[\mathcal{E}^{(r)}_{\boldsymbol{q}\alpha_p}(t'')-i\frac{\Gamma_{\boldsymbol{q}\alpha_p}(t'')}{2}\right]dt''\right\}\\&\times e^{-\mathfrak{Z}_{\boldsymbol{q}\bar{\alpha}_p}(t,t_D)}\pi\rho^0_{\boldsymbol{q}\bar{\alpha}_p}\left[1-\frac{\pi\rho^0_{\boldsymbol{q}\bar{\alpha}_p}|\tilde{z}_{\boldsymbol{q}\bar{\alpha}_p\alpha_p}(t_D)|^2}{\bar{\Gamma}_{\boldsymbol{q}\alpha_p}(t,t_D)/2}\right]\\&\times(-i)\tilde{z}_{\boldsymbol{q}\bar{\alpha}_p\alpha_p}(t).\end{aligned} \tag{E75}$$

Similarly, Eq. (E51) becomes

$$\begin{aligned}&\tilde{R}_{\boldsymbol{q}\bar{\boldsymbol{\alpha}}'\alpha_p}(t,t_D)\\&\approx \delta_{\bar{\alpha}'\bar{\alpha}_p}\exp\left\{-i\int_{t_D}^{t}\left[\mathcal{E}^{(r)}_{\boldsymbol{q}\alpha_p}(t'')-i\frac{\Gamma_{\boldsymbol{q}\alpha_p}(t'')}{2}\right]dt''\right\}\\&\times e^{-\mathfrak{Z}_{\boldsymbol{q}\bar{\alpha}_p}(t,t_D)}\pi\rho^0_{\boldsymbol{q}\bar{\alpha}_p}\left[1-\frac{\pi\rho^0_{\boldsymbol{q}\bar{\alpha}_p}|\tilde{z}_{\boldsymbol{q}\bar{\alpha}_p\alpha_p}(t)|^2}{\bar{\Gamma}_{\boldsymbol{q}\alpha_p}(t,t_D)/2}\right]\\&\times(+i)\tilde{z}^*_{\boldsymbol{q}\bar{\alpha}_p\alpha_p}(t_D).\end{aligned} \tag{E76}$$

It is evident that this expression is just compatible to the identity relation given by

$$\tilde{R}_{\boldsymbol{q}\alpha_p\bar{\alpha}}(t_D,t_D)=0,\;\;\tilde{R}_{\boldsymbol{q}\bar{\alpha}\alpha_p}(t_D,t_D)=0, \tag{E77}$$

where these arise from equal-time commutation relations of Eq. (D80).

Finally, for evaluation of Eq. (E52), this is more involved than the others of Eqs. (E49)-(E51), since a dual integral of Cauchy's principle values is incorporated due to the presence of the first term in parentheses of Eq. (D89). For the same reason as the introduction of an auxiliary function to $\tilde{R}_{\boldsymbol{q}\bar{\alpha}\alpha_p}(t,t_D)$ in advance, it is convenient to introduce auxiliary regular-functions of $\mathcal{E}_{\boldsymbol{q}\bar{\alpha}'}$ and $\mathcal{E}_{\boldsymbol{q}\bar{\alpha}''}$, namely, $C_{\bar{\alpha}'}$ and $C'_{\bar{\alpha}''}$, respectively, and to calculate $\sum_{\bar{\alpha}'\bar{\alpha}''}C_{\bar{\alpha}'}\tilde{R}_{\boldsymbol{q}\bar{\alpha}'\bar{\alpha}''}(t,t_D)C'_{\bar{\alpha}''}$ in place of Eq. (E52). Owing to Poincaré's theorem of Eq. (D85), the product of Cauchy's principle values is allowed to be split into a sum of two Cauchy's principle values and delta-functions, which makes the resulting contour integrals feasible. Lengthy but elementary calculations bring Eq. (E52) to the following final expression as:

$$\begin{aligned}&\tilde{R}_{\boldsymbol{q}\bar{\boldsymbol{\alpha}}'\bar{\alpha}''}(t,t_D)\\&\approx \delta_{\bar{\alpha}'\bar{\alpha}''}\exp\left\{-i\int_{t_D}^{t}\mathcal{E}_{\boldsymbol{q}\bar{\alpha}'}(t'')dt''\right\}e^{-\mathfrak{Z}_{\boldsymbol{q}\bar{\alpha}'}(t,t_D)}\\&+\sum_p\delta_{\bar{\alpha}'\bar{\alpha}_p}\delta_{\bar{\alpha}''\bar{\alpha}_p}\\&\times\exp\left\{-i\int_{t_D}^{t}\left[\mathcal{E}^{(r)}_{\boldsymbol{q}\alpha_p}(t'')-i\frac{\Gamma_{\boldsymbol{q}\alpha_p}(t'')}{2}\right]dt''\right\}\\&\times e^{-\mathfrak{Z}_{\boldsymbol{q}\bar{\alpha}_p}(t,t_D)}(\pi\rho^0_{\boldsymbol{q}\bar{\alpha}_p})^2\Bigg[|\tilde{z}_{\boldsymbol{q}\bar{\alpha}_p\alpha_p}(t)|^2+|\tilde{z}_{\boldsymbol{q}\bar{\alpha}_p\alpha_p}(t_D)|^2\\&-\frac{2\pi\rho^0_{\boldsymbol{q}\bar{\alpha}_p}|\tilde{z}_{\boldsymbol{q}\bar{\alpha}_p\alpha_p}(t)|^2|\tilde{z}_{\boldsymbol{q}\bar{\alpha}_p\alpha_p}(t_D)|^2}{\bar{\Gamma}_{\boldsymbol{q}\alpha_p}(t,t_D)/2}\Bigg].\end{aligned} \tag{E78}$$

It is evident that this expression is just compatible to the identity relation given by

$$\tilde{R}_{\boldsymbol{q}\bar{\alpha}'\bar{\alpha}''}(t_D,t_D)=\delta_{\bar{\alpha}'\bar{\alpha}''} \tag{E79}$$

where this arises from equal-time commutation relation of Eq. (D81).

[5] W. Schäfer and M. Wegener, *Semiconductor Optics and Transport Phenomena* (Springer-Verlag, Berlin, 2002) Chaps. 2, 10, and 11.

## APPENDIX F: DERIVATION OF EQ. (114): SHORE'S SPECTRAL PROFILE

The spectral function $A_{\boldsymbol{q}}(t;\omega)$ of Eq. (113) is calculated in an analytic manner, to show that this is reduced to Shore's spectral profile given by Eq. (114) [6]. To begin with the expression of the total retarded susceptibility $\chi_{\boldsymbol{q}}^{(t)}(t'+\tau,t')$ of Eq. (79), given by

$$\begin{aligned}
&-i\chi_{\boldsymbol{q}}^{(t)}(t'+\tau,t')\\
&=\frac{4\pi}{V}\left\{\sum_{\bar{\alpha}=\bar{\alpha}_\pm} e^{i\mathcal{E}_{\boldsymbol{q}\bar{\alpha}}(t_D)\tau}\Xi_{\boldsymbol{q}\bar{\alpha}}^{(c)*}(t'+\tau,t')\right.\\
&+\sum_{p=1,2} e^{i[\mathcal{E}_{\boldsymbol{q}\alpha_p}^{(r)}(t_D)+i\Gamma_{\boldsymbol{q}\alpha_p}(t_D)/2]\tau}\\
&\times\left[\Xi_{\boldsymbol{q}\alpha_p}^{(r)*}(t'+\tau,t')+\Pi_{\boldsymbol{q}\alpha_p}^{(r)*}(t'+\tau,t')\right]\\
&\left.-\sum_{p=1,2} e^{-i[\mathcal{E}_{\boldsymbol{q}\alpha_p}^{(r)}(t_D)-i\Gamma_{\boldsymbol{q}\alpha_p}(t_D)/2]\tau}\Pi_{\boldsymbol{q}\alpha_p}^{(r)}(t'+\tau,t')\right\},
\end{aligned}\tag{F1}$$

in terms of Eqs. (89) and (103), it is seen that $A_{\boldsymbol{q}}(t;\omega)$ is composed of expressions of the form

$$Y_\alpha(t+\tau,t)=e^{i\mathcal{E}_\alpha(t_D)\tau}\Psi_\alpha(t+\tau,t),\tag{F2}$$

where $\mathcal{E}_\alpha(t_D)$ represents complex energy of the state $\alpha$. For instance, in the second term in the curl brackets of Eq. (F1), $\mathcal{E}_\alpha(t_D)$ corresponds to $\mathcal{E}_{\boldsymbol{q}\alpha_p}^{(r)}(t_D)+i\Gamma_{\boldsymbol{q}\alpha_p}(t_D)/2$ , and $\Psi_\alpha(t+\tau,t)$ corresponds to $[\Xi_{\boldsymbol{q}\alpha_p}^{(r)*}(t'+\tau,t')+\Pi_{\boldsymbol{q}\alpha_p}^{(r)*}(t'+\tau,t')]$. Hereafter, the argument of $t_D$ of $\mathcal{E}_\alpha(t_D)$ and so on is omitted just for the sake of typographical simplicity throughout this section, unless otherwise stated.

The Fourier-transform of Eq. (F2) is shown as

$$\begin{aligned}
\tilde{Y}_\alpha(t;\omega) &= \int_0^\infty d\tau\, e^{-i\omega\tau}Y_\alpha(t+\tau,t)\\
&= \int_0^\infty d\tau\, e^{-i(\omega-\mathcal{E}_\alpha)\tau}\Psi_\alpha(t+\tau,t).
\end{aligned}\tag{F3}$$

Applying repeated partial integrations to Eq. (F3) yields

$$\begin{aligned}
\tilde{Y}_\alpha(t;\omega) &= -\frac{1}{i\theta_\alpha}\sum_{n=0}^\infty\left[\frac{1}{i\theta_\alpha}\frac{d}{d\tau}\right]^n[-\Psi_\alpha(t+\tau,t)]\Big|_{\tau=0}\\
&\equiv -\frac{1}{i\theta_\alpha}\sum_{n=0}^\infty\left[\frac{1}{i\theta_\alpha}\frac{d}{d\tau}\right]^n[-\Psi_\alpha(t,t)]\\
&= -\frac{i}{\theta_\alpha+i\frac{d}{d\tau}}\Psi_\alpha(t,t)\\
&= \frac{d_\alpha(\omega)}{(\omega-\mathrm{Re}\mathcal{E}_\alpha)^2+(\mathrm{Im}\mathcal{E}_\alpha)^2},
\end{aligned}\tag{F4}$$

where the $n$th-order derivative of $\Psi_\alpha(t+\tau,t)$ at $\tau=0$, namely, $\Psi_\alpha^{(n)}(t,t)$, is denoted as $d^n\Psi_\alpha(t,t)/d\tau^n$, and $\theta_\alpha\equiv\omega-\mathcal{E}_\alpha$. In the last equality, $d_\alpha(\omega)$ is defined as

$$\begin{aligned}
d_\alpha(\omega) &= -\left[i(\omega-\mathrm{Re}\mathcal{E}_\alpha)-\left(\mathrm{Im}\mathcal{E}_\alpha-\frac{d}{d\tau}\right)\right]\\
&\quad\times\hat{D}_\alpha\left(\omega,\frac{d}{d\tau}\right)\Psi_\alpha(t,t),
\end{aligned}\tag{F5}$$

where an operator $\hat{D}_\alpha\left(\omega,\frac{d}{d\tau}\right)$ is defined as

$$\hat{D}_\alpha\left(\omega,\frac{d}{d\tau}\right)=\left[1-\frac{2\mathrm{Im}\mathcal{E}_\alpha\frac{d}{d\tau}-\frac{d^2}{d\tau^2}}{(\omega-\mathrm{Re}\mathcal{E}_\alpha)^2+(\mathrm{Im}\mathcal{E}_\alpha)^2}\right]^{-1}.\tag{F6}$$

Thus, real and imaginary parts of $d_\alpha(\omega)$ are given by

$$\begin{aligned}
&\mathrm{Re}d_\alpha(\omega)\\
&=(\omega-\mathrm{Re}\mathcal{E}_\alpha)\hat{D}_\alpha\left(\omega,\frac{d}{d\tau}\right)\mathrm{Im}\Psi_\alpha(t,t)\\
&+\left(\mathrm{Im}\mathcal{E}_\alpha-\frac{d}{d\tau}\right)\hat{D}_\alpha\left(\omega,\frac{d}{d\tau}\right)\mathrm{Re}\Psi_\alpha(t,t),
\end{aligned}\tag{F7}$$

and

$$\begin{aligned}
&\mathrm{Im}d_\alpha(\omega)\\
&=-(\omega-\mathrm{Re}\mathcal{E}_\alpha)\hat{D}_\alpha\left(\omega,\frac{d}{d\tau}\right)\mathrm{Re}\Psi_\alpha(t,t)\\
&+\left(\mathrm{Im}\mathcal{E}_\alpha-\frac{d}{d\tau}\right)\hat{D}_\alpha\left(\omega,\frac{d}{d\tau}\right)\mathrm{Im}\Psi_\alpha(t,t),
\end{aligned}\tag{F8}$$

respectively. Expanding $\hat{D}_\alpha$ with respect to $d/d\tau$, and retaining the resulting expressions up to terms including the first-order derivative of $\Psi'_\alpha(t,t)\equiv\Psi_\alpha^{(1)}(t,t)$, $\mathrm{Re}d_\alpha(\omega)$ becomes

$$\begin{aligned}
&\mathrm{Re}d_\alpha(\omega)\\
&\approx(\omega-\mathrm{Re}\mathcal{E}_\alpha)\frac{2\mathrm{Im}\mathcal{E}_\alpha\mathrm{Im}\Psi'_\alpha(t,t)}{(\omega-\mathrm{Re}\mathcal{E}_\alpha)^2+(\mathrm{Im}\mathcal{E}_\alpha)^2}\\
&+(\mathrm{Im}\mathcal{E}_\alpha)\mathrm{Re}\Psi_\alpha(t,t)\\
&-\left[1-\frac{2(\mathrm{Im}\mathcal{E}_\alpha)^2}{(\omega-\mathrm{Re}\mathcal{E}_\alpha)^2+(\mathrm{Im}\mathcal{E}_\alpha)^2}\right]\mathrm{Re}\Psi'_\alpha(t,t),
\end{aligned}\tag{F9}$$

while $\mathrm{Im}d_\alpha(\omega)$ becomes

$$\begin{aligned}
&\mathrm{Im}d_\alpha(\omega)\\
&\approx-(\omega-\mathrm{Re}\mathcal{E}_\alpha)\\
&\times\left[\mathrm{Re}\Psi_\alpha(t,t)+\frac{2\mathrm{Im}\mathcal{E}_\alpha\mathrm{Re}\Psi'_\alpha(t,t)}{(\omega-\mathrm{Re}\mathcal{E}_\alpha)^2+(\mathrm{Im}\mathcal{E}_\alpha)^2}\right]\\
&-\left[1-\frac{2(\mathrm{Im}\mathcal{E}_\alpha)^2}{(\omega-\mathrm{Re}\mathcal{E}_\alpha)^2+(\mathrm{Im}\mathcal{E}_\alpha)^2}\right]\mathrm{Im}\Psi'_\alpha(t,t),
\end{aligned}\tag{F10}$$

where the fact of $\Psi_\alpha(t,t)$ being real is taken into account [see Eqs. (92), (93), and (104)].

First, the Fourier-transform of the first term of Eq. (F1), $\tilde{Y}^{(c)}_{\boldsymbol{q}\bar{\alpha}}(t;\omega)$, is evaluated, which is given by consulting Eqs. (F3), (F9), and (F10) as

$$\begin{aligned}\tilde{Y}^{(c)}_{\boldsymbol{q}\bar{\alpha}}(t;\omega) &= \int_0^\infty d\tau e^{-i(\omega-\mathcal{E}_{\boldsymbol{q}\bar{\alpha}}-\imath\eta)\tau}\Xi^{(c)*}_{\boldsymbol{q}\bar{\alpha}}(t+\tau,t)\\ &\approx \frac{[\eta-i(\omega-\mathcal{E}_{\boldsymbol{q}\bar{\alpha}})]\mathrm{Re}\Xi^{(c)*}_{\boldsymbol{q}\bar{\alpha}}(t,t)}{(\omega-\mathcal{E}_{\boldsymbol{q}\bar{\alpha}})^2+\eta^2}\\ &= \left[\pi\delta(\omega-\mathcal{E}_{\boldsymbol{q}\bar{\alpha}})-i\mathbb{P}\frac{1}{\omega-\mathcal{E}_{\boldsymbol{q}\bar{\alpha}}}\right]\mathrm{Re}\Xi^{(c)*}_{\boldsymbol{q}\bar{\alpha}}(t,t),\end{aligned} \tag{F11}$$

with $\eta = +0$. Further, in the second equality, it is supposed that the continuum energy of $\mathcal{E}_{\boldsymbol{q}\bar{\alpha}}(t)$ varies so slowly in time $t$ that $\mathcal{E}_{\boldsymbol{q}\bar{\alpha}}(t) \approx \mathcal{E}_{\boldsymbol{q}\bar{\alpha}}$, and thus, $\Xi^{(c)*}_{\boldsymbol{q}\bar{\alpha}}(t+\tau,t) \approx \Xi^{(c)*}_{\boldsymbol{q}\bar{\alpha}}(t,t)$: it is remarked that $\Xi^{(c)*}_{\boldsymbol{q}\bar{\alpha}}(t,t)$ is real. Hence, taking a summation of Eq. (F11) over $\bar{\alpha}$ yields the following expression:

$$\begin{aligned}\sum_{\bar{\alpha}}\tilde{Y}^{(c)}_{\boldsymbol{q}\bar{\alpha}}(t;\omega) &= \pi\rho^0_{\boldsymbol{q}\bar{\alpha}_\omega}\mathrm{Re}\Xi^{(c)*}_{\boldsymbol{q}\bar{\alpha}_\omega}(t,t)\\ &\quad -i\sum_{\bar{\alpha}}\mathbb{P}\frac{\mathrm{Re}\Xi^{(c)*}_{\boldsymbol{q}\bar{\alpha}}(t,t)}{\omega-\mathcal{E}_{\boldsymbol{q}\bar{\alpha}}},\end{aligned} \tag{F12}$$

where in the first term of the right-hand side, $\bar{\alpha}_\omega$ is defined as $\mathcal{E}_{\boldsymbol{q}\bar{\alpha}_\omega} = \omega$.

Next, the Fourier-transform of the second term of Eq. (F1), $\tilde{Y}^{(r)}_{\boldsymbol{q}\alpha_p}(t;\omega)$, is evaluated. Here, letting $\Psi^{(r)}_{\boldsymbol{q}\bar{\alpha}_p}(t+\tau,t)$ be defined as

$$\Psi^{(r)}_{\boldsymbol{q}\bar{\alpha}_p}(t+\tau,t) = \Xi^{(r)*}_{\boldsymbol{q}\bar{\alpha}_p}(t+\tau,t)+\Pi^{(r)*}_{\boldsymbol{q}\bar{\alpha}_p}(t+\tau,t), \tag{F13}$$

one obtains the following expression:

$$\begin{aligned}\tilde{Y}^{(r)}_{\boldsymbol{q}\alpha_p}(t;\omega) &= \int_0^\infty d\tau e^{-i(\omega-\mathcal{E}^{(r)}_{\boldsymbol{q}\alpha_p}-i\Gamma_{\boldsymbol{q}\alpha_p}/2)\tau}\Psi^{(r)}_{\boldsymbol{q}\bar{\alpha}_p}(t+\tau,t)\\ &= \frac{d^{(r)}_{\boldsymbol{q}\alpha_p}(t;\omega)}{L_{\boldsymbol{q}\alpha_p}(\omega)},\end{aligned} \tag{F14}$$

by consulting Eq. (F4). Here, real and imaginary parts of $d^{(r)}_{\boldsymbol{q}\alpha_p}(t;\omega)$ correspond to Eqs. (F9) and (F10), respectively, with substituting $\mathcal{E}^{(r)}_{\boldsymbol{q}\alpha_p}$, $\Gamma_{\boldsymbol{q}\alpha_p}/2$, $\Psi^{(r)}_{\boldsymbol{q}\bar{\alpha}_p}(t,t)$, and $\Psi^{(r)\prime}_{\boldsymbol{q}\bar{\alpha}_p}(t,t)$ for $\mathrm{Re}\mathcal{E}_\alpha$, $\mathrm{Im}\mathcal{E}_\alpha$, $\Psi_\alpha(t,t)$, and $\Psi'_\alpha(t,t)$, respectively. Further, $L_{\boldsymbol{q}\alpha_p}(\omega)$ is defined as

$$L_{\boldsymbol{q}\alpha_p}(\omega) = (\omega-\mathcal{E}^{(r)}_{\boldsymbol{q}\alpha_p})^2+(\Gamma_{\boldsymbol{q}\alpha_p}/2)^2. \tag{F15}$$

As regards the Fourier-transform of the third term of Eq. (F1), in fact, an explicit expression of it is unnecessary for the subsequent discussion, and thus, this is just denoted as $\Delta\tilde{Y}^{(r)}_{\boldsymbol{q}\alpha_p}(t;\omega)$.

Lumping the respective expressions obtained above for the Fourier-transform of Eq. (F1), Eq. (111) is provided as

$$\begin{aligned}&\epsilon_\infty[\tilde{\epsilon}^{(t)}(t;\omega)]^{-1}\\ &= 1+ic_{\boldsymbol{q}}(t;\omega)\\ &+iV^{(C)}_{\boldsymbol{q}}\sum_{p=1,2}\left[\frac{d^{(r)}_{\boldsymbol{q}\alpha_p}(t;\omega)}{L_{\boldsymbol{q}\alpha_p}(\omega)}+\Delta\tilde{Y}^{(r)}_{\boldsymbol{q}\alpha_p}(t;\omega)\right],\end{aligned} \tag{F16}$$

where $c_{\boldsymbol{q}}(t;\omega)$ is defined as Eq. (F12) multiplied by $V^{(C)}_{\boldsymbol{q}}$, that is,

$$c_{\boldsymbol{q}}(t;\omega) = V^{(C)}_{\boldsymbol{q}}\sum_{\bar{\alpha}}\tilde{Y}^{(c)}_{\boldsymbol{q}\bar{\alpha}}(t;\omega). \tag{F17}$$

Since one is primarily concerned with the behavior of $A_{\boldsymbol{q}}(t;\omega)$ in the vicinity of phonon energy, namely, $\omega = \mathcal{E}^{(r)}_{\boldsymbol{q}\alpha_2}$, Eq. (F16) is readily approximated as

$$\epsilon_\infty[\tilde{\epsilon}^{(t)}(t;\omega)]^{-1} \approx 1+ic_{\boldsymbol{q}}(t;\omega)+\frac{i\bar{d}^{(r)}_{\boldsymbol{q}\alpha_2}(t;\omega)}{L_{\boldsymbol{q}\alpha_2}(\omega)}, \tag{F18}$$

where

$$\bar{d}^{(r)}_{\boldsymbol{q}\alpha_2}(t;\omega) = V^{(C)}_{\boldsymbol{q}}d^{(r)}_{\boldsymbol{q}\alpha_2}(t;\omega). \tag{F19}$$

Thus, $\tilde{\epsilon}^{(t)}(t;\omega)$ is given by

$$\frac{\tilde{\epsilon}^{(t)}(t;\omega)}{\epsilon_\infty} \approx 1-ic_{\boldsymbol{q}}(t;\omega)-\frac{i\bar{d}^{(r)}_{\boldsymbol{q}\alpha_2}(t;\omega)}{L_{\boldsymbol{q}\alpha_2}(\omega)+i\bar{d}^{(r)}_{\boldsymbol{q}\alpha_2}(t;\omega)}, \tag{F20}$$

which brings $A_{\boldsymbol{q}}(t;\omega)$ to the following form:

$$\begin{aligned}&-A_{\boldsymbol{q}}(t;\omega)/\epsilon_\infty\\ &= \mathrm{Re}c_{\boldsymbol{q}}(t;\omega)\\ &+\frac{L_{\boldsymbol{q}\alpha_2}(\omega)\mathrm{Re}\bar{d}^{(r)}_{\boldsymbol{q}\alpha_2}(t;\omega)}{[L_{\boldsymbol{q}\alpha_2}(\omega)-\mathrm{Im}\bar{d}^{(r)}_{\boldsymbol{q}\alpha_2}(t;\omega)]^2+[\mathrm{Re}\bar{d}^{(r)}_{\boldsymbol{q}\alpha_2}(t;\omega)]^2}.\end{aligned} \tag{F21}$$

Letting the denominator of the second term in the right-hand side of the above equation be $L_{\boldsymbol{q}\alpha_2}(\omega)D_{\boldsymbol{q}\alpha_2}(t;\omega)$, $D_{\boldsymbol{q}\alpha_2}(t;\omega)$ is reduced to

$$\begin{aligned}D_{\boldsymbol{q}\alpha_2}(t;\omega) &= L_{\boldsymbol{q}\alpha_2}(\omega)-2\mathrm{Im}\bar{d}^{(r)}_{\boldsymbol{q}\alpha_2}(t;\omega)+\frac{|\bar{d}^{(r)}_{\boldsymbol{q}\alpha_2}(t;\omega)|^2}{L_{\boldsymbol{q}\alpha_2}(\omega)}\\ &= \left[\omega-\bar{\mathcal{E}}^{(r)}_{\boldsymbol{q}\alpha_2}(t;\omega)\right]^2+\left[\bar{\Gamma}_{\boldsymbol{q}\alpha_2}(t;\omega)/2\right]^2.\end{aligned} \tag{F22}$$

Here, it is seen that the resonant energy $\bar{\mathcal{E}}^{(r)}_{\boldsymbol{q}\alpha_2}$ and the associated energy width $\bar{\Gamma}_{\boldsymbol{q}\alpha_2}$ are $\omega$-dependent as well as $t$-dependent, and these are given by

$$\bar{\mathcal{E}}^{(r)}_{\boldsymbol{q}\alpha_2}(t;\omega) = \mathcal{E}^{(r)}_{\boldsymbol{q}\alpha_2}+\mathrm{Im}a_{\boldsymbol{q}\alpha_2}(t;\omega), \tag{F23}$$

and

$$\left[\bar{\Gamma}_{\boldsymbol{q}\alpha_2}(t;\omega)/2\right]^2 = (\Gamma_{\boldsymbol{q}\alpha_2}/2)^2 + [\mathrm{Re}a_{\boldsymbol{q}\alpha_2}(t;\omega)]^2 - 2\mathrm{Im}b_{\boldsymbol{q}\alpha_2}(t;\omega) + \Delta_{\boldsymbol{q}\alpha_2}(t;\omega), \tag{F24}$$

where both of $a_{\boldsymbol{q}\alpha_2}(t;\omega)$ and $b_{\boldsymbol{q}\alpha_2}(t;\omega)$ are defined by representing Eq. (F19) as

$$\bar{d}^{(r)}_{\boldsymbol{q}\alpha_2}(t;\omega) = a_{\boldsymbol{q}\alpha_2}(t;\omega)(\omega - \mathcal{E}^{(r)}_{\boldsymbol{q}\alpha_2}) + b_{\boldsymbol{q}\alpha_2}(t;\omega) \tag{F25}$$

according to Eqs. (F9) and (F10), and

$$\begin{aligned}&\Delta_{\boldsymbol{q}\alpha_2}(t;\omega)\\&= \{2\left[(\mathrm{Re}a_{\boldsymbol{q}\alpha_2})(\mathrm{Re}b_{\boldsymbol{q}\alpha_2}) + (\mathrm{Im}a_{\boldsymbol{q}\alpha_2})(\mathrm{Im}b_{\boldsymbol{q}\alpha_2})\right]\\&\quad\times(\omega - \mathcal{E}^{(r)}_{\boldsymbol{q}\alpha_2}) + |b_{\boldsymbol{q}\alpha_2}|^2 - |a_{\boldsymbol{q}\alpha_2}|^2(\Gamma_{\boldsymbol{q}\alpha_2}/2)^2\Big\}\\&\quad\times\left[L_{\boldsymbol{q}\alpha_2}(\omega)\right]^{-1}.\end{aligned} \tag{F26}$$

with the arguments, $t$ and $\omega$, of both of $a_{\boldsymbol{q}\alpha_2}(t;\omega)$ and $b_{\boldsymbol{q}\alpha_2}(t;\omega)$ being omitted just for the sake of typographical simplicity. Hereafter, it is assumed that both of $a_{\boldsymbol{q}\alpha_2}(t;\omega)$ and $b_{\boldsymbol{q}\alpha_2}(t;\omega)$ are well-approximated as the lowest-order expressions of $a_{\boldsymbol{q}\alpha_2}(t;\mathcal{E}^{(r)}_{\boldsymbol{q}\alpha_2})$ and $b_{\boldsymbol{q}\alpha_2}(t;\mathcal{E}^{(r)}_{\boldsymbol{q}\alpha_2})$, respectively, and thus, $\Delta_{\boldsymbol{q}\alpha_2}(t;\omega)$ is also approximated as $\Delta_{\boldsymbol{q}\alpha_2}(t;\mathcal{E}^{(r)}_{\boldsymbol{q}\alpha_2})$.

Therefore, in view of Eq. (F22), Eq. (F21) is cast into

$$\begin{aligned}&\bar{A}_{\boldsymbol{q}}(t;\omega) \equiv -A_{\boldsymbol{q}}(t;\omega)\\&\approx \mathcal{C}_{\boldsymbol{q}}(t) + \frac{\mathcal{A}_{\boldsymbol{q}\alpha_2}(t)\left[\omega - \bar{\mathcal{E}}^{(r)}_{\boldsymbol{q}\alpha_2}(t)\right] + \mathcal{B}_{\boldsymbol{q}\alpha_2}(t)\bar{\Gamma}_{\boldsymbol{q}\alpha_2}(t)/2}{\left[\omega - \bar{\mathcal{E}}^{(r)}_{\boldsymbol{q}\alpha_2}(t)\right]^2 + \left[\bar{\Gamma}_{\boldsymbol{q}\alpha_2}(t)/2\right]^2}\end{aligned} \tag{F27}$$

in the vicinity of $\omega = \bar{\mathcal{E}}^{(r)}_{\boldsymbol{q}\alpha_2}(t)$, where it is defined that

$$\bar{\mathcal{E}}^{(r)}_{\boldsymbol{q}\alpha_2}(t) \equiv \bar{\mathcal{E}}^{(r)}_{\boldsymbol{q}\alpha_2}(t;\mathcal{E}^{(r)}_{\boldsymbol{q}\alpha_2}),\ \bar{\Gamma}_{\boldsymbol{q}\alpha_2}(t) \equiv \bar{\Gamma}_{\boldsymbol{q}\alpha_2}(t;\mathcal{E}^{(r)}_{\boldsymbol{q}\alpha_2}). \tag{F28}$$

Further, $\mathcal{A}_{\boldsymbol{q}\alpha_2}(t)$, $\mathcal{B}_{\boldsymbol{q}\alpha_2}(t)$, and $\mathcal{C}_{\boldsymbol{q}}(t)$ are given by

$$\mathcal{A}_{\boldsymbol{q}\alpha_2}(t) = \epsilon_\infty \mathrm{Re}a_{\boldsymbol{q}\alpha_2}(t;\mathcal{E}^{(r)}_{\boldsymbol{q}\alpha_2}), \tag{F29}$$

$$\begin{aligned}\mathcal{B}_{\boldsymbol{q}\alpha_2}(t) &= \epsilon_\infty\Big[\mathrm{Re}b_{\boldsymbol{q}\alpha_2}(t;\mathcal{E}^{(r)}_{\boldsymbol{q}\alpha_2}) + \mathrm{Re}a_{\boldsymbol{q}\alpha_2}(t;\mathcal{E}^{(r)}_{\boldsymbol{q}\alpha_2})\\&\quad\times\mathrm{Im}a_{\boldsymbol{q}\alpha_2}(t;\mathcal{E}^{(r)}_{\boldsymbol{q}\alpha_2})\Big]/\left[\bar{\Gamma}_{\boldsymbol{q}\alpha_2}(t)/2\right],\end{aligned} \tag{F30}$$

and

$$\begin{aligned}\mathcal{C}_{\boldsymbol{q}}(t) &= \epsilon_\infty \mathrm{Re}c_{\boldsymbol{q}}(t;\mathcal{E}^{(r)}_{\boldsymbol{q}\alpha_2})\\&= \epsilon_\infty \pi \rho^0_{\boldsymbol{q}\bar{\alpha}_\omega} X^{(c)}_{\boldsymbol{q}\bar{\alpha}_\omega\bar{\alpha}_\omega}(t,t) V^{(C)}_{\boldsymbol{q}},\end{aligned} \tag{F31}$$

respectively. Moreover, explicit expressions of both of $a_{\boldsymbol{q}\alpha_2}(t;\mathcal{E}^{(r)}_{\boldsymbol{q}\alpha_2})$ and $b_{\boldsymbol{q}\alpha_2}(t;\mathcal{E}^{(r)}_{\boldsymbol{q}\alpha_2})$ are provided as

$$\mathrm{Re}a_{\boldsymbol{q}\alpha_2}(t;\mathcal{E}^{(r)}_{\boldsymbol{q}\alpha_2}) = \frac{2\mathrm{Im}\Psi^{(r)\prime}_{\boldsymbol{q}\bar{\alpha}_2}(t,t)}{\bar{\Gamma}_{\boldsymbol{q}\alpha_2}(t)/2} V^{(C)}_{\boldsymbol{q}}, \tag{F32}$$

$$\begin{aligned}&\mathrm{Im}a_{\boldsymbol{q}\alpha_2}(t;\mathcal{E}^{(r)}_{\boldsymbol{q}\alpha_2})\\&= -\left[\mathrm{Re}\Psi^{(r)}_{\boldsymbol{q}\bar{\alpha}_2}(t,t) + \frac{2\mathrm{Re}\Psi^{(r)\prime}_{\boldsymbol{q}\bar{\alpha}_2}(t,t)}{\bar{\Gamma}_{\boldsymbol{q}\alpha_2}(t)/2}\right] V^{(C)}_{\boldsymbol{q}},\end{aligned} \tag{F33}$$

$$\begin{aligned}&\mathrm{Re}b_{\boldsymbol{q}\alpha_2}(t;\mathcal{E}^{(r)}_{\boldsymbol{q}\alpha_2})\\&= \left[\mathrm{Re}\Psi^{(r)}_{\boldsymbol{q}\bar{\alpha}_2}(t,t)\bar{\Gamma}_{\boldsymbol{q}\alpha_2}(t)/2 + \mathrm{Re}\Psi^{(r)\prime}_{\boldsymbol{q}\bar{\alpha}_2}(t,t)\right] V^{(C)}_{\boldsymbol{q}},\end{aligned} \tag{F34}$$

and

$$\mathrm{Im}b_{\boldsymbol{q}\alpha_2}(t;\mathcal{E}^{(r)}_{\boldsymbol{q}\alpha_2}) = \mathrm{Im}\Psi^{(r)\prime}_{\boldsymbol{q}\bar{\alpha}_2}(t,t) V^{(C)}_{\boldsymbol{q}}. \tag{F35}$$

If $\bar{A}_{\boldsymbol{q}}(t;\omega)$ of Eq. (F27) is positive in the vicinity of $\omega = \bar{\mathcal{E}}^{(r)}_{\boldsymbol{q}\alpha_2}(t)$, this implies transient induced photoemission spectra, namely, transient negative absorption spectra, at time $t$. It is noticed that $\bar{A}_{\boldsymbol{q}}(t;\omega)$ shows Shore's spectral profile, in which asymmetric spectral profile due to $\mathcal{A}_{\boldsymbol{q}\alpha_2}(t)$ is superimposed with continuum background governed by $\mathcal{C}_{\boldsymbol{q}}(t)$: here the three parameters of $\mathcal{A}_{\boldsymbol{q}\alpha_2}(t)$, $\mathcal{B}_{\boldsymbol{q}\alpha_2}(t)$, and $\mathcal{C}_{\boldsymbol{q}}(t)$ are considered as Shore's spectral parameters. $\bar{A}_{\boldsymbol{q}}(t;\omega)$ seems to be a key observable to understand manifestation of transient Fano resonance that would be accompanied by coherent-phonon generation. The origin of the asymmetry can be traced back to the presence of Im $\Psi^{(r)\prime}_{\boldsymbol{q}\bar{\alpha}_2}(t,t)$ determined by Eq. (F13). The associated Fano's $q$-parameter is determined in terms of Shore's parameters as

$$q_{\boldsymbol{q}\alpha_2}(t) = r_{\boldsymbol{q}\alpha_2}(t) + \sigma_{\boldsymbol{q}\alpha_2}(t)\sqrt{[r_{\boldsymbol{q}\alpha_2}(t)]^2 + 1}, \tag{F36}$$

where

$$r_{\boldsymbol{q}\alpha_2}(t) = \frac{\mathcal{B}_{\boldsymbol{q}\alpha_2}(t)}{\mathcal{A}_{\boldsymbol{q}\alpha_2}(t)},\quad \sigma_{\boldsymbol{q}\alpha_2}(t) = \frac{\mathcal{A}_{\boldsymbol{q}\alpha_2}(t)}{|\mathcal{A}_{\boldsymbol{q}\alpha_2}(t)|}. \tag{F37}$$

[6] B. W. Shore, Rev. Mod. Phys. **39**, 439 (1967).

## APPENDIX G: DERIVATION OF EQ. (126): PHONON DISPLACEMENT FUNCTION $Q_{\boldsymbol{q}}(t)$

An expectation value of $[c^\dagger_{\boldsymbol{q}}(t) + c_{\boldsymbol{q}}(t)]/2$ with respect to the ground state, namely,

$$Q_{\boldsymbol{q}}(t) = \frac{1}{2}\langle c_{\boldsymbol{q}}(t) + c^\dagger_{-\boldsymbol{q}}(t)\rangle. \tag{G1}$$

is examined. This is regarded as a classical phonon displacement function, if this expectation value is taken with respect to a coherent state of phonon. In addition, this is also considered as transition probability of Raman scattering process [7]. The phonon operator $c_{\boldsymbol{q}}$ is extracted from a PQ operator by means of the projection similar to Eq. (86), that is,

$$c_{\boldsymbol{q}}(t) = \sum_{\beta} V_{\boldsymbol{q}\alpha_2\beta}(t) F_{\boldsymbol{q}\beta}(t). \tag{G2}$$

Employing Eqs. (D37), (D43), and (E9), this becomes

$$\begin{aligned} c_{\boldsymbol{q}}(t) &= \sum_{\beta\gamma} V_{\boldsymbol{q}\alpha_2\beta}(t) e^{-i\Theta_{\boldsymbol{q}\beta}(t)} V^\dagger_{\boldsymbol{q}\beta\gamma}(t_D) \\ &\quad \times \left[\mathcal{T}^\dagger_{\boldsymbol{q}}(t) F^0_{\boldsymbol{q}}(t_D)\right]_\gamma \\ &= \sum_{\gamma} R_{\boldsymbol{q}\alpha_2\gamma}(t) \left[\mathcal{T}^\dagger_{\boldsymbol{q}}(t) F^0_{\boldsymbol{q}}(t_D)\right]_\gamma. \end{aligned} \tag{G3}$$

Further, the explicit expression of Eq. (E14) is applied to this with $\alpha$ replaced by $\alpha_2$ and $\mathcal{A}^{(r)\dagger}_{\boldsymbol{q}\alpha_2\alpha}(t) = 0$, which yields

$$\begin{aligned} \langle c_{\boldsymbol{q}}(t)\rangle &= \sum_{p=1,2} \mathcal{A}^{(r)\dagger}_{\boldsymbol{q}\alpha_2\alpha_p}(t) \exp\left[-i\int_{t_D}^{t} \mathcal{E}^{(r)}_{\boldsymbol{q}\alpha_p}(t'')dt''\right] \\ &\quad \times \exp\left[-\int_{t_D}^{t} \frac{\Gamma_{\boldsymbol{q}\alpha_p}(t'')}{2} dt''\right] e^{-\mathfrak{Z}_{\boldsymbol{q}\bar{\alpha}_p}(t,t_D)} \\ &\quad \times \mathcal{D}_{\boldsymbol{q}\alpha_p}(t,t_D) \left[\mathcal{A}^{(r)}_{\boldsymbol{q}}(t_D) \mathcal{T}^\dagger_{\boldsymbol{q}}(t) \langle F^0_{\boldsymbol{q}}(t_D)\rangle\right]_{\alpha_p} \\ &= \sum_{p=1,2} P_{\boldsymbol{q}\alpha_p}(t,t_D) \exp\left[-i\int_0^t \mathcal{E}^{(r)}_{\boldsymbol{q}\alpha_p}(t'')dt''\right] \\ &\quad \times \exp\left[-\int_{t_D}^{t} \frac{\Gamma_{\boldsymbol{q}\alpha_p}(t'')}{2} dt''\right]. \end{aligned} \tag{G4}$$

Here, in the second equality, $P_{\boldsymbol{q}\alpha_p}(t,t_D)$ is defined as

$$\begin{aligned} P_{\boldsymbol{q}\alpha_p}(t,t_D) &= \mathcal{A}^{(r)\dagger}_{\boldsymbol{q}\alpha_2\alpha_p}(t) \mathcal{D}_{\boldsymbol{q}\alpha_p}(t,t_D) \mathcal{O}^*_{\boldsymbol{q}\alpha_p}(t,t_D) \\ &\quad \times e^{-\mathfrak{Z}_{\boldsymbol{q}\bar{\alpha}_p}(t,t_D)}, \end{aligned} \tag{G5}$$

where $\mathcal{O}^*_{\boldsymbol{q}\alpha_p}(t,t_D)$ is defined as

$$\begin{aligned} \mathcal{O}^*_{\boldsymbol{q}\alpha_p}(t,t_D) &= \left[\mathcal{A}^{(r)}_{\boldsymbol{q}}(t_D) \mathcal{T}^\dagger_{\boldsymbol{q}}(t) \langle F^0_{\boldsymbol{q}}(t_D)\rangle\right]_{\alpha_p} \\ &\quad \times \exp\left[-i\int_{t_D}^{0} \mathcal{E}^{(r)}_{\boldsymbol{q}\alpha_p}(t'')dt''\right]. \end{aligned} \tag{G6}$$

Therefore, $Q_{\boldsymbol{q}}(t)$ ends up with

$$\begin{aligned} Q_{\boldsymbol{q}}(t) &= X_{\boldsymbol{q}}(t,t_D) \exp\left[-\int_{t_D}^{t} dt' \, \frac{\Gamma_{\boldsymbol{q}\alpha_2}(t')}{2}\right] \\ &\quad \times \sin\left[\omega^{(LO)}_{\boldsymbol{q}} t + \theta_{\boldsymbol{q}}(t)\right] + \Delta Q_{\boldsymbol{q}}(t), \end{aligned} \tag{G7}$$

where the approximation that $\langle c^\dagger_{-\boldsymbol{q}}(t)\rangle = \langle c^\dagger_{\boldsymbol{q}}(t)\rangle = \langle c_{\boldsymbol{q}}(t)\rangle^\dagger$ is taken into account; this is verified in a similar manner to that mentioned right below Eq. (F1). Further, $X_{\boldsymbol{q}}(t,t_D)$ and $\theta_{\boldsymbol{q}}(t)$ are defined as

$$X_{\boldsymbol{q}}(t,t_D) = |P_{\boldsymbol{q}\alpha_2}(t,t_D)|, \tag{G8}$$

and

$$\theta_{\boldsymbol{q}}(t) = \frac{\pi}{2} + \Delta\alpha'_{\boldsymbol{q}}(t) - \xi_{\boldsymbol{q}}(t) + \upsilon_{\boldsymbol{q}\bar{\alpha}_2}(t,t_D) + \theta^0_{\boldsymbol{q}}(t), \tag{G9}$$

respectively. Here, $\upsilon_{\boldsymbol{q}\bar{\alpha}_2}(t,t_D)$ is defined in Eq. (132), $\Delta\alpha'_{\boldsymbol{q}}(t)$ is an integrated adiabatic energy-phase at $t$, given by

$$\Delta\alpha'_{\boldsymbol{q}}(t) = \int_0^t \left[\mathcal{E}^{(r)}_{\boldsymbol{q}\alpha_2}(t'') - \omega^{(LO)}_{\boldsymbol{q}}\right] dt'', \tag{G10}$$

$\xi_{\boldsymbol{q}}(t)$ is a phase associated with FR dynamics, given by

$$\mathcal{D}_{\boldsymbol{q}\alpha_2}(t,t_D) = |\mathcal{D}_{\boldsymbol{q}\alpha_2}(t,t_D)| e^{i\xi_{\boldsymbol{q}}(t)}, \tag{G11}$$

and an additional phase $\theta^0_{\boldsymbol{q}}(t)$ is defined as an argument of $\mathcal{O}^*_{\boldsymbol{q}\alpha_p}(t,t_D)$, that is,

$$\mathcal{O}_{\boldsymbol{q}\alpha_p}(t,t_D) = |\mathcal{O}_{\boldsymbol{q}\alpha_p}(t,t_D)| e^{i\theta^0_{\boldsymbol{q}}(t)}. \tag{G12}$$

In addition, in Eq. (G7), $\Delta Q_{\boldsymbol{q}}(t)$ arises from a plasmonic contribution, defined as

$$\begin{aligned} \Delta Q_{\boldsymbol{q}}(t) &= P_{\boldsymbol{q}\alpha_1}(t,t_D) \exp\left[-i\int_0^t \mathcal{E}^{(r)}_{\boldsymbol{q}\alpha_1}(t'')dt''\right] \\ &\quad \times \exp\left[-\int_{t_D}^{t} \frac{\Gamma_{\boldsymbol{q}\alpha_1}(t'')}{2} dt''\right]. \end{aligned} \tag{G13}$$

[7] D. Lee, J. Inoue, and M. Hase, Phys. Rev. Lett. **97**, 157405 (2006).

## APPENDIX H: PROPERTIES OF DIMENSIONLESS FUNCTION $\mathcal{D}_{\boldsymbol{q}\alpha_p}(t, t_D)$

Traces of dimensionless function $\mathcal{D}_{\boldsymbol{q}\alpha_2}(t, t_D)$ given by Eq. (94) for Si and GaAs are shown in Figs. H-1 and H-2, respectively; this function is pertinent to an LO-phonon mode. It is noted that this is one of the key functions to understand the spectral profiles of $\bar{A}_{\boldsymbol{q}}(t_p;\omega)$ and $S_{\boldsymbol{q}}(\omega)$ [see Eqs. (93), (104), and (128)]. This function is a constituent marking $R_{\boldsymbol{q}\gamma\gamma'}(t, t_D)$, as shown in Eq. (E14). The function $\mathcal{D}_{\boldsymbol{q}\alpha_2}(t, t_D)$ is considered relevant to the time-evolution of PQ state $\alpha_2$ from $t_D$ to $t$, since it is evident from Eq. (E9) that $R_{\boldsymbol{q}\gamma\gamma'}(t, t_D)$ is attached a meaning of time-evolution of PQ from state $\gamma'$ at $t_D$ to state $\gamma$ at $t$. With the increase in $t$ from $t_D$ to $t_L$, overall $\mathcal{D}_{\boldsymbol{q}\alpha_2}(t, t_D)$ decreases with change from unity to the asymptotic constant-value given by Eq. (133). The traces of $\mathrm{Re}\mathcal{D}_{\boldsymbol{q}\alpha_2}(t, t_D)$ and $\mathrm{Im}\mathcal{D}_{\boldsymbol{q}\alpha_2}(t, t_D)$ as a function of time $t$ are shown in panel (a) and (b) of both figures, respectively. The traces shown by red solid lines are adopted for actual calculations in place of the traces shown by blue solid lines, since numerical inaccuracy caused approximately in the region $t > 80$ fs makes the calculations more unstable as seen from ripples observed in the latter traces. Here, the traces shown by the red and blue solid lines are calculated with and without a manipulative procedure of multiplying the original function $\mathcal{D}_{\boldsymbol{q}\alpha_2}(t, t_D)$ by an exponentially damping function in the region $t > 80$ fs, followed by a forced extrapolation to an asymptote $\mathcal{D}_{\boldsymbol{q}\alpha_2}(t_L, t_D)$ given by Eq. (133), respectively. The degree of damping in this procedure has little effects on physical quantities. In reality, the fact is made sure that there is little difference between $\bar{A}_{\boldsymbol{q}}(t_p;\omega)$'s obtained by employing heavily exponentially-damping function as given in Figs. H-1 and H-2 and those obtained by employing a couple of more moderately exponentially-damping functions.

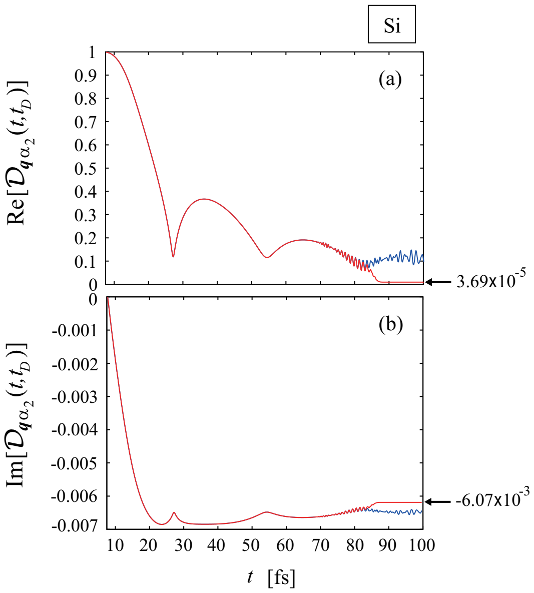


FIG. H-1: (Color Online) Traces of $\mathcal{D}_{\boldsymbol{q}\alpha_2}(t, t_D)$ of Si as a function of time $t$ (in the unit of fs). (a) $\mathrm{Re}\mathcal{D}_{\boldsymbol{q}\alpha_2}(t, t_D)$, (b) $\mathrm{Im}\mathcal{D}_{\boldsymbol{q}\alpha_2}(t, t_D)$. The red and blue solid lines represent traces with and without a manipulative procedure of multiplying the original function by an exponentially damping function in the region $t > 80$, followed by a forced extrapolation to an asymptote $\mathcal{D}_{\boldsymbol{q}\alpha_2}(t_L, t_D)$ given by Eq. (133), respectively. Further, numerical values of $\mathrm{Re}\mathcal{D}_{\boldsymbol{q}\alpha_2}(t_L, t_D)$ and $\mathrm{Im}\mathcal{D}_{\boldsymbol{q}\alpha_2}(t_L, t_D)$ are indicated by arrows in (a) and (b), respectively. The ripples observed in the region $t > 80$ are just due to numerical instability. It is noted that $\mathcal{D}_{\boldsymbol{q}\alpha_2}(t, t_D)$ is a dimensionless function.

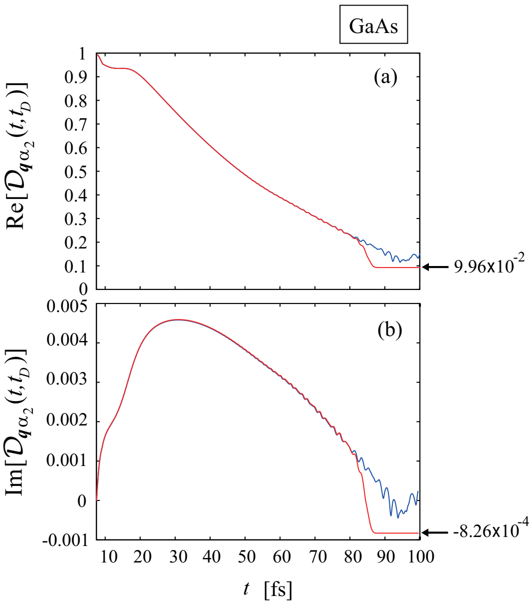


FIG. H-2: (Color Online) The same as Fig. H-1 but for GaAs.

Although the above-mentioned overall behavior is common to both cases of Si and GaAs, there is sharp contrast between the two in the patterns of alteration of phase factor $\xi_{\boldsymbol{q}}(t)$ defined in Eq. (G11). To be specific, as $t$ increases, $\xi_{\boldsymbol{q}}(t)$ changes from 0 to approximately $-\pi/2$ in Si , while it remains almost zero in GaAs; the trace of $\xi_{\boldsymbol{q}}(t)$ as a function of $t$ for Si is shown in Fig. H-3, where the meanings of the red and blue solid lines correspond to those in Fig. H-1. The difference between these is attributed to the effective coupling constant given by Eq. (52) along with Eqs. (50) and (51). In Si, $M_{\boldsymbol{q}\bar{\alpha}_2} = M^D_{\boldsymbol{q}\bar{\alpha}_2}$, and thus, the effective coupling constant is real. On the other hand, in GaAs, $M_{\boldsymbol{q}\bar{\alpha}_2} \approx M^F_{\boldsymbol{q}\bar{\alpha}_2}$, and thus, this is almost pure-imaginary. It is remarked that $\mathrm{Im}\mathcal{D}_{\boldsymbol{q}\alpha_2}(t, t_D)$ of Fig. H-2(b) just arises from the contribution from $M^D_{\boldsymbol{q}\bar{\alpha}_2}$; thus, the contribution of the optical-phonon deformation potential interaction to $\mathcal{D}_{\boldsymbol{q}\alpha_2}(t, t_D)$ is considered roughly one hundred times smaller than that of the Fröhlich interaction. The difference of $\mathcal{D}_{\boldsymbol{q}\alpha_2}(t, t_D)$ in argument between in Si and

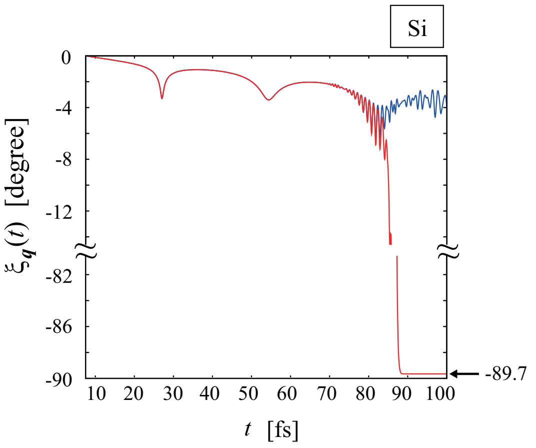


FIG. H-3: (Color Online) A trace of $\xi_{\boldsymbol{q}}(t)$ of Si as a function of time $t$ (in the unit of fs). The traces shown by red and blue solid lines are obtained from the corresponding curves shown in Fig. H-1. A numerical value of asymptotic phase $\xi_{\boldsymbol{q}}(t_L)$ is indicated by an arrow.

GaAs plays a decisive role of discriminating spectral profiles of $\bar{A}_{\boldsymbol{q}}(\omega)$ in both cases. Moreover, it is pointed out that for large $t$, $|\mathcal{D}_{\boldsymbol{q}\alpha_2}(t,t_D)|$ of GaAs is roughly sixteen times greater than that of Si, due presumably to the difference between $M^D_{\boldsymbol{q}\bar{\alpha}_2}$ and $M^F_{\boldsymbol{q}\bar{\alpha}_2}$. In fact, the difference of $\mathcal{D}_{\boldsymbol{q}\alpha_2}(t,t_D)$ in magnitude also plays a significant role of making a sharp contrast of spectral profiles of $S_{\boldsymbol{q}}(\omega)$ between the two. For such reasons, special attention should be paid to $\mathcal{D}_{\boldsymbol{q}\alpha_2}(t,t_D)$ in the discussion made in both of Secs. IIIA and IIIC.

In the meantime, a couple of dips are discerned in $\mathcal{D}_{\boldsymbol{q}\alpha_2}(t,t_D)$ of Si at $t \approx 25$ and 55 fs, as shown in Fig. H-1, in contrast with that of GaAs shown in Fig. H-2. It is considered that such dips are due to non-adiabatic couplings of the state $\bar{\alpha}_2$ with adjacent adiabatic states around these $t$'s. To confirm this statement, one examines alteration of an adiabatic energy value $\mathcal{E}^{(r)}_{\boldsymbol{q}\alpha_2}(t)$ of Si with respect to $t$ shown in Fig. E-1, where an approximate definition of it is given in Eq. (90). The first time of $t \approx 25$ fs coincides with the time at which $\mathcal{E}^{(r)}_{\boldsymbol{q}\alpha_2}(t)$ varies with a kink in an irregular manner; though slight irregularity in $\mathcal{E}^{(r)}_{\boldsymbol{q}\alpha_2}(t)$ at $t \approx 55$ fs is not discerned in the scale employed in this figure. Such irregularity would be attributed to a crossing between adiabatic states, resulting in a conspicuous non-adiabatic interaction. In fact, the number of crossings and the temporal locations of them would depend on the laser parameters listed in Table A-2 – such as pulse area $A_L$ – as well as the number of sites $N_s$ given in Table A-1. For instance, with the increase of $A_L$, more crossings would manifest themselves in a more complicated manner. This tendency would apply for both cases of Si and GaAs, though no dip structure is discerned in Fig. H-2 within the present choice of the parameters. In actual calculations, in order to mimic a situation with larger $A_L$ and $N_s$, some parameters requisite for a non-adiabatic coupling are dealt with just as given parameters, as shown in more detail in Secs. IIIA and IIIC.

As regards another dimensionless function $\mathcal{D}_{\boldsymbol{q}\alpha_1}(t,t_D)$ pertinent to a plasmon mode, this is almost real and independent of whether an effective coupling constant is real or pure-imaginary, though not shown here. Actually, it is readily shown that for $t \gg t_D$, the expression of $\mathcal{D}_{\boldsymbol{q}\alpha_1}(t,t_D)$ is reduced to a real function given by

$$\mathcal{D}_{\boldsymbol{q}\alpha_1}(t,t_D) \overset{t\gg t_D}{\approx} \frac{2M_{\boldsymbol{q}\bar{\alpha}_1}(t)}{M_{\boldsymbol{q}\bar{\alpha}_1}(t_D)}, \tag{H1}$$

where with the increase in $t$ from $t_D$, overall $\mathcal{D}_{\boldsymbol{q}\alpha_1}(t,t_D)$ decreases from unity to an asymptote proportional to $M_{\boldsymbol{q}\bar{\alpha}_1}(t)$; $|M_{\boldsymbol{q}\bar{\alpha}_1}(t)| \ll |M_{\boldsymbol{q}\bar{\alpha}_1}(t_D)|$.
